# Supplementary material for: ACL-SPC: Adaptive Closed-Loop system for Self-Supervised Point Cloud Completion
Source: arXiv:2303.01979 source file (2023-03-28)
Supplement: Supplementary file 5 [file views4.tex]

\begin{figure*}[ht]
	\captionsetup[subfloat]{labelformat=empty}
	%\begin{center}
		\newcommand{\rowArg}{0.6cm}
		\newcommand{\fullSize}{2.cm}
		\newcommand{\patchSize}{2.6cm}
		% 			\begin{adjustbox}{width=\linewidth, center=\linewidth}
		\setlength{\tabcolsep}{0.05cm}		
            \begin{tabular}[b]{c c c}
			\multicolumn{2}{c}{\multirow{2}{*}[\rowArg]{
					\subfloat[GT]
					% 			{\includegraphics[width = \fullSize, height = \fullSize]
					{\includegraphics[page=23, height=\fullSize]
					{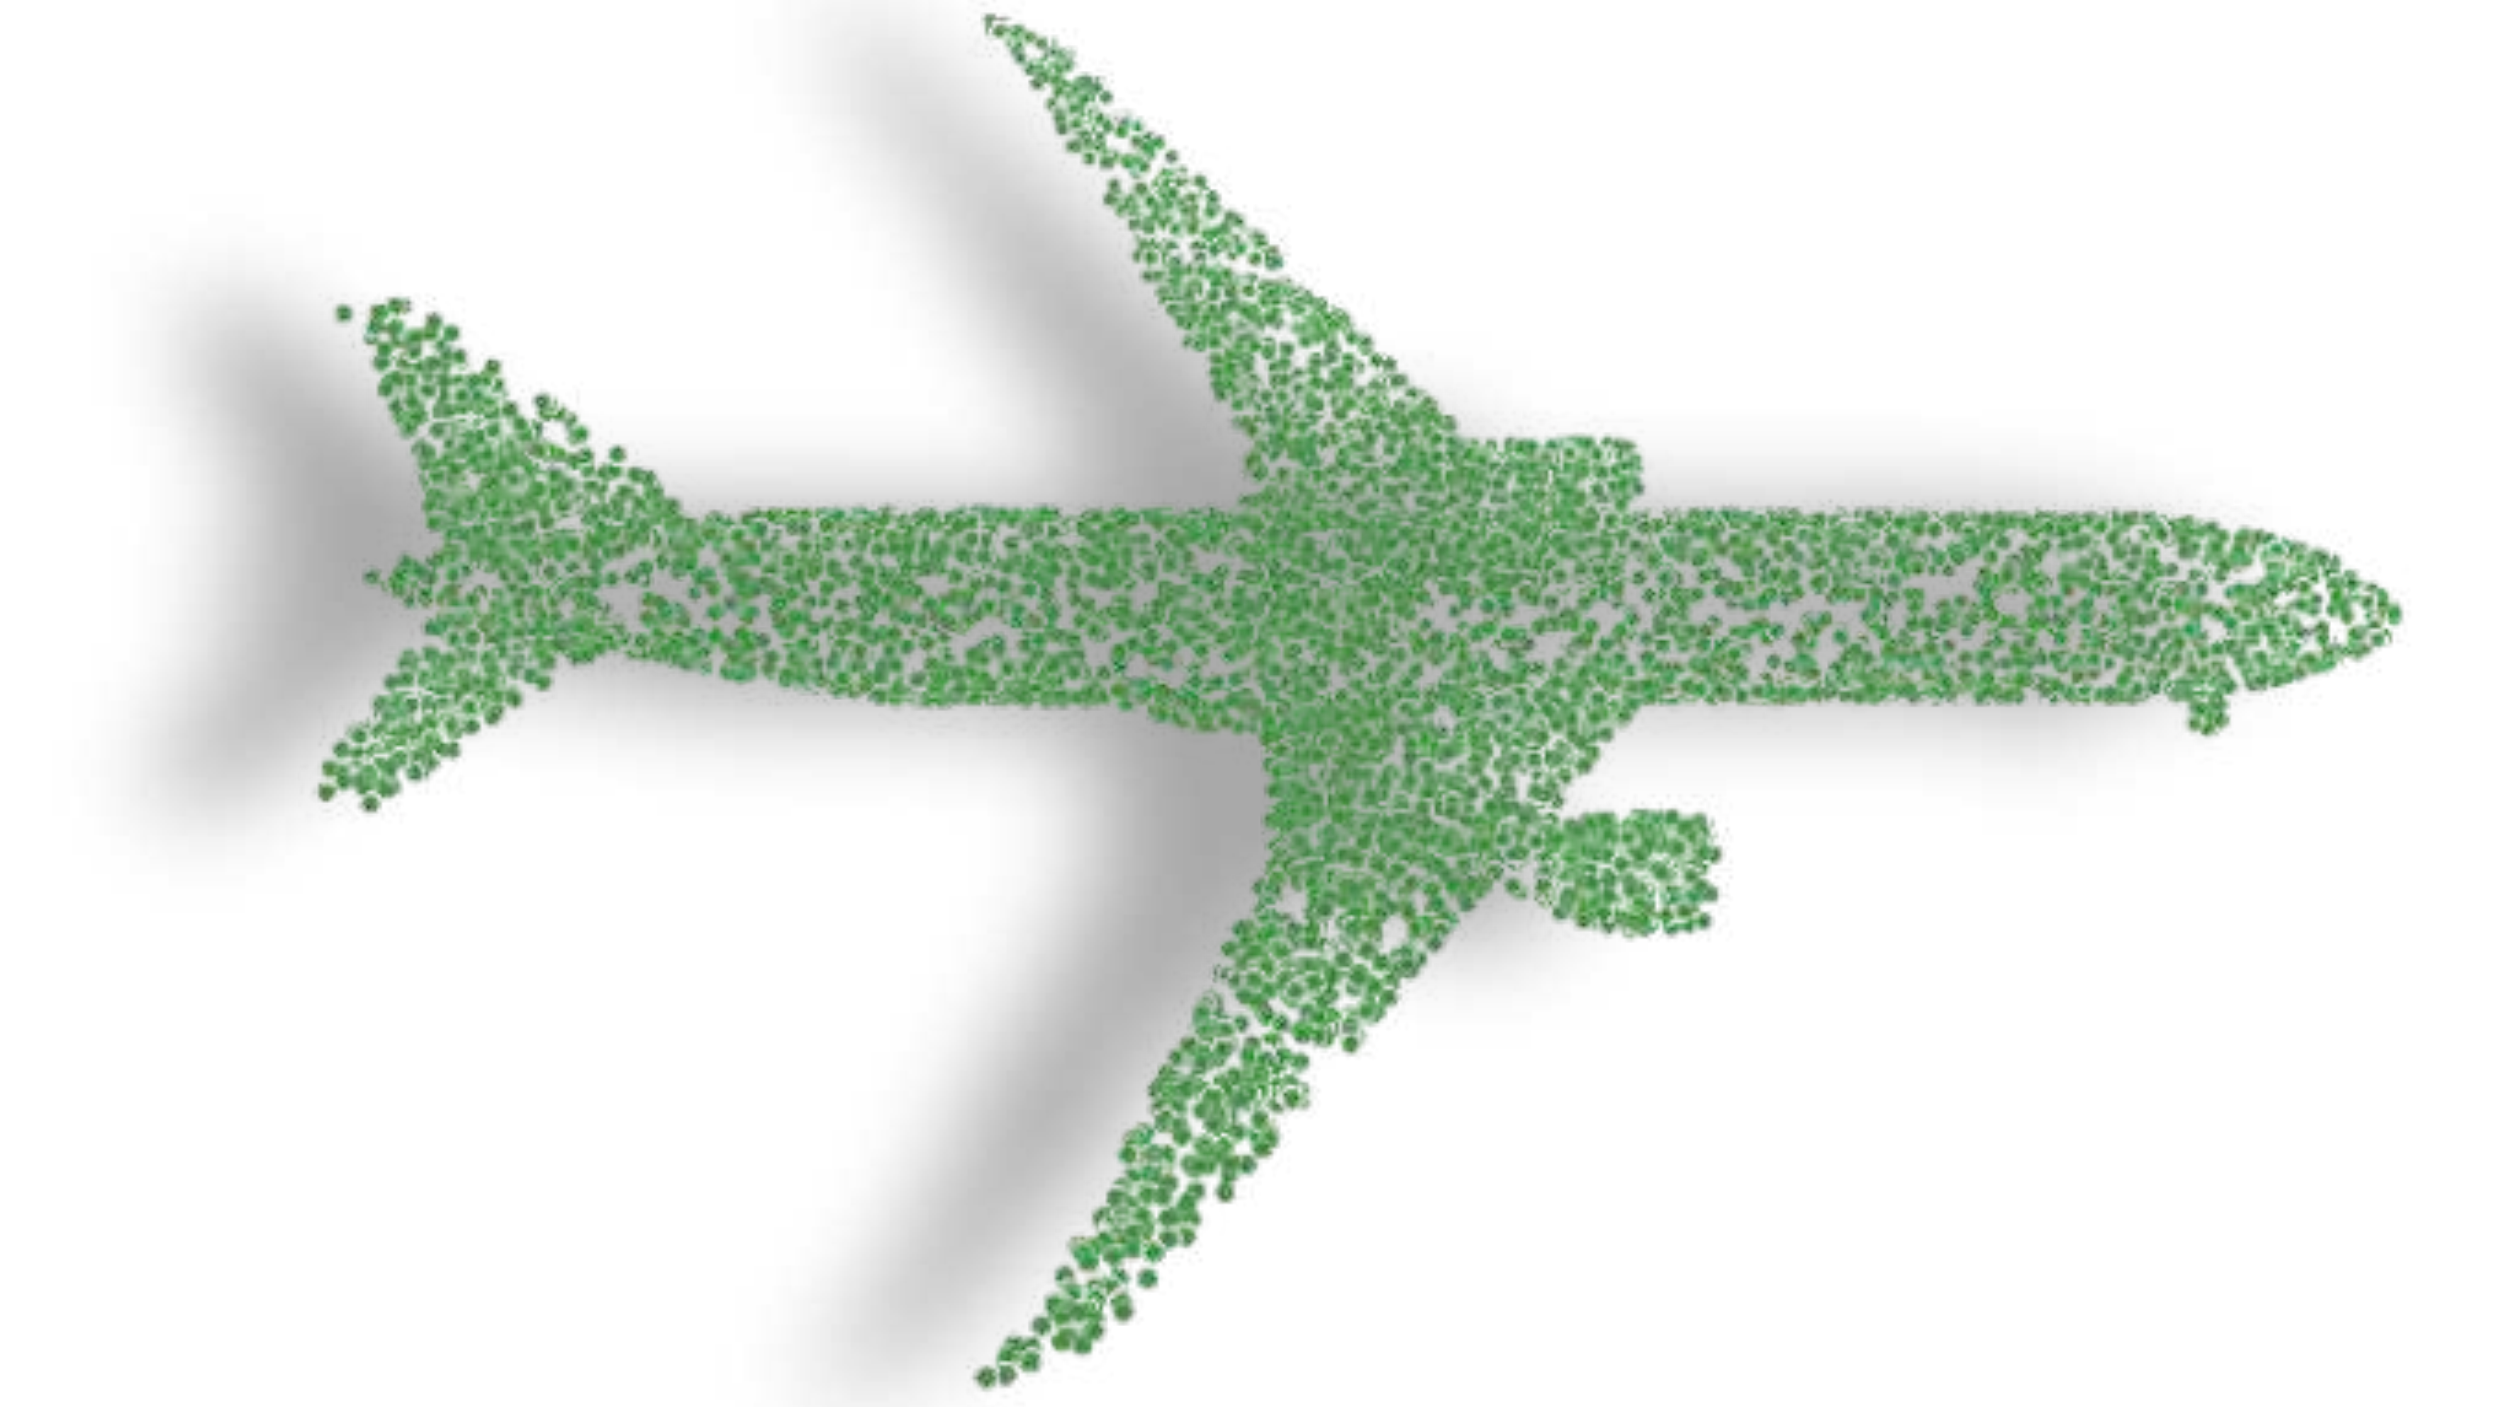}}}} &
			\subfloat[\centering \tiny Partial View 1 ]{
				\includegraphics[page=24, width = \patchSize]
				{figures/supp_view.pdf}} 
			\subfloat[\centering \tiny Partial View 2  ]{
				\includegraphics[page=25, width = \patchSize]
				{figures/supp_view.pdf}} 
			\subfloat[\centering \tiny Partial View 3  ]{
				\includegraphics[page=26, width = \patchSize]
				{figures/supp_view.pdf}} 
			\subfloat[\centering \tiny Partial View 4  ]{
				\includegraphics[page=27, width = \patchSize]
				{figures/supp_view.pdf}}
			\subfloat[\centering \tiny Partial View 5  ]{
				\includegraphics[page=28, width = \patchSize]
				{figures/supp_view.pdf}} \\  & &

			\subfloat[\centering  \tiny Complete 1  ]{
				\includegraphics[page=29, width = \patchSize]
				{figures/supp_view.pdf}}
			\subfloat[\centering \tiny Complete 2 ]{
				\includegraphics[page=30, width = \patchSize]
				{figures/supp_view.pdf}}
			\subfloat[\centering \tiny Complete 3 ]{
				\includegraphics[page=31, width = \patchSize]
				{figures/supp_view.pdf}}
			\subfloat[\centering \tiny Complete 4]{
				\includegraphics[page=32, width = \patchSize]
				{figures/supp_view.pdf}}
			\subfloat[\centering \tiny Complete 5]{
				\includegraphics[page=33, width = \patchSize]
				{figures/supp_view.pdf}}\\
	    \end{tabular}
    \caption{\textbf{The qualitative effect of viewpoint.} 
    }
    \label{fig:supp_views}	    

\vspace{4mm}     
\end{figure*}
