# Supplementary material for: ACL-SPC: Adaptive Closed-Loop system for Self-Supervised Point Cloud Completion
Source: arXiv:2303.01979 source file (2023-03-28)

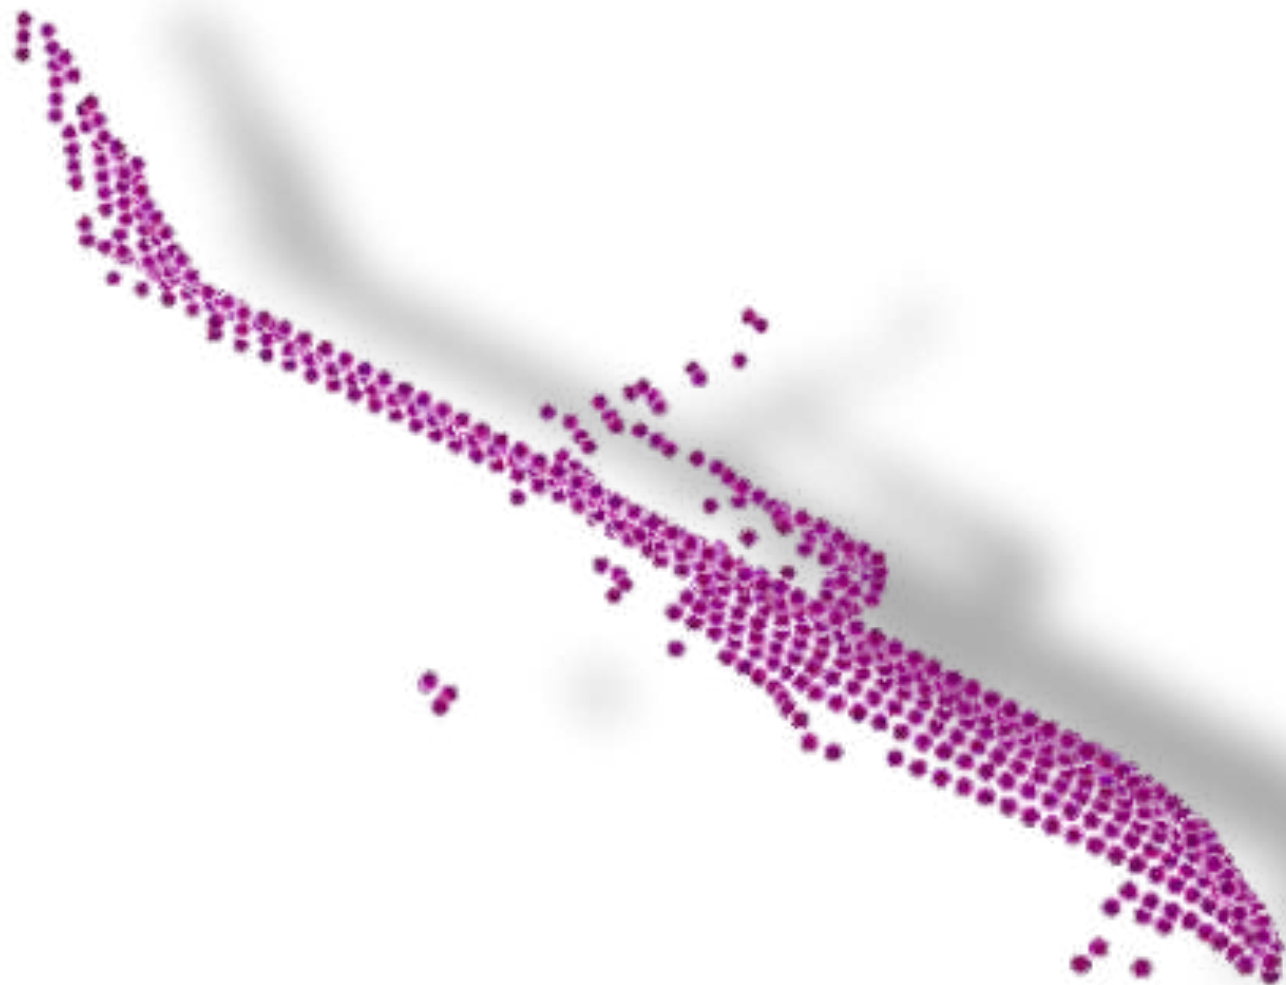

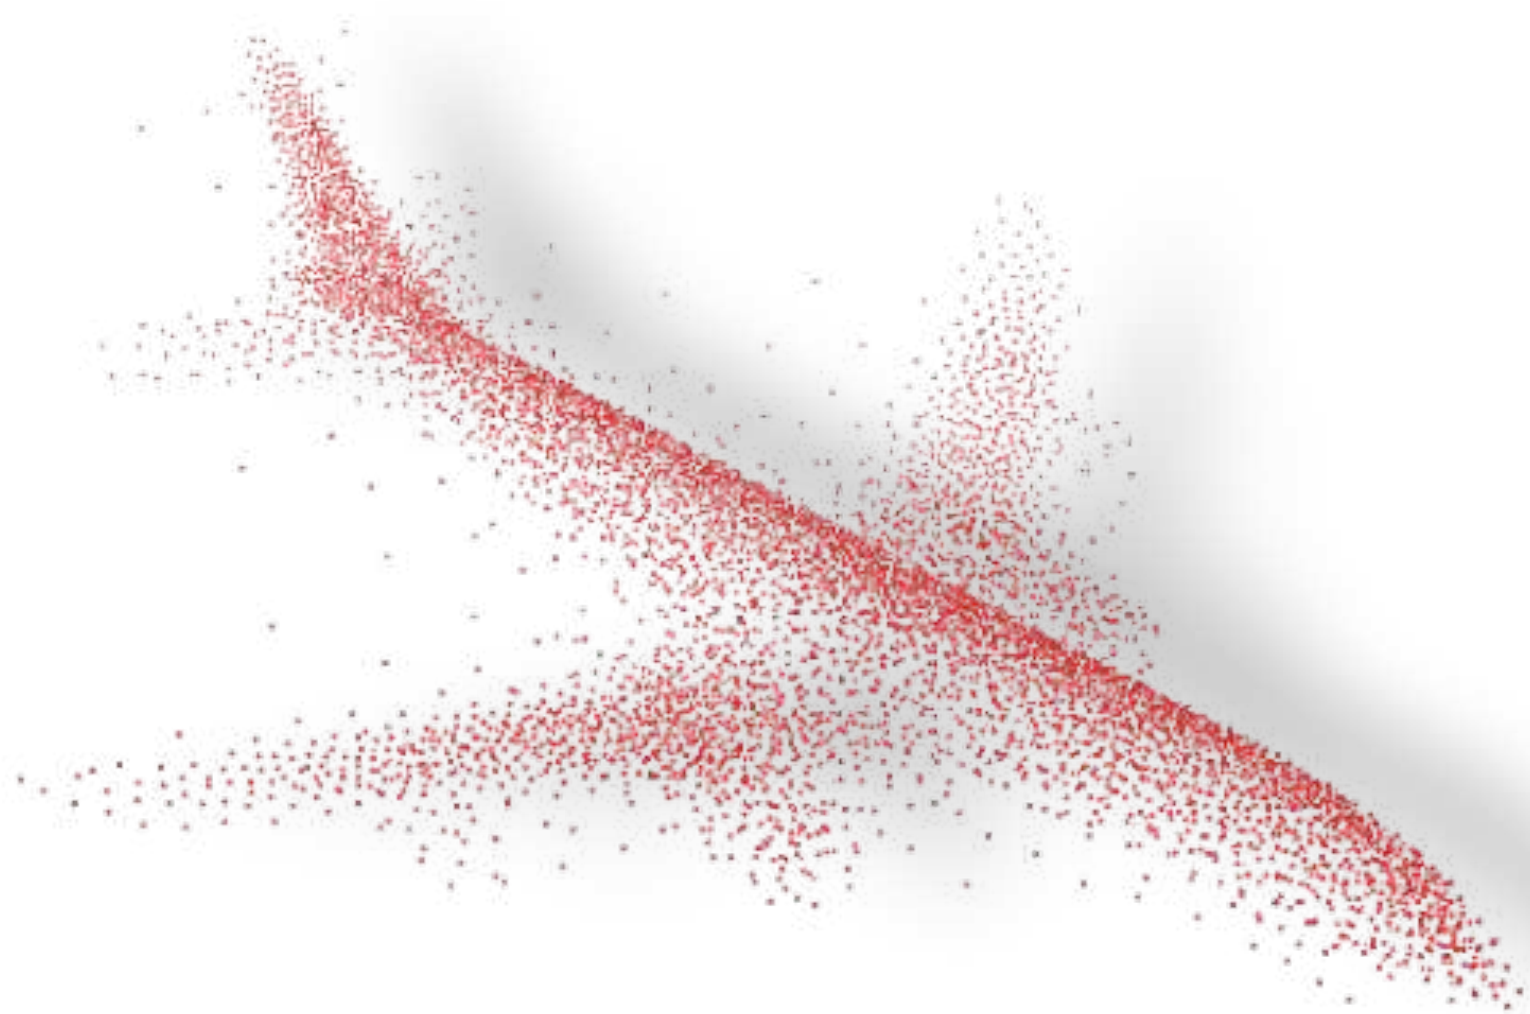

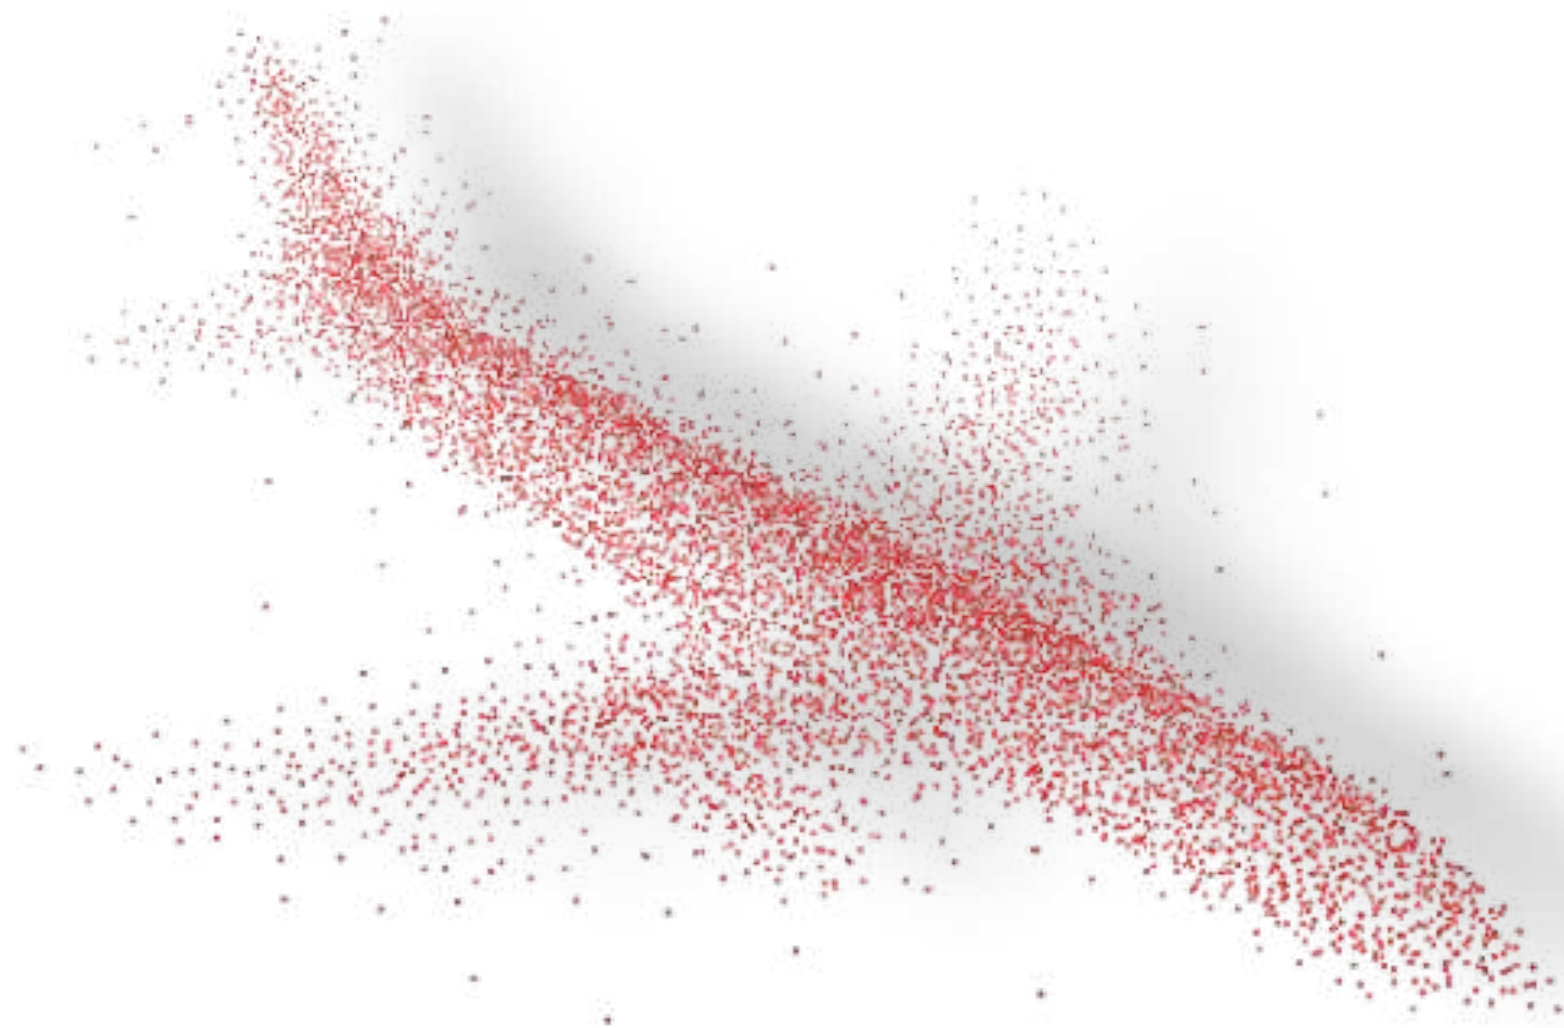

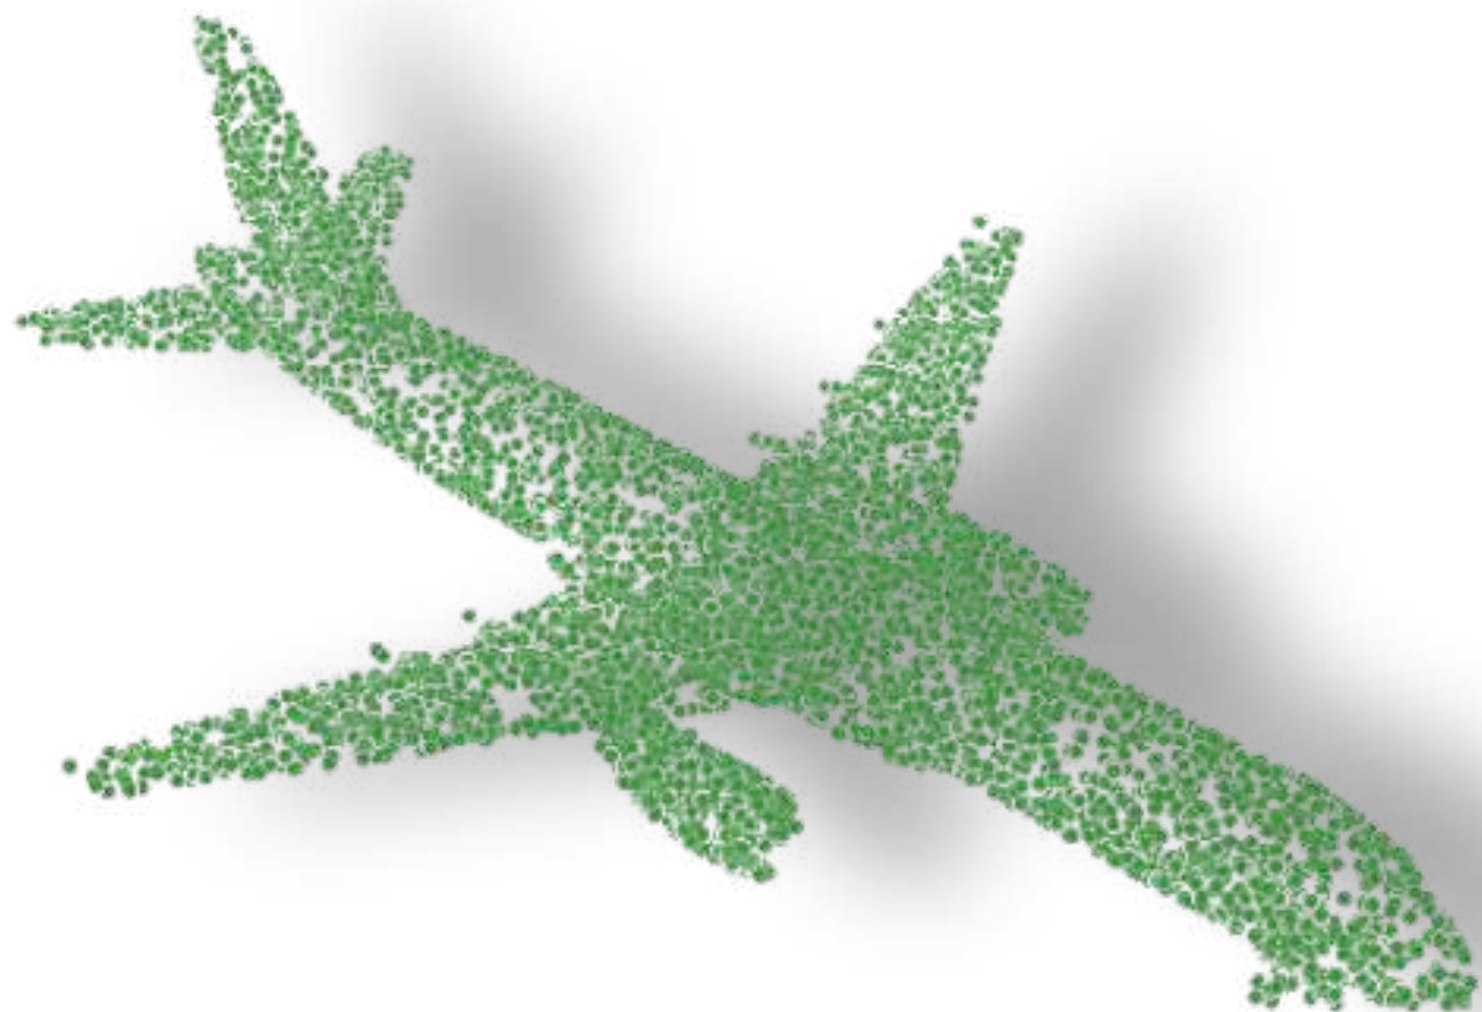

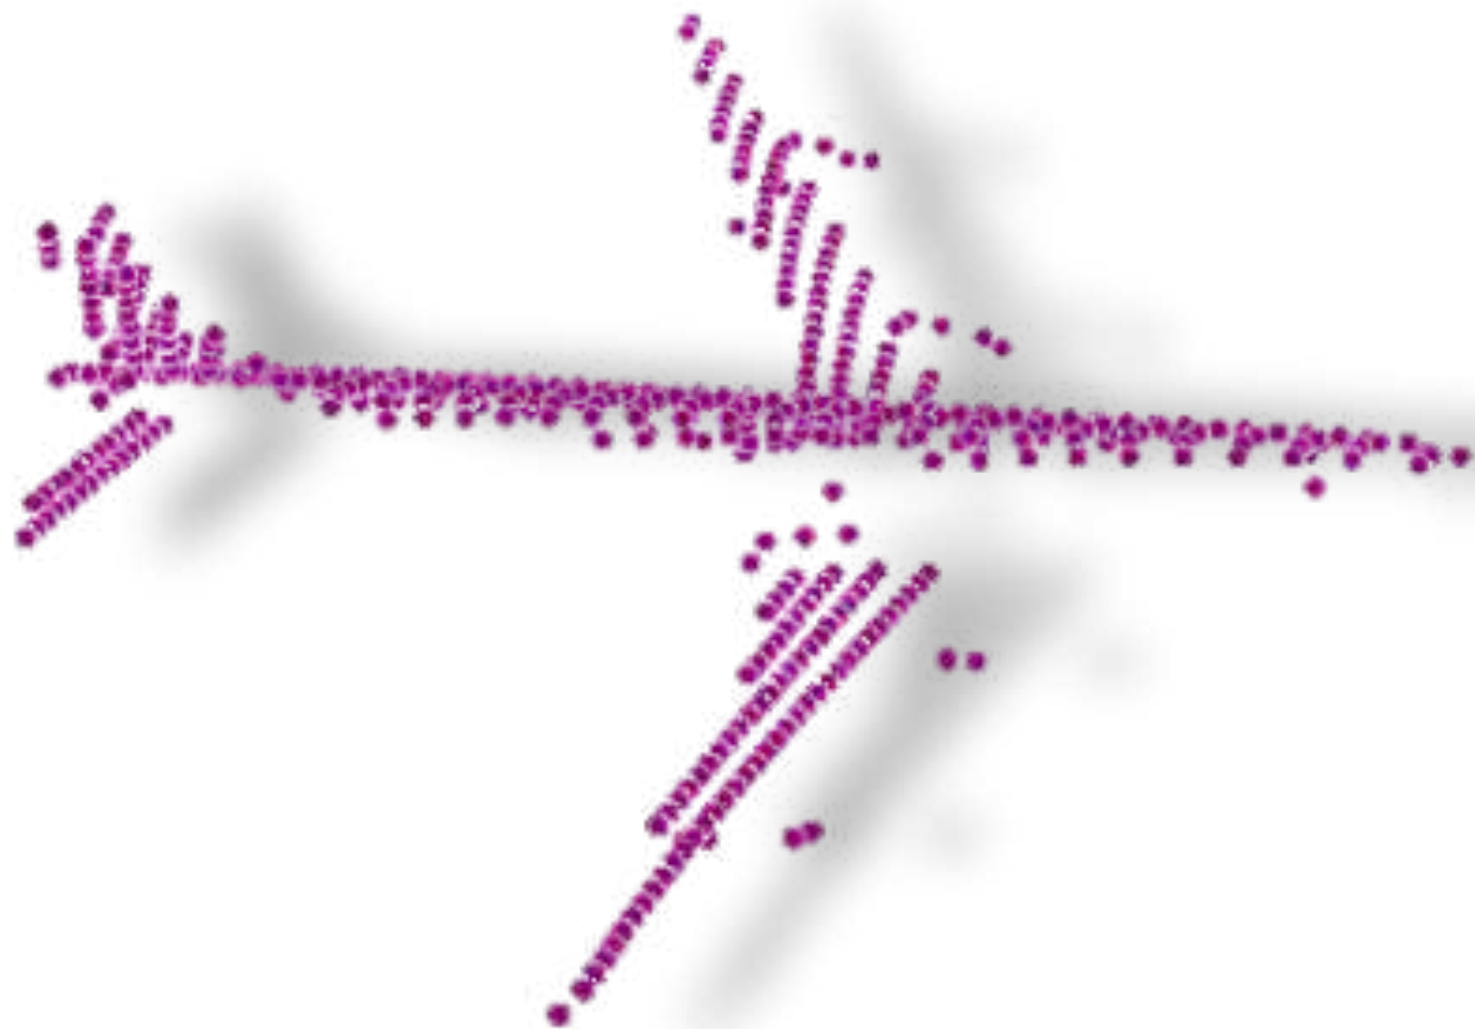



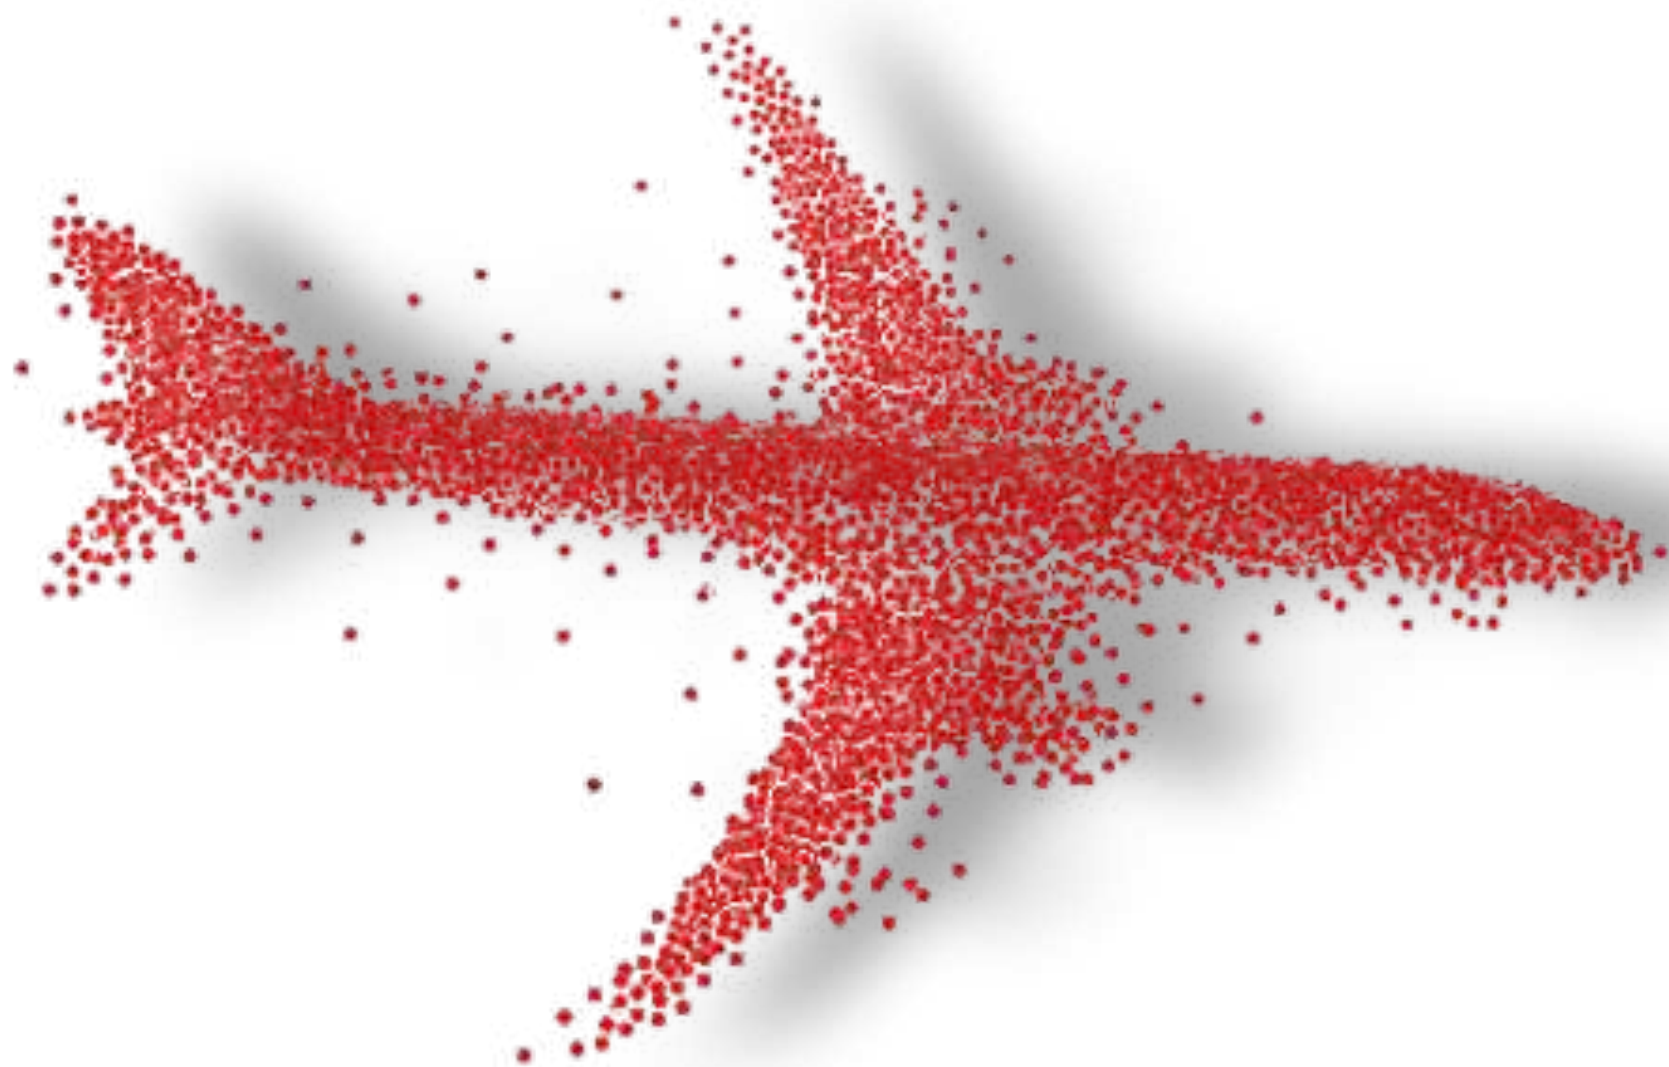

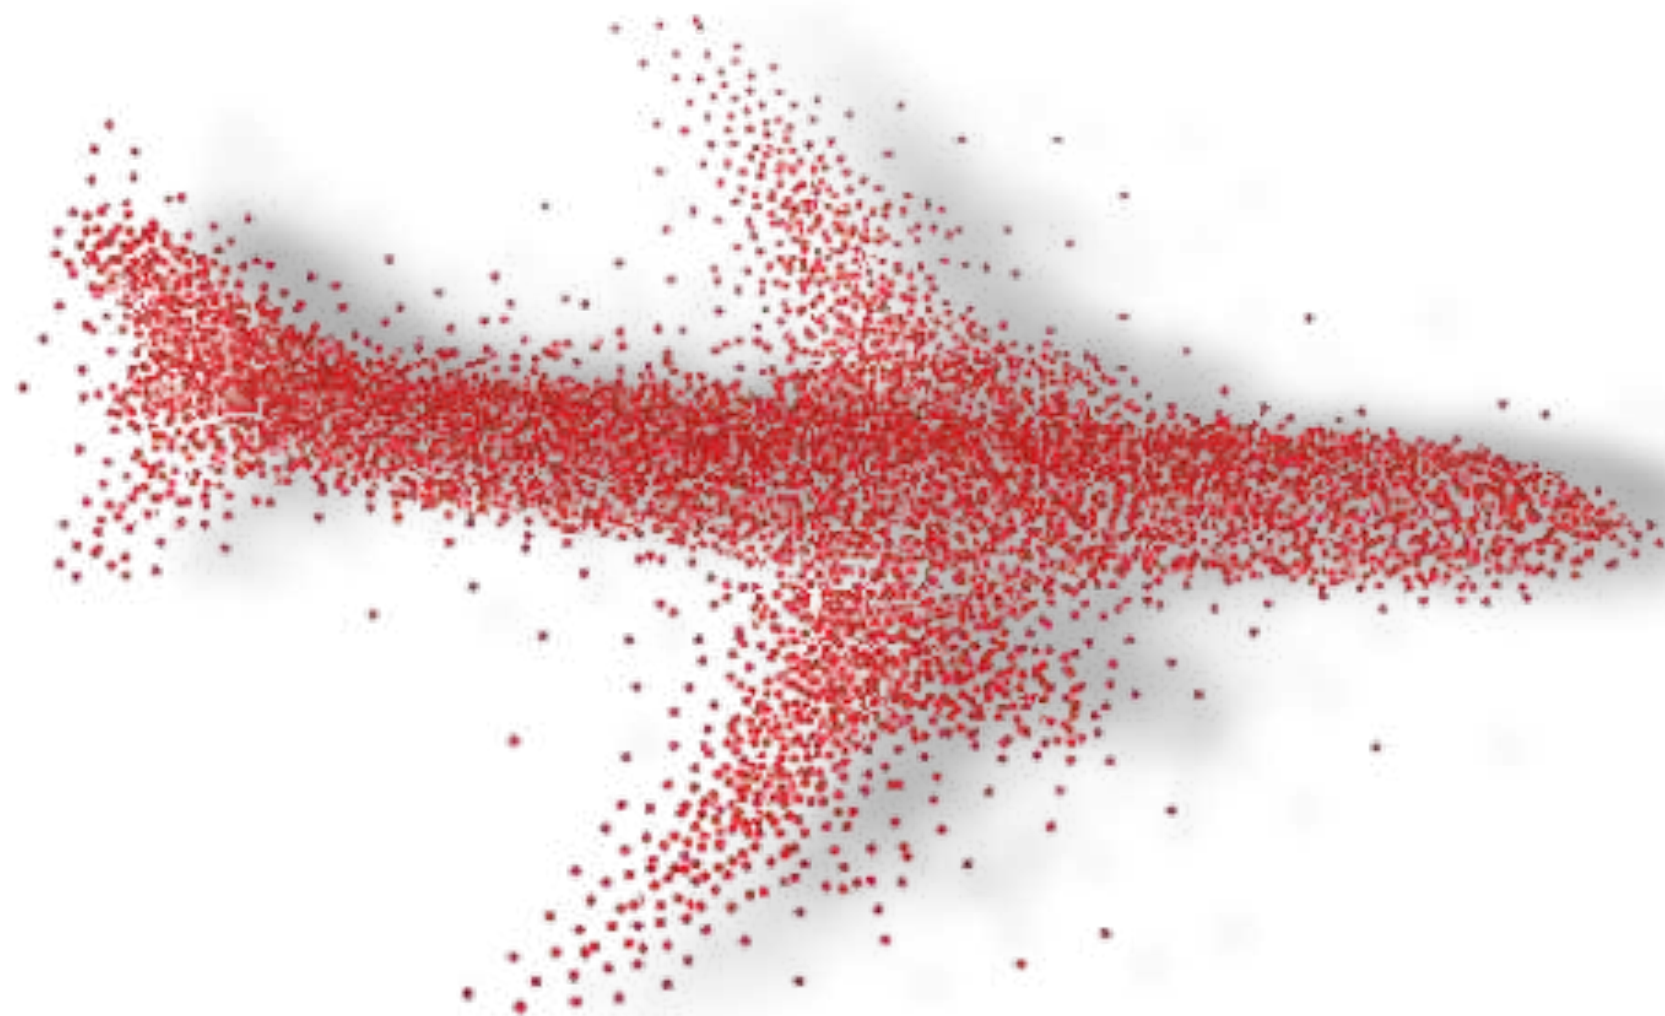

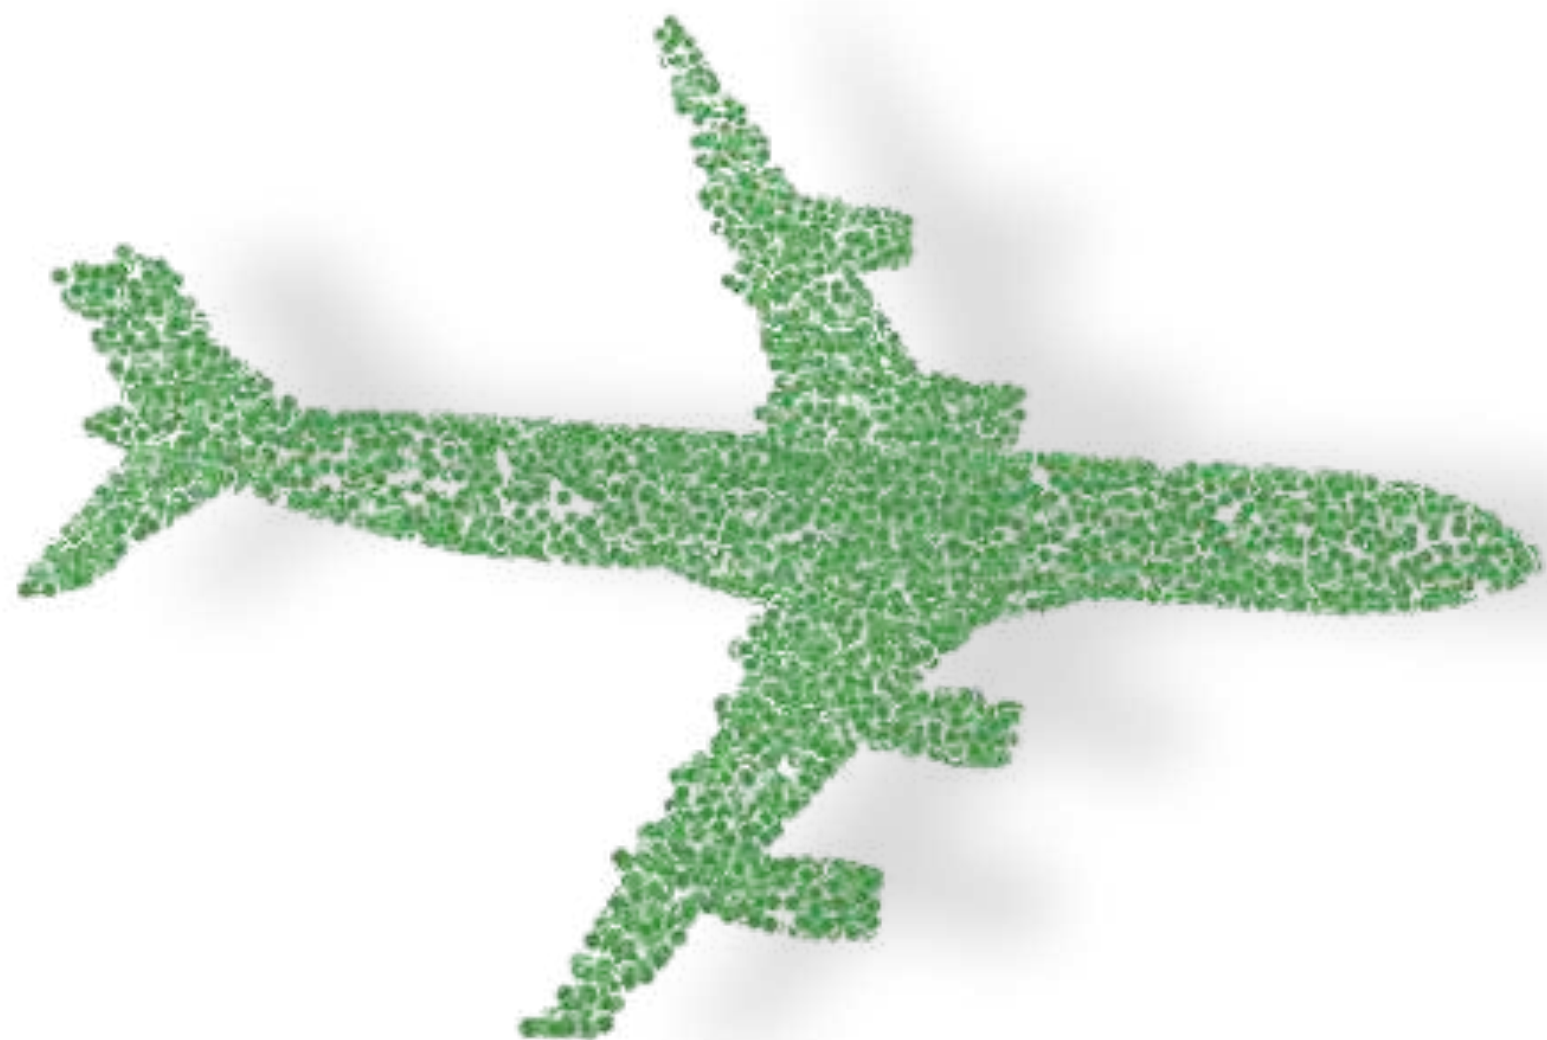



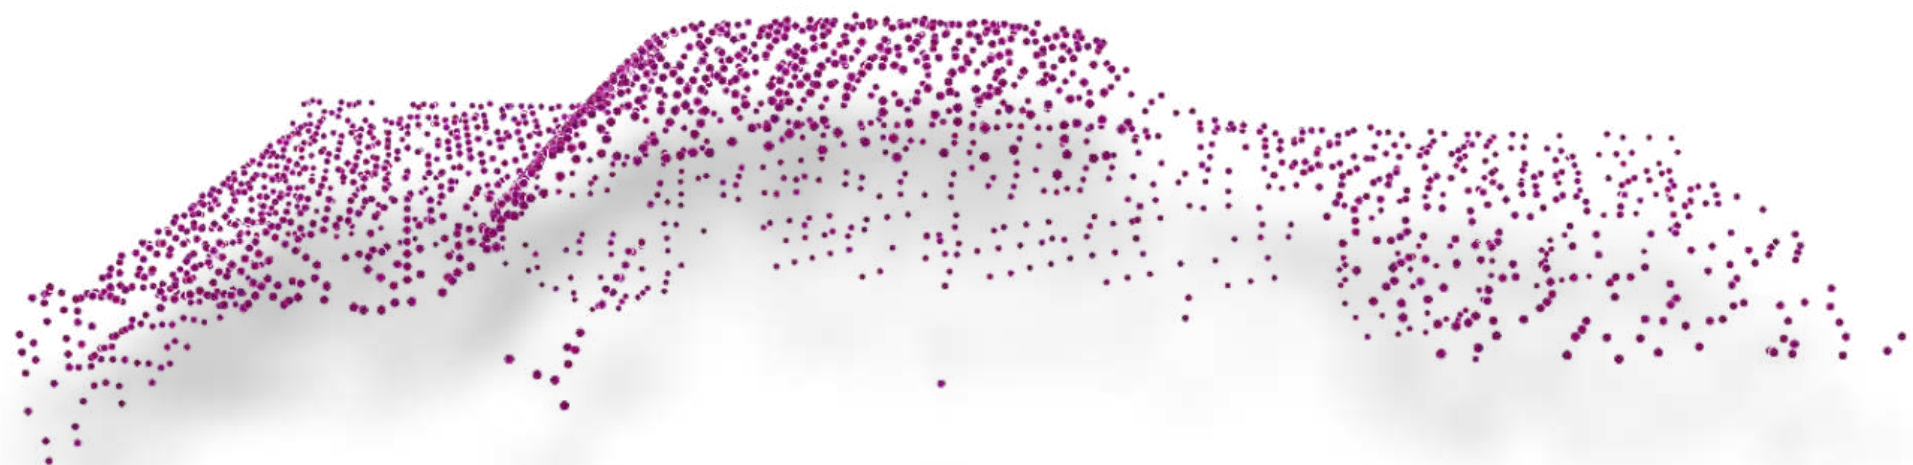

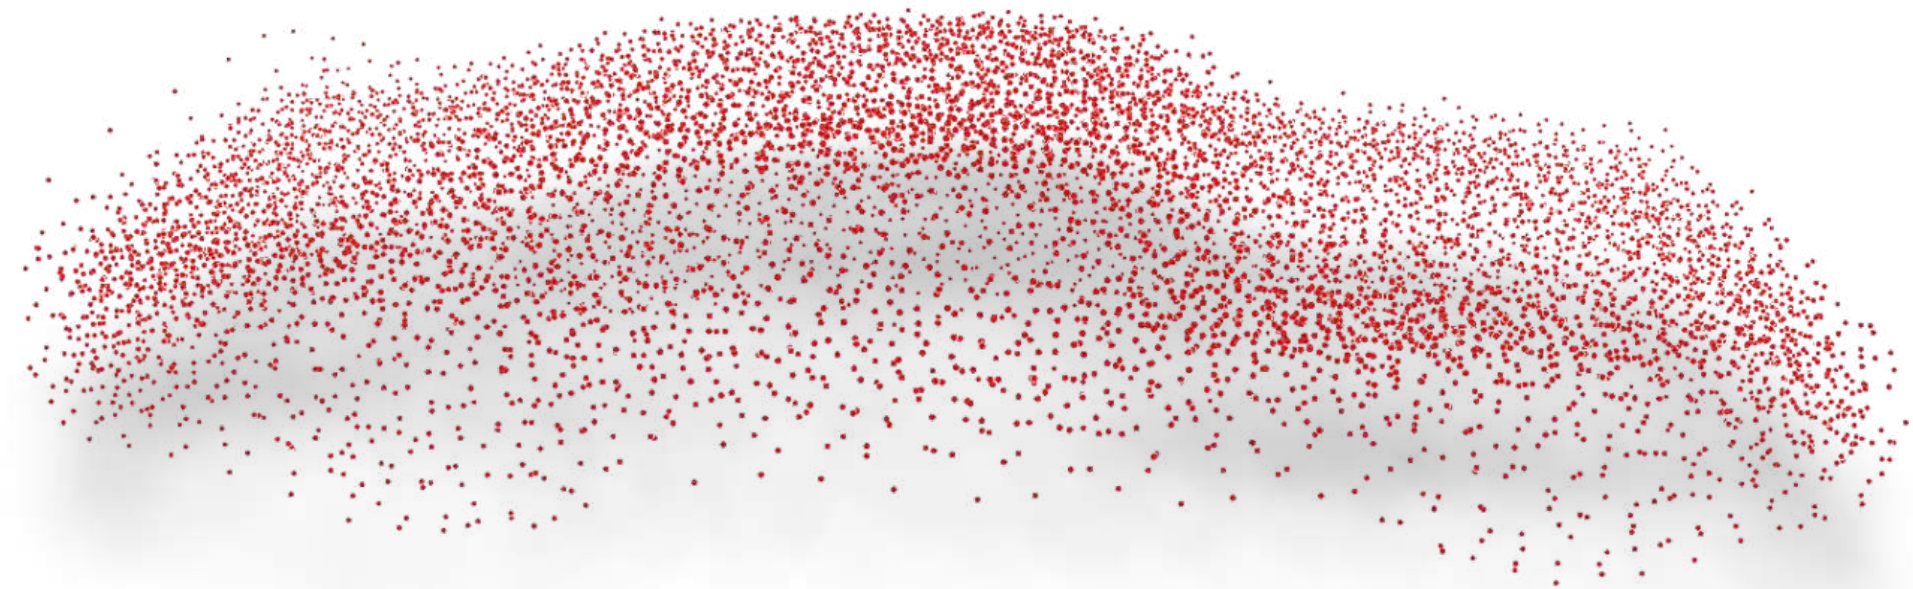

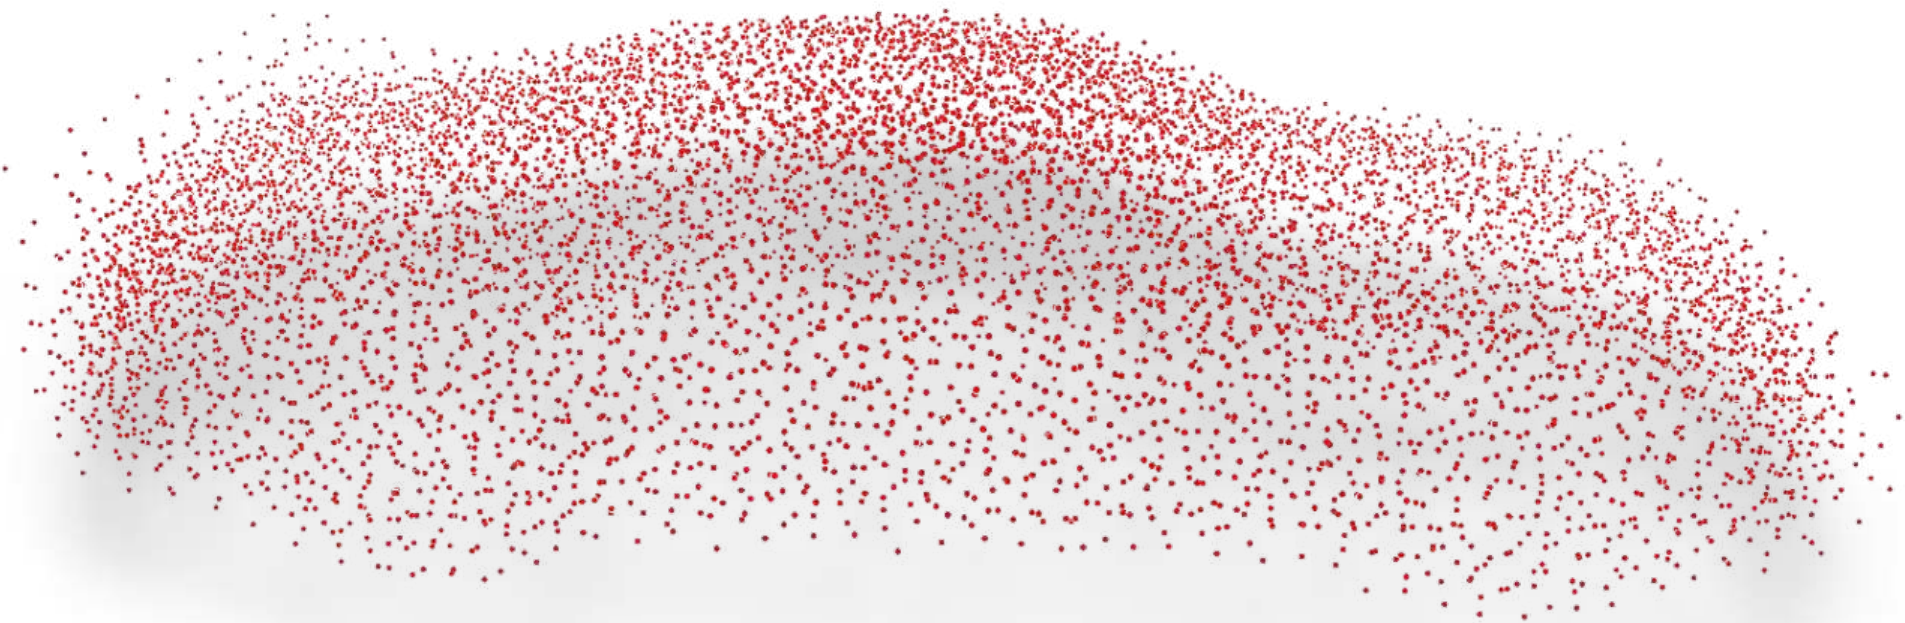



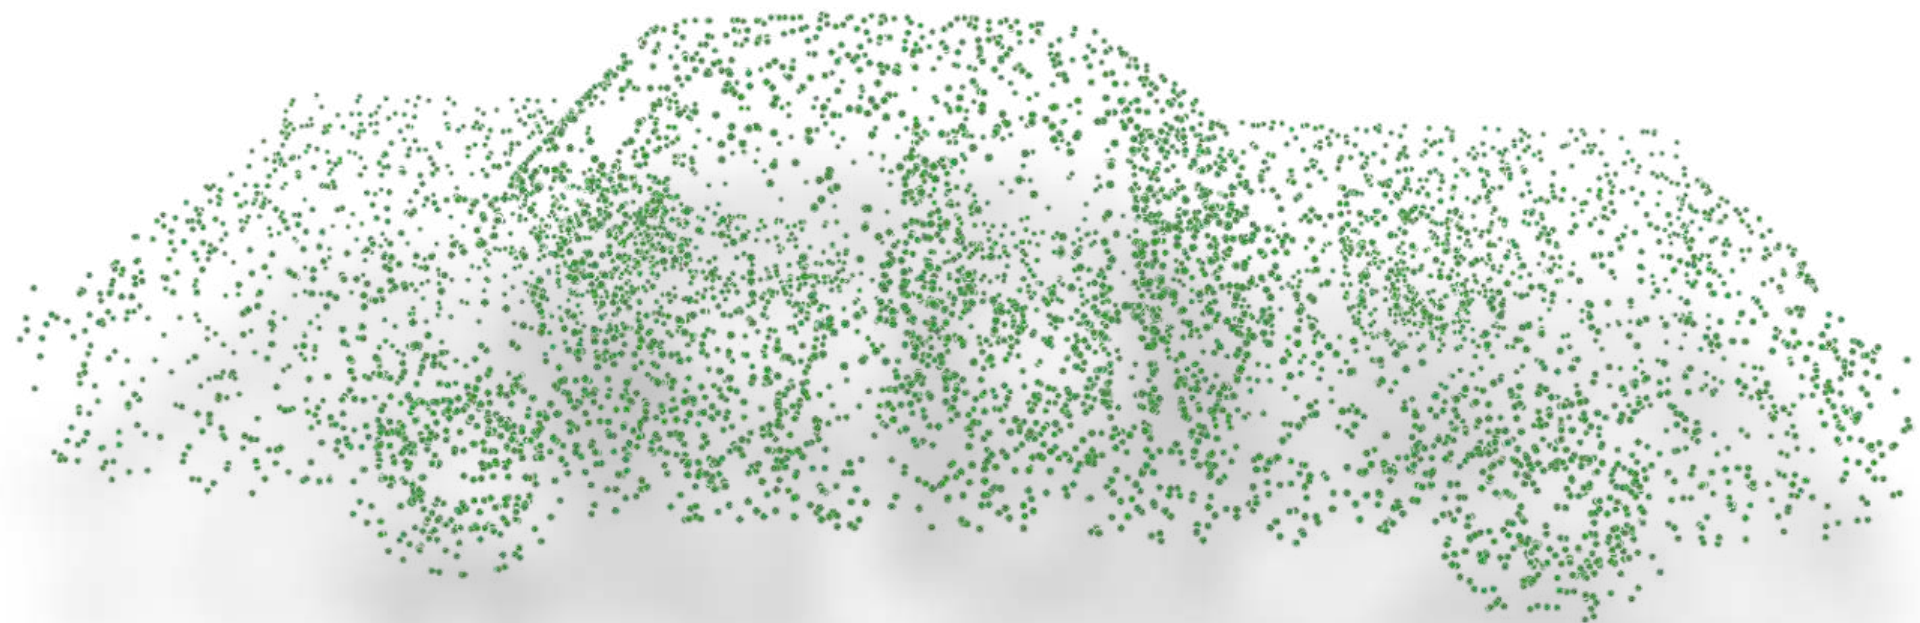

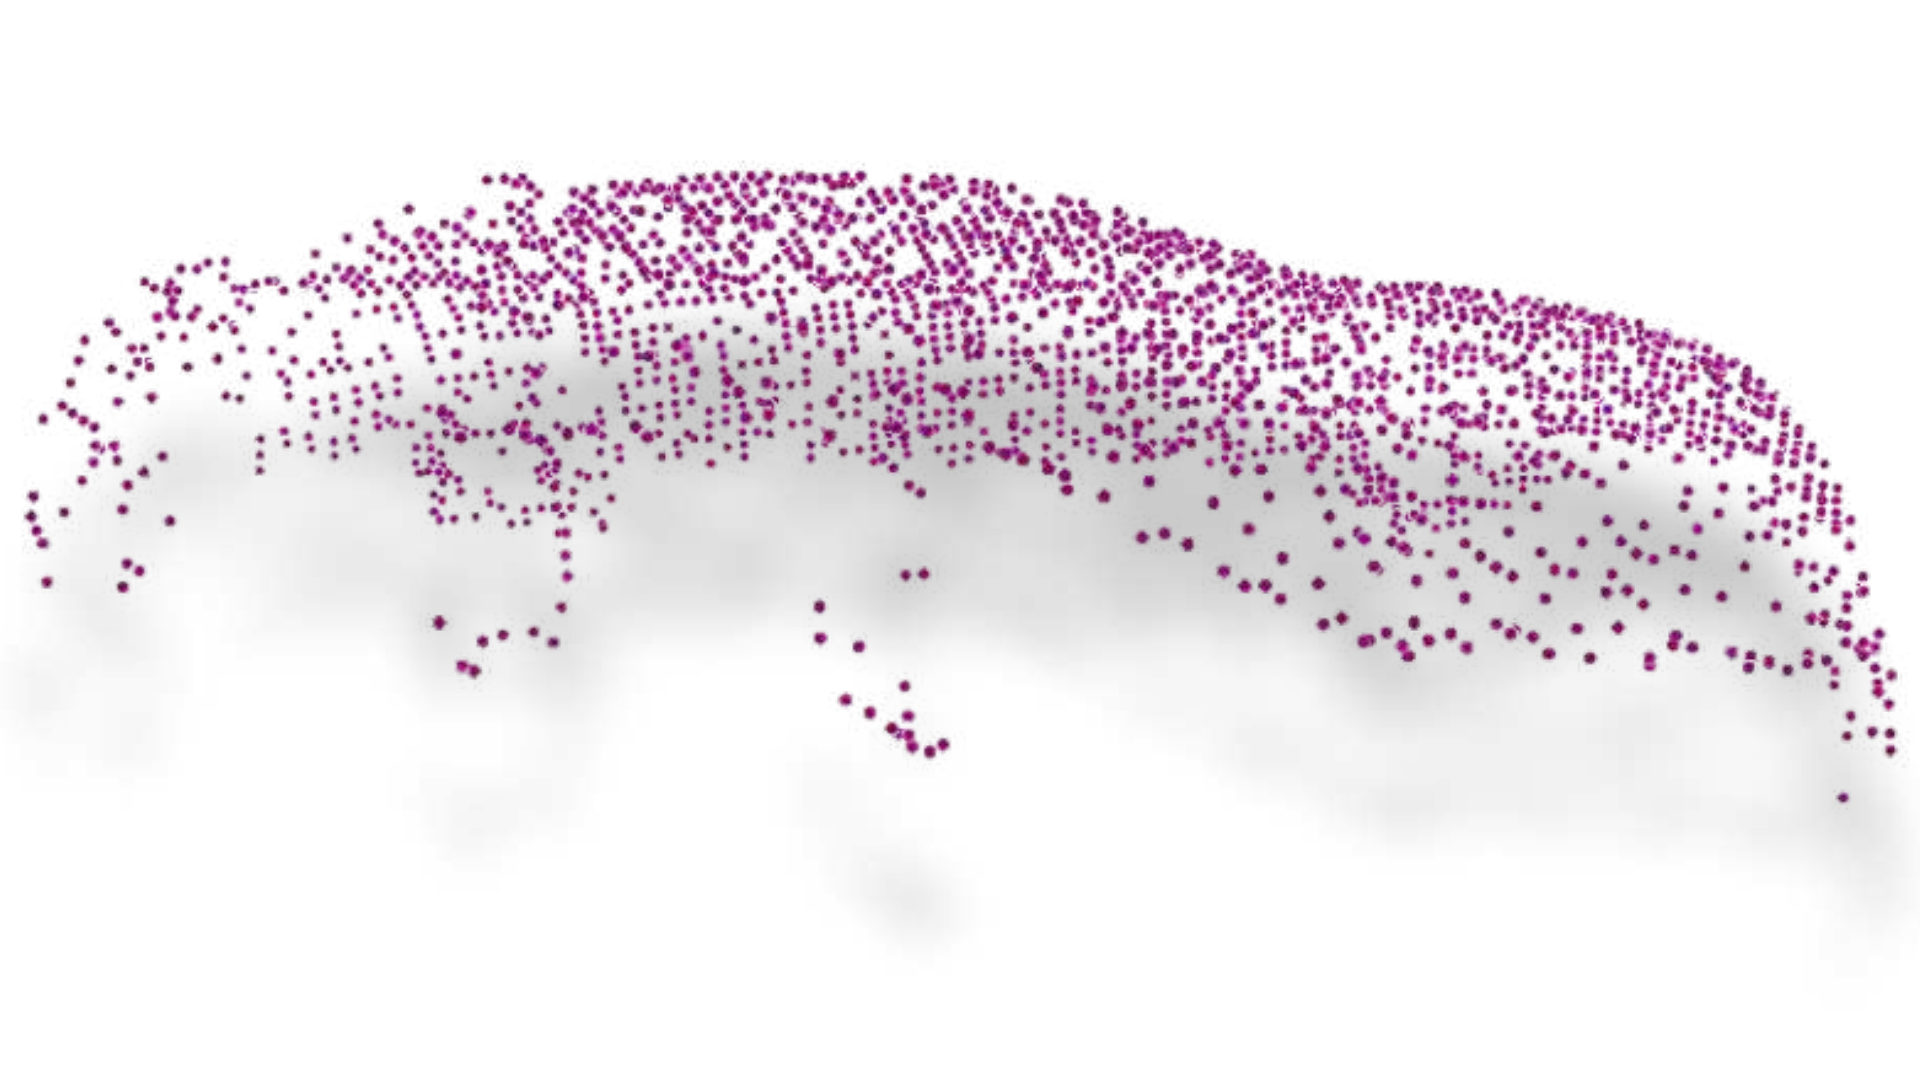



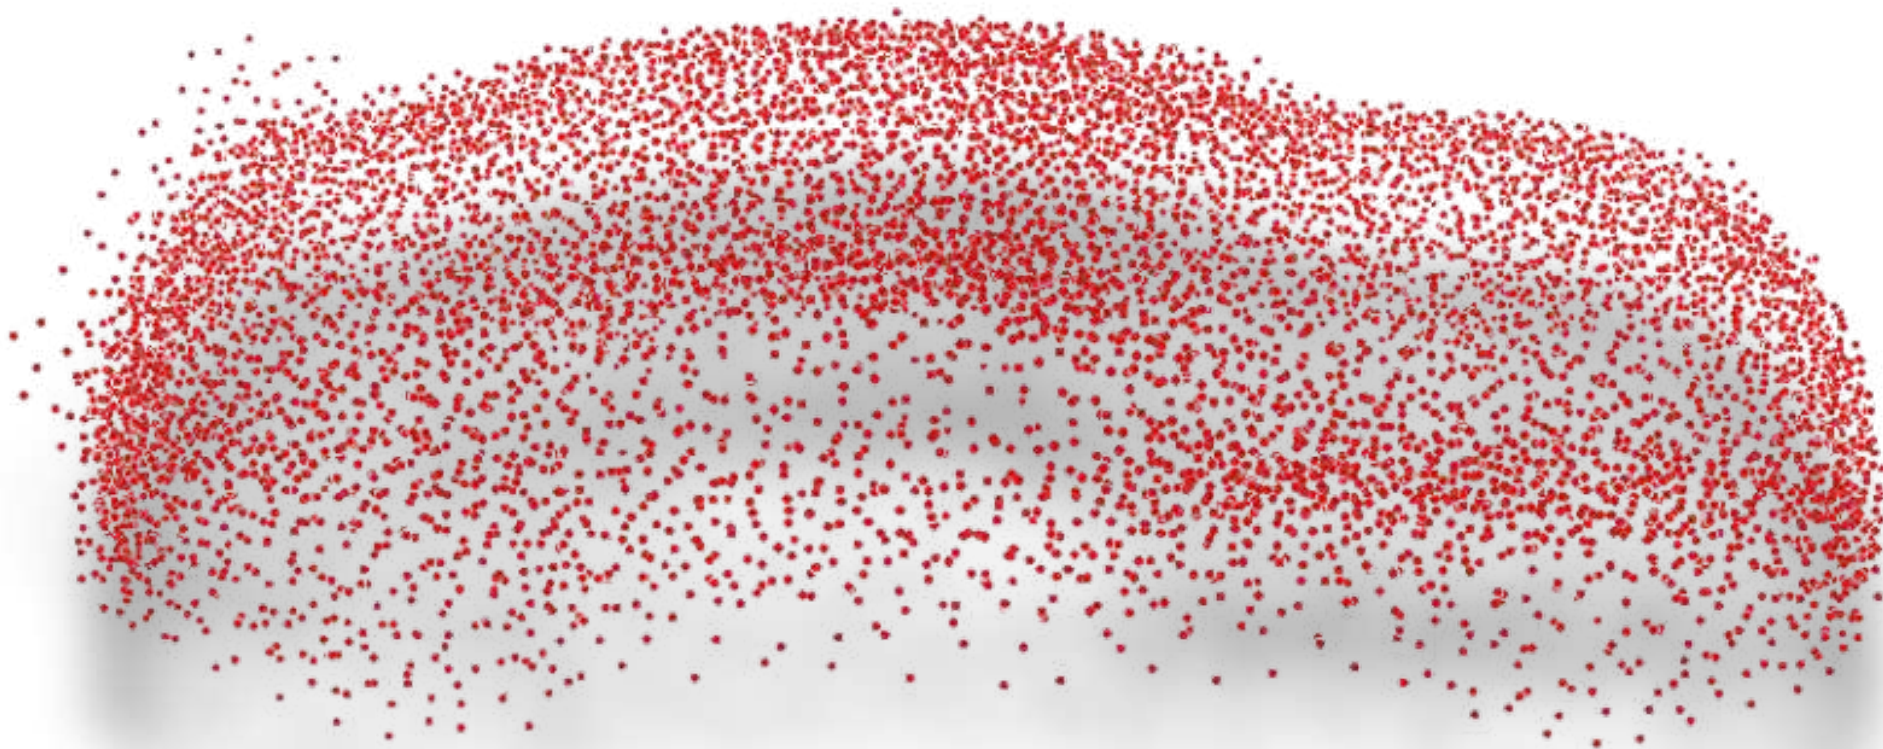

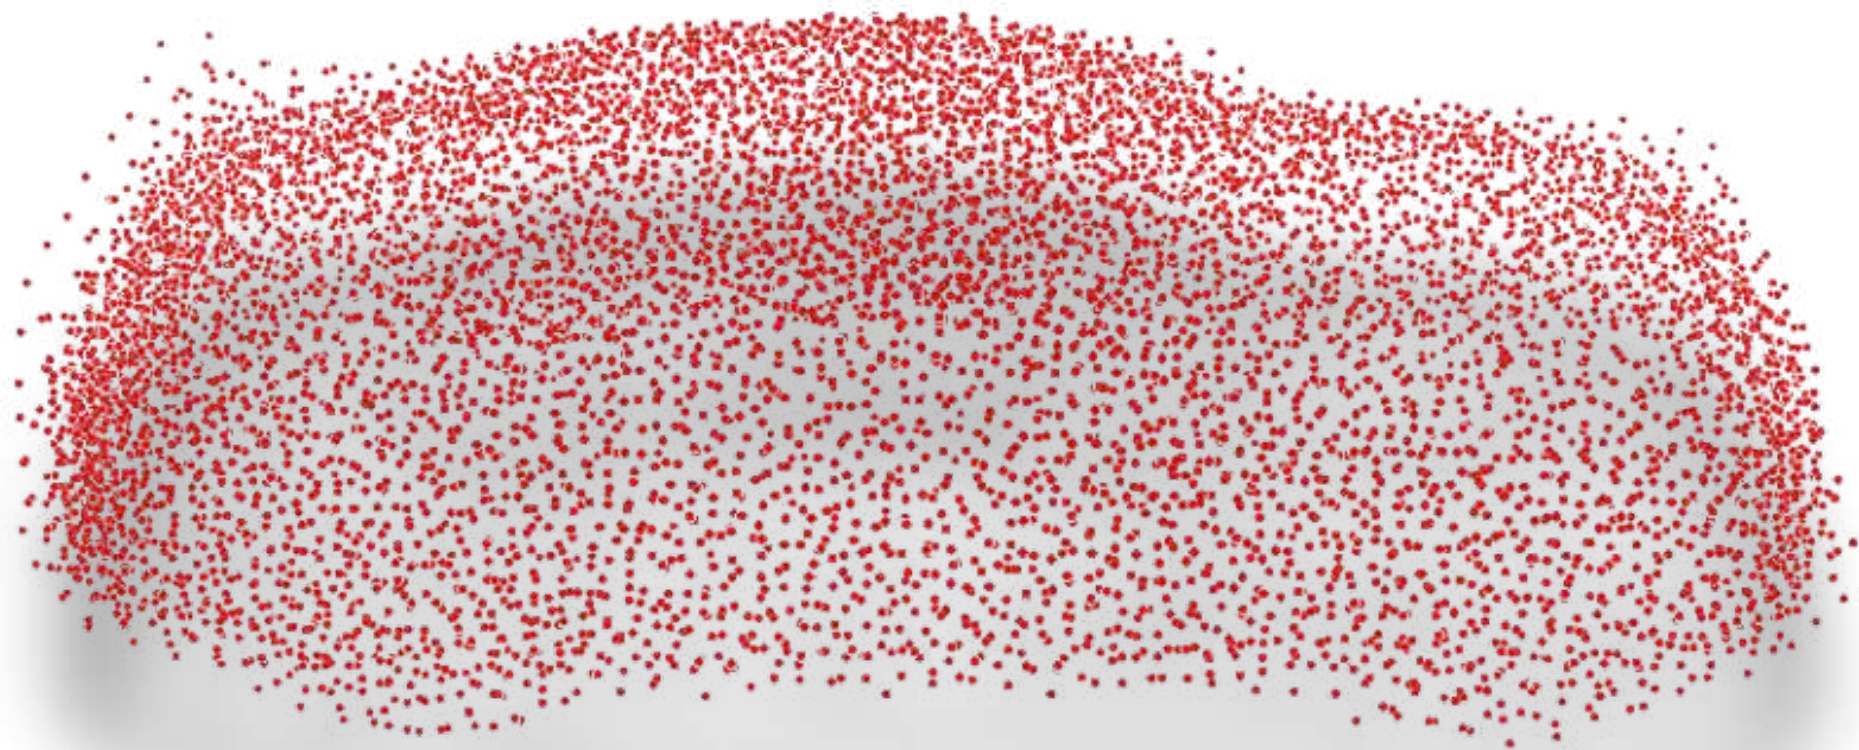



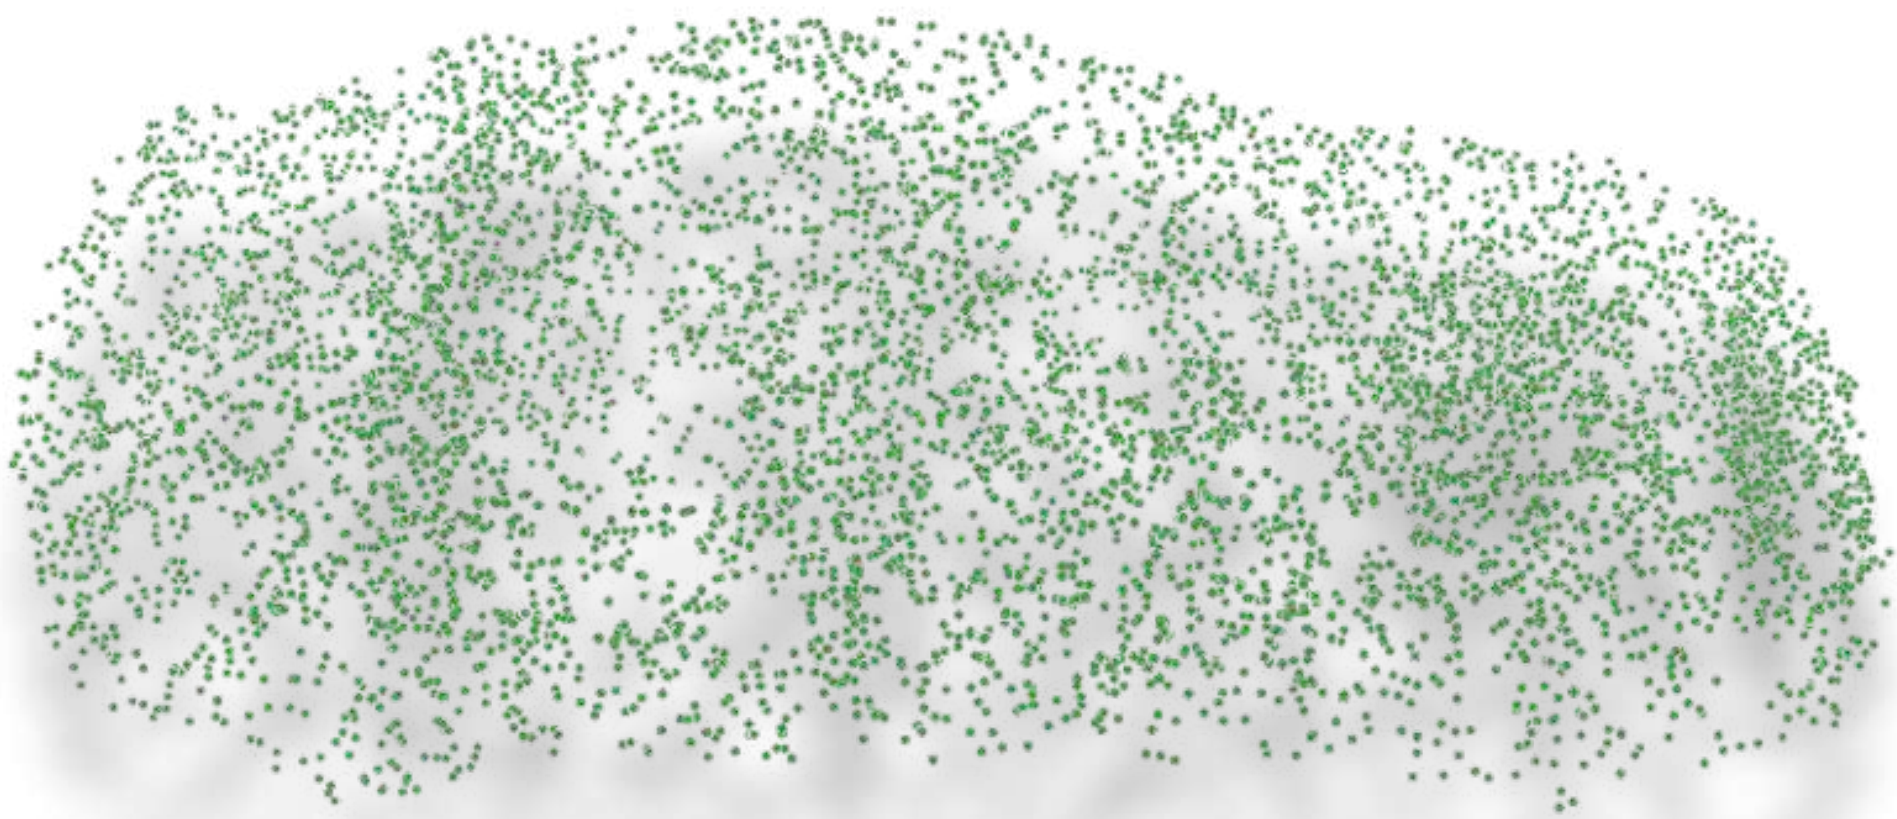

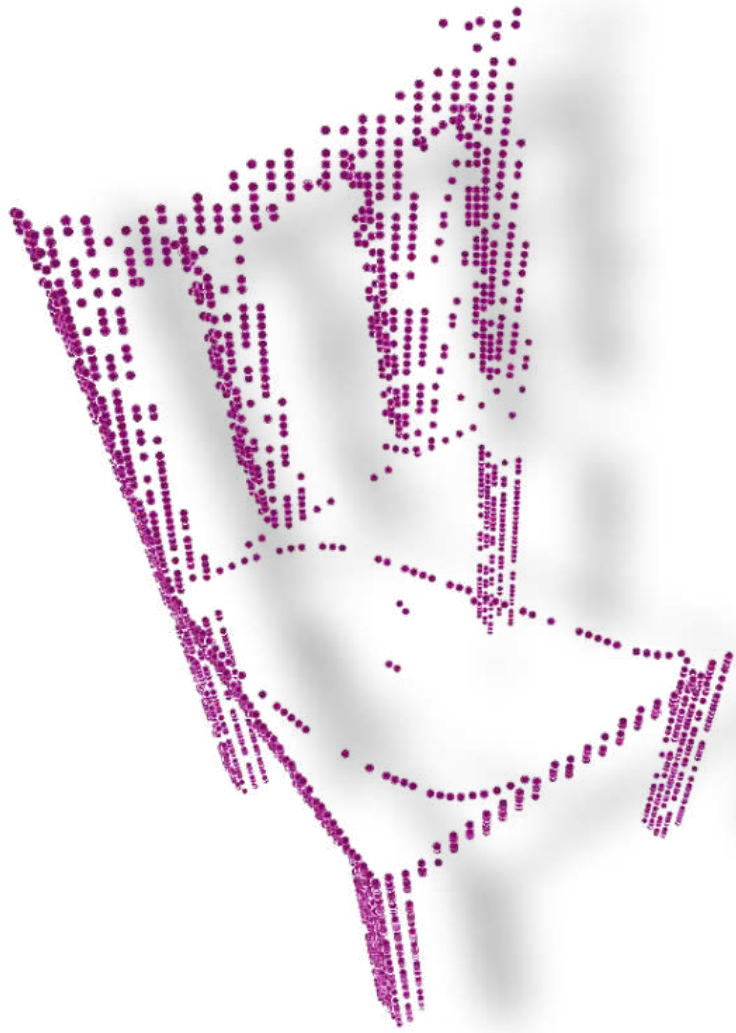

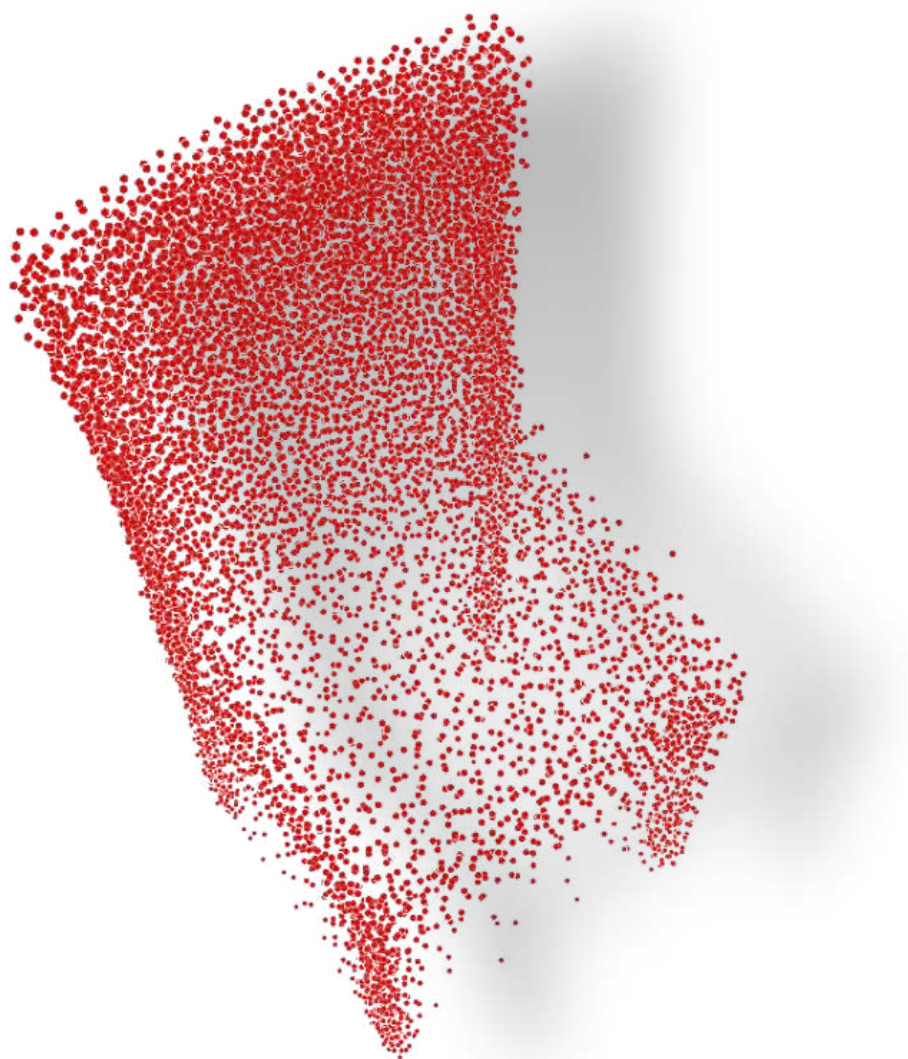



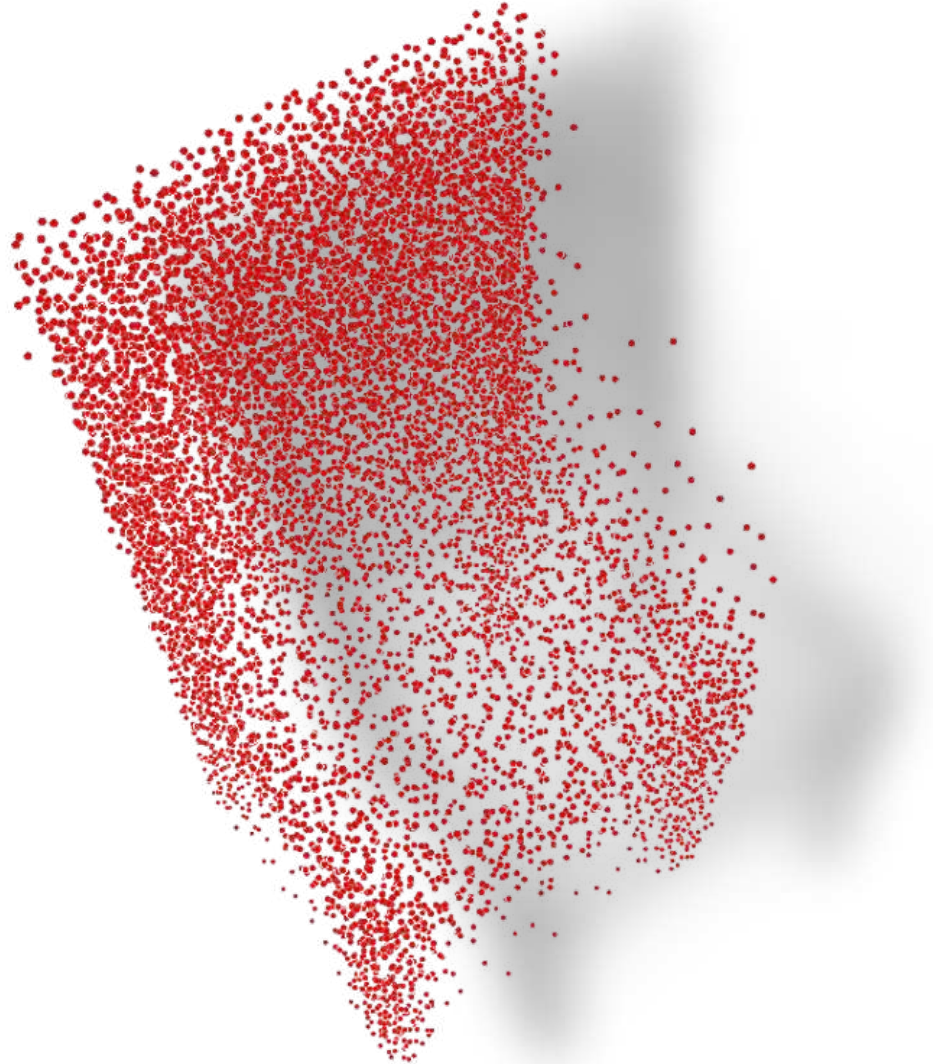

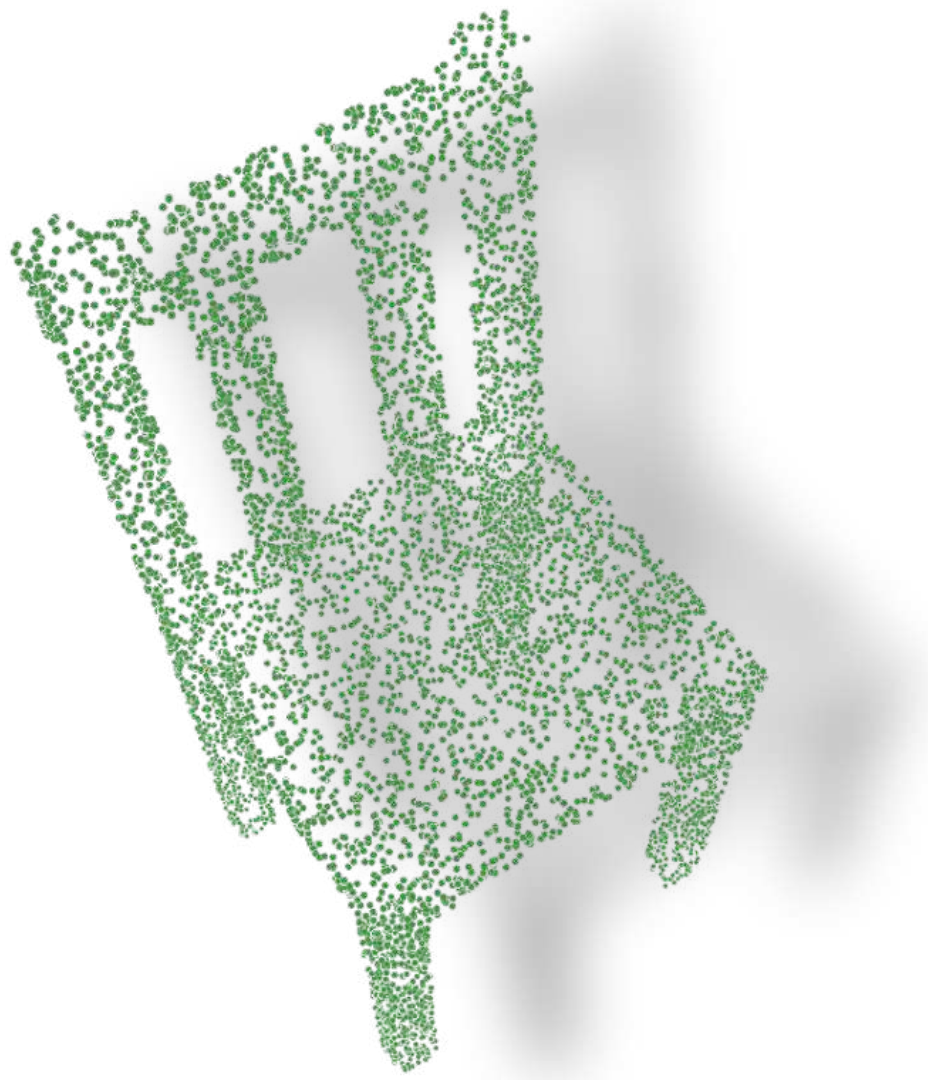

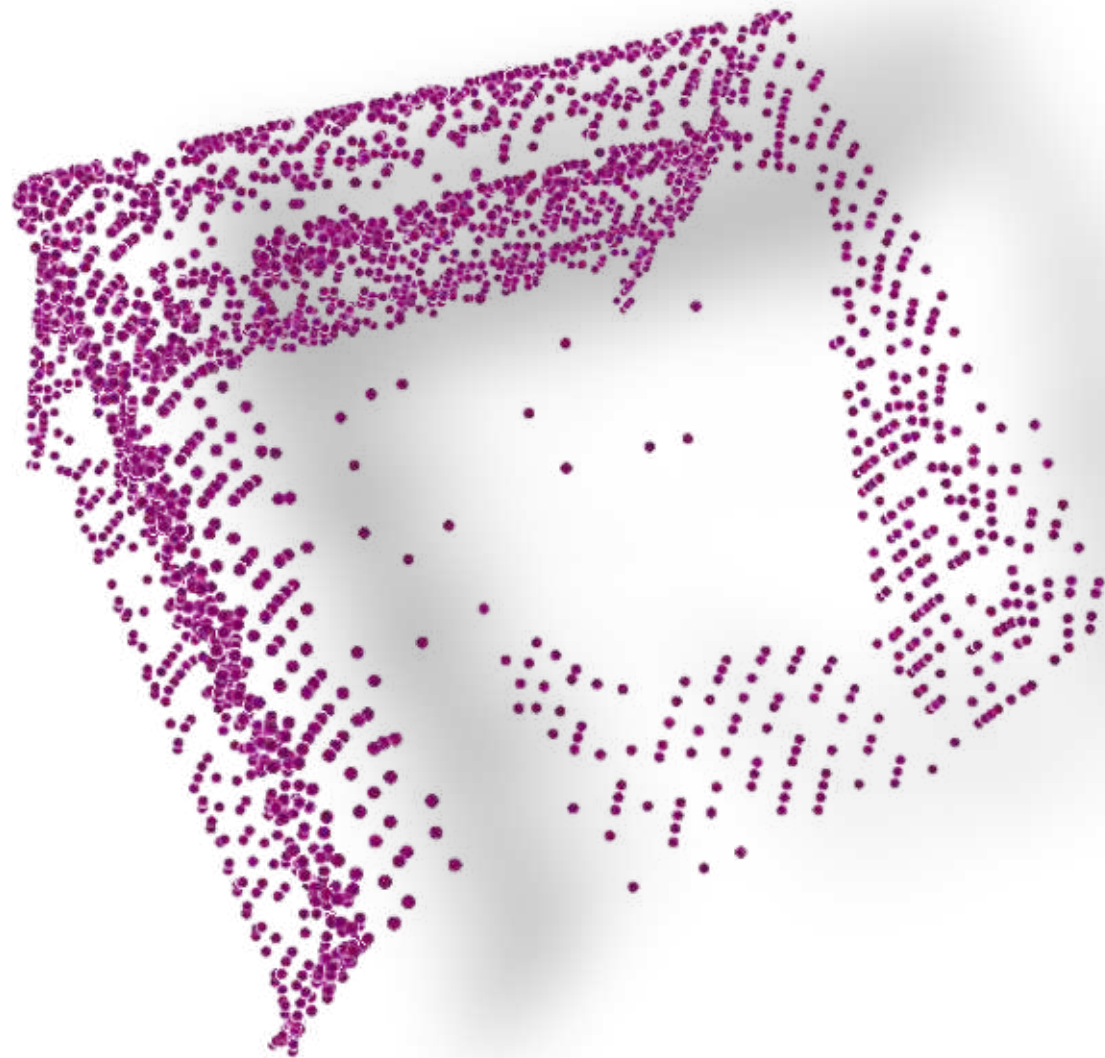

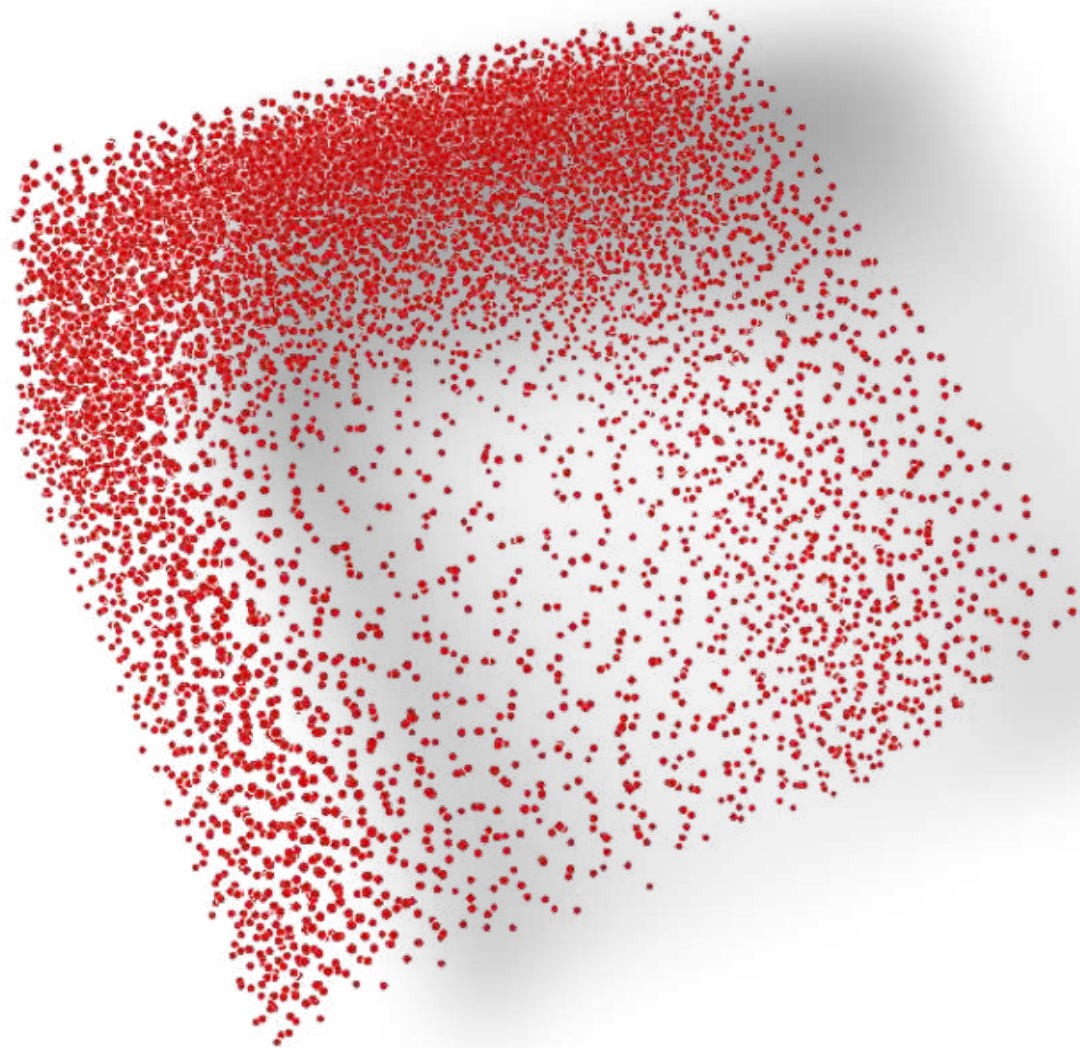



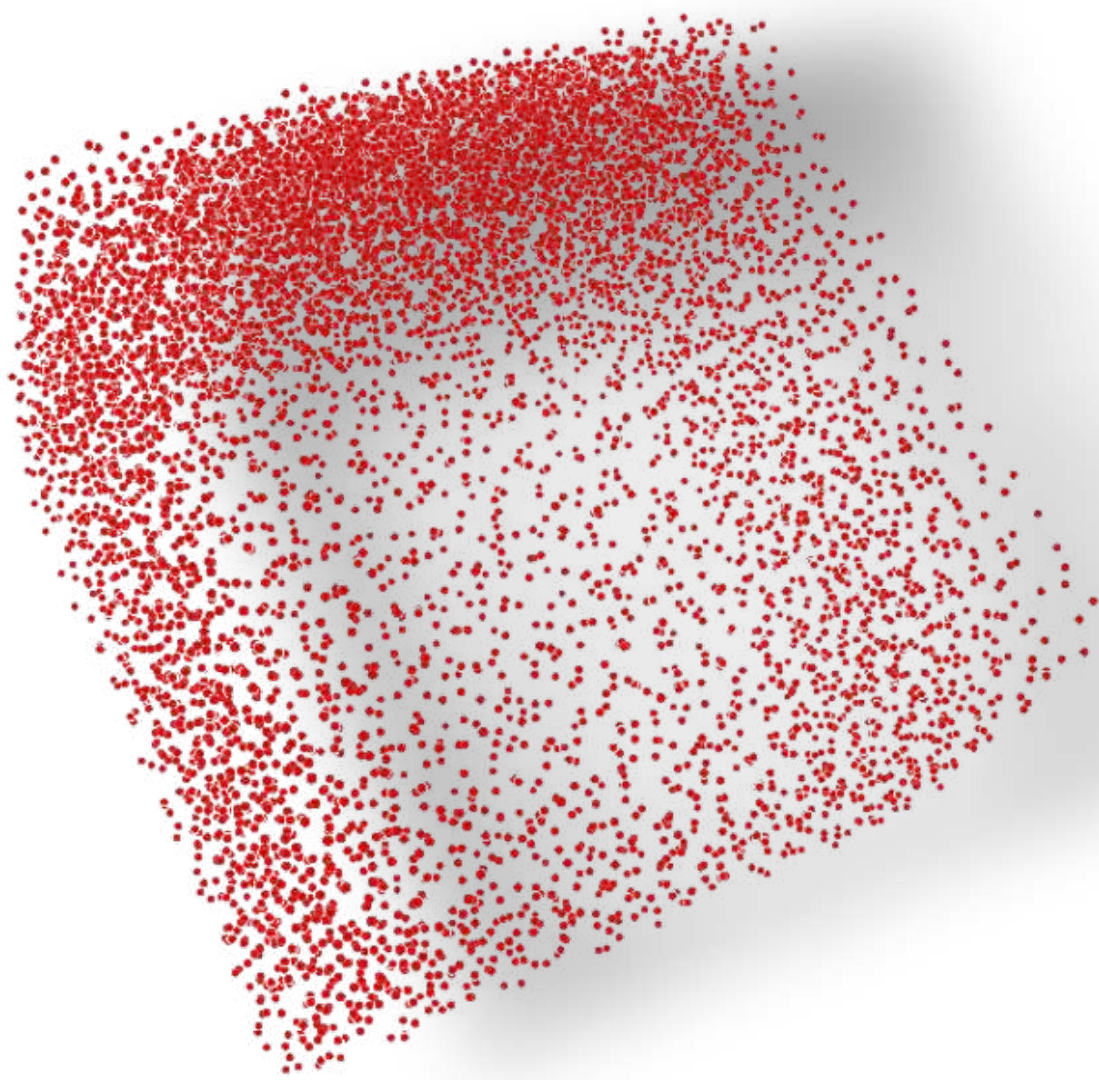



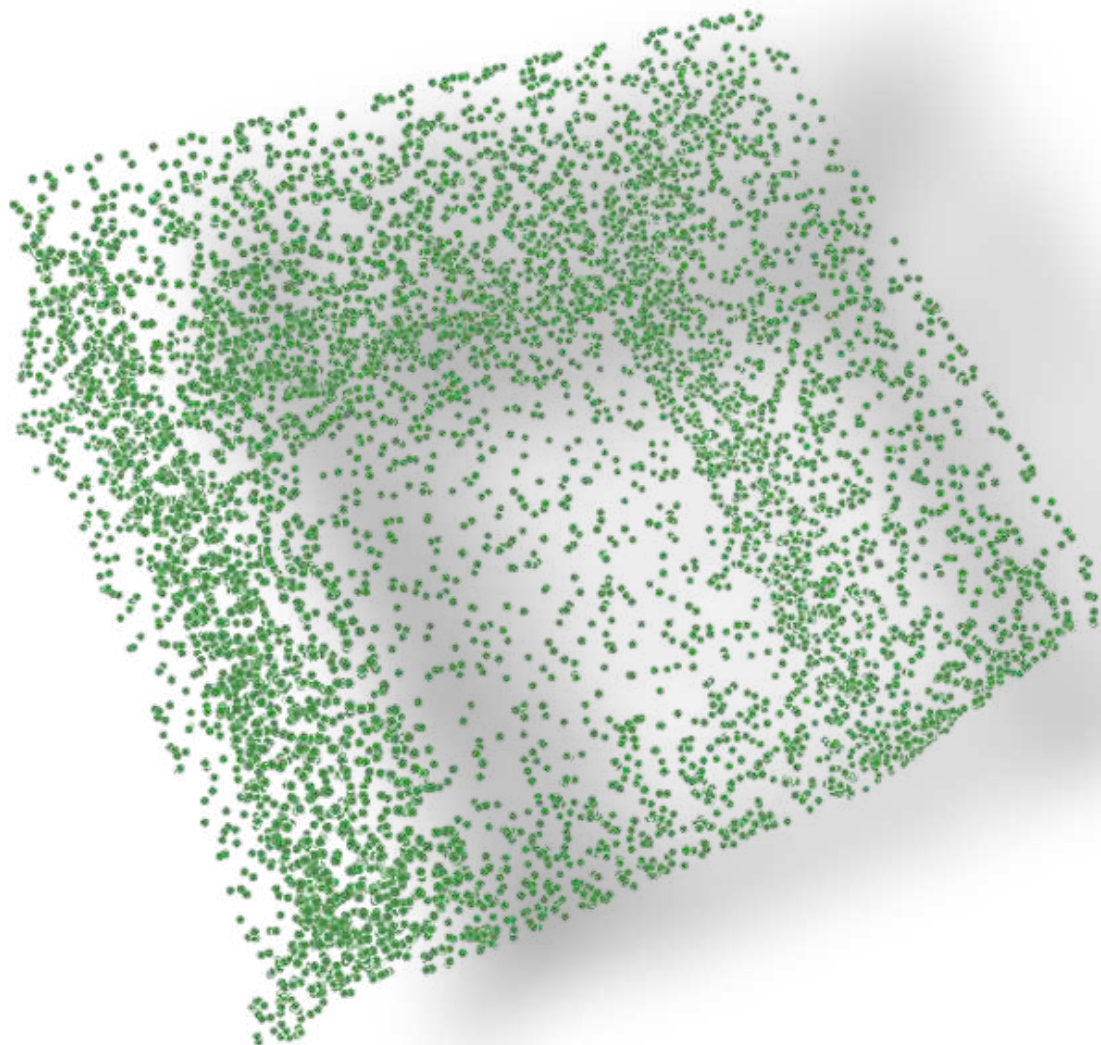

Supplement: Supplementary file 6 [file supp_multi.pdf]
