# Supplementary material for: ACL-SPC: Adaptive Closed-Loop system for Self-Supervised Point Cloud Completion
Source: arXiv:2303.01979 source file (2023-03-28)

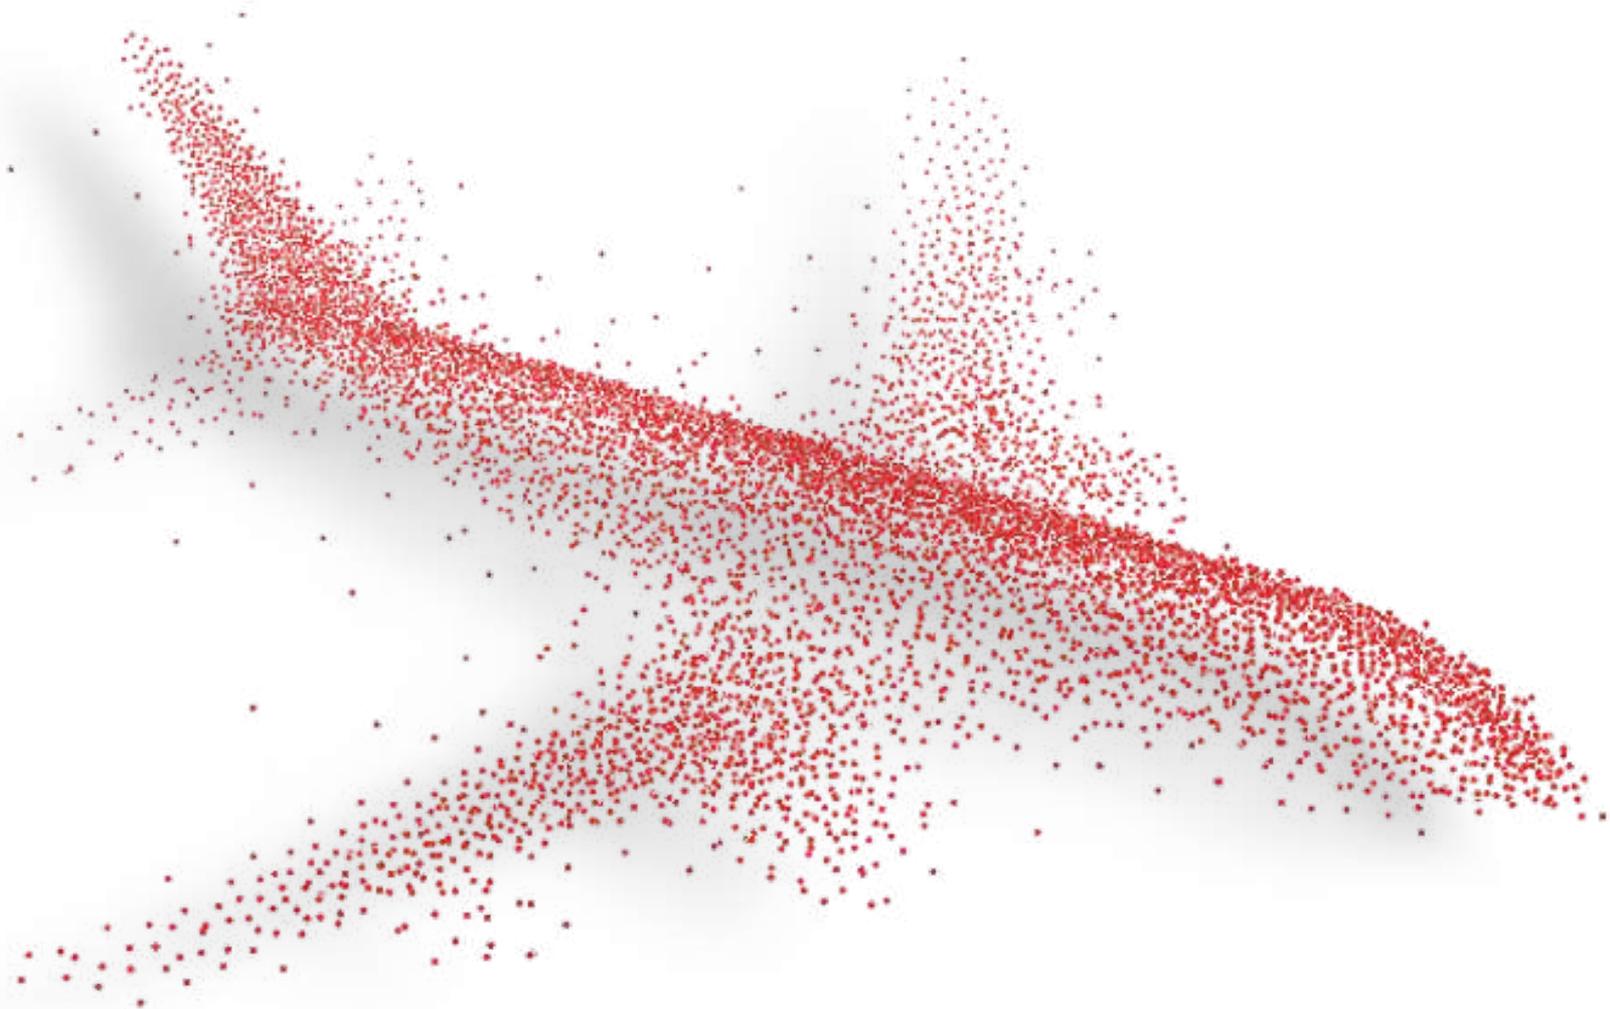

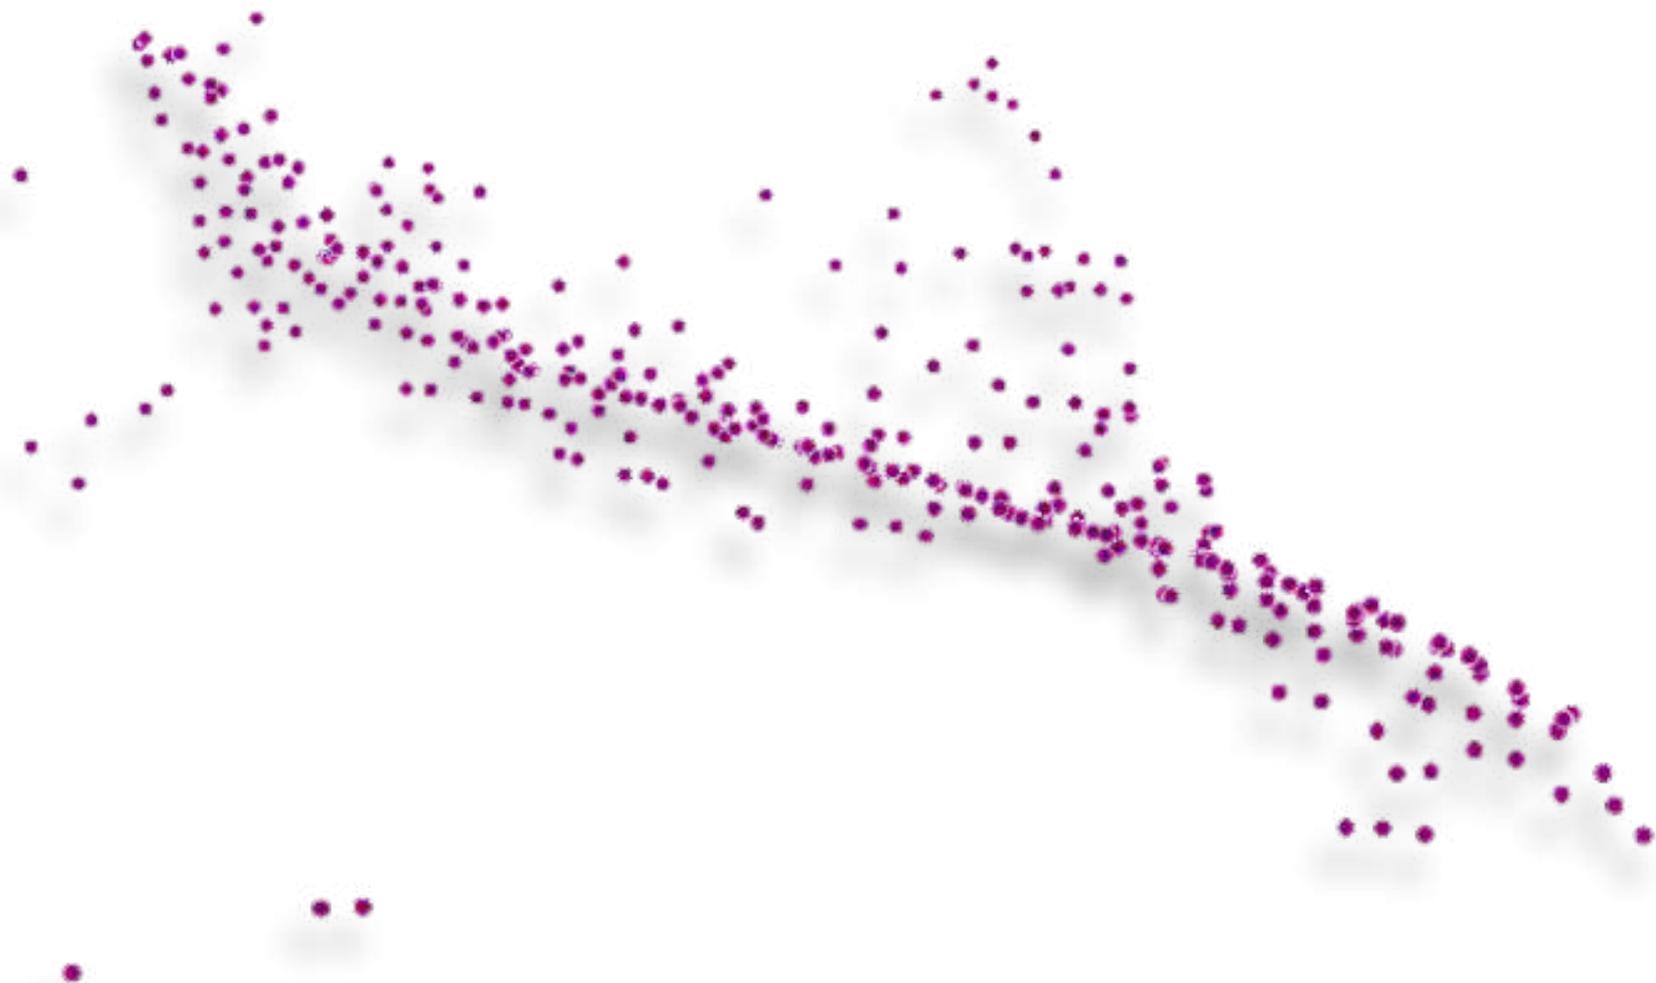

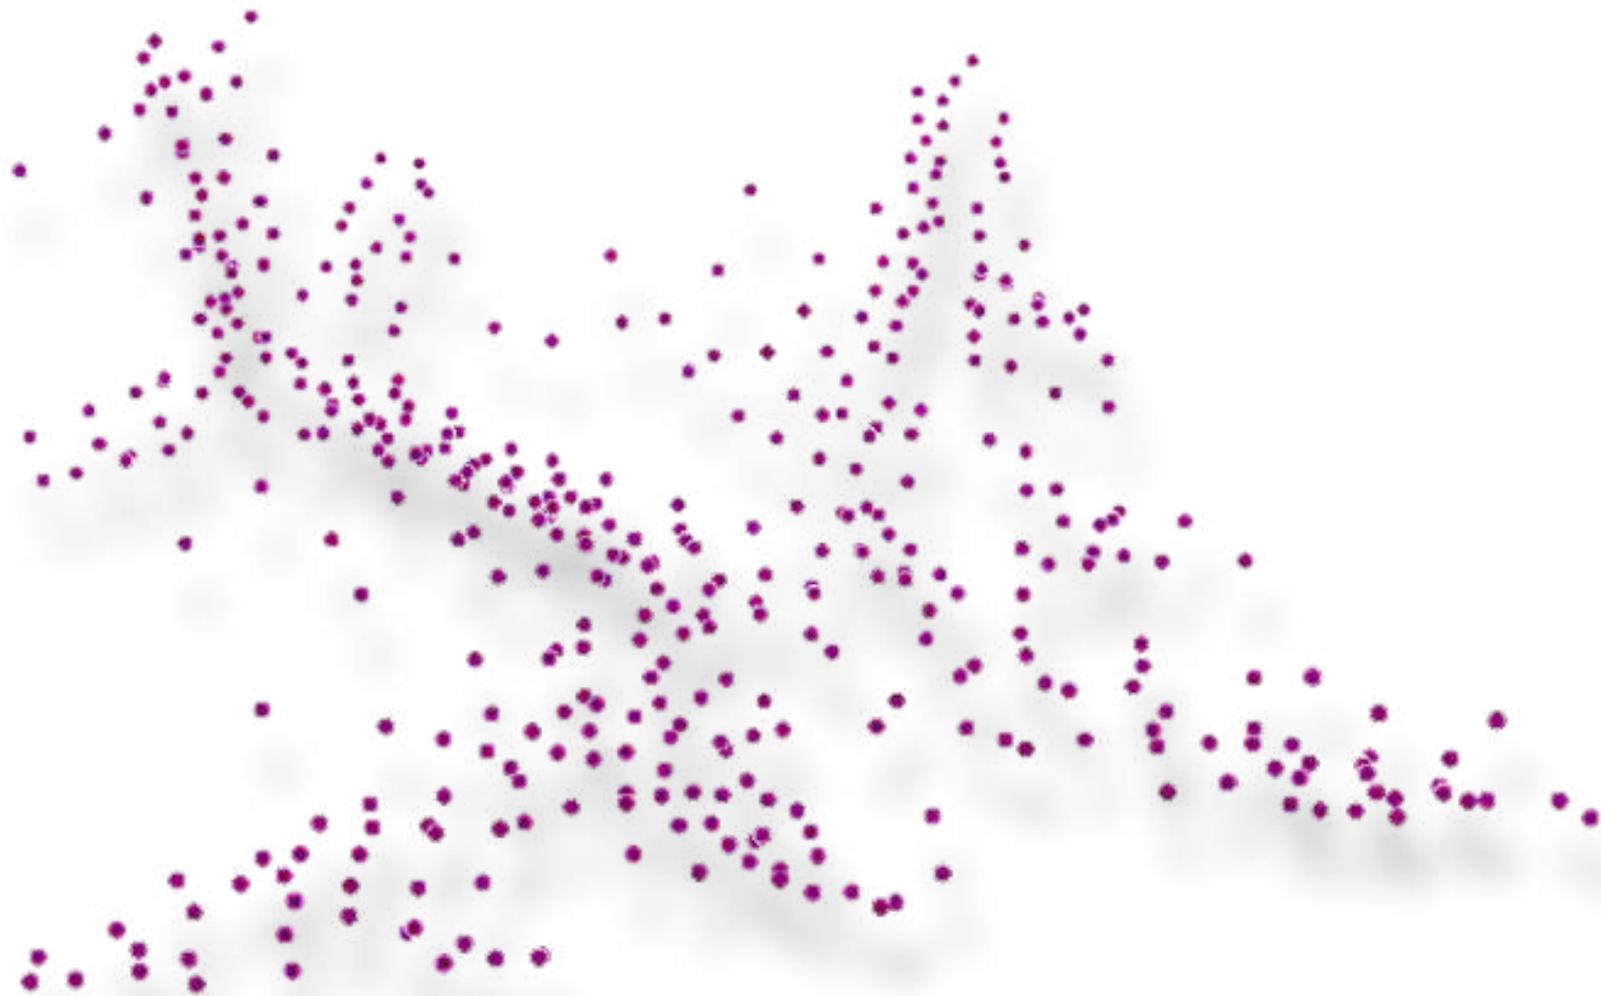

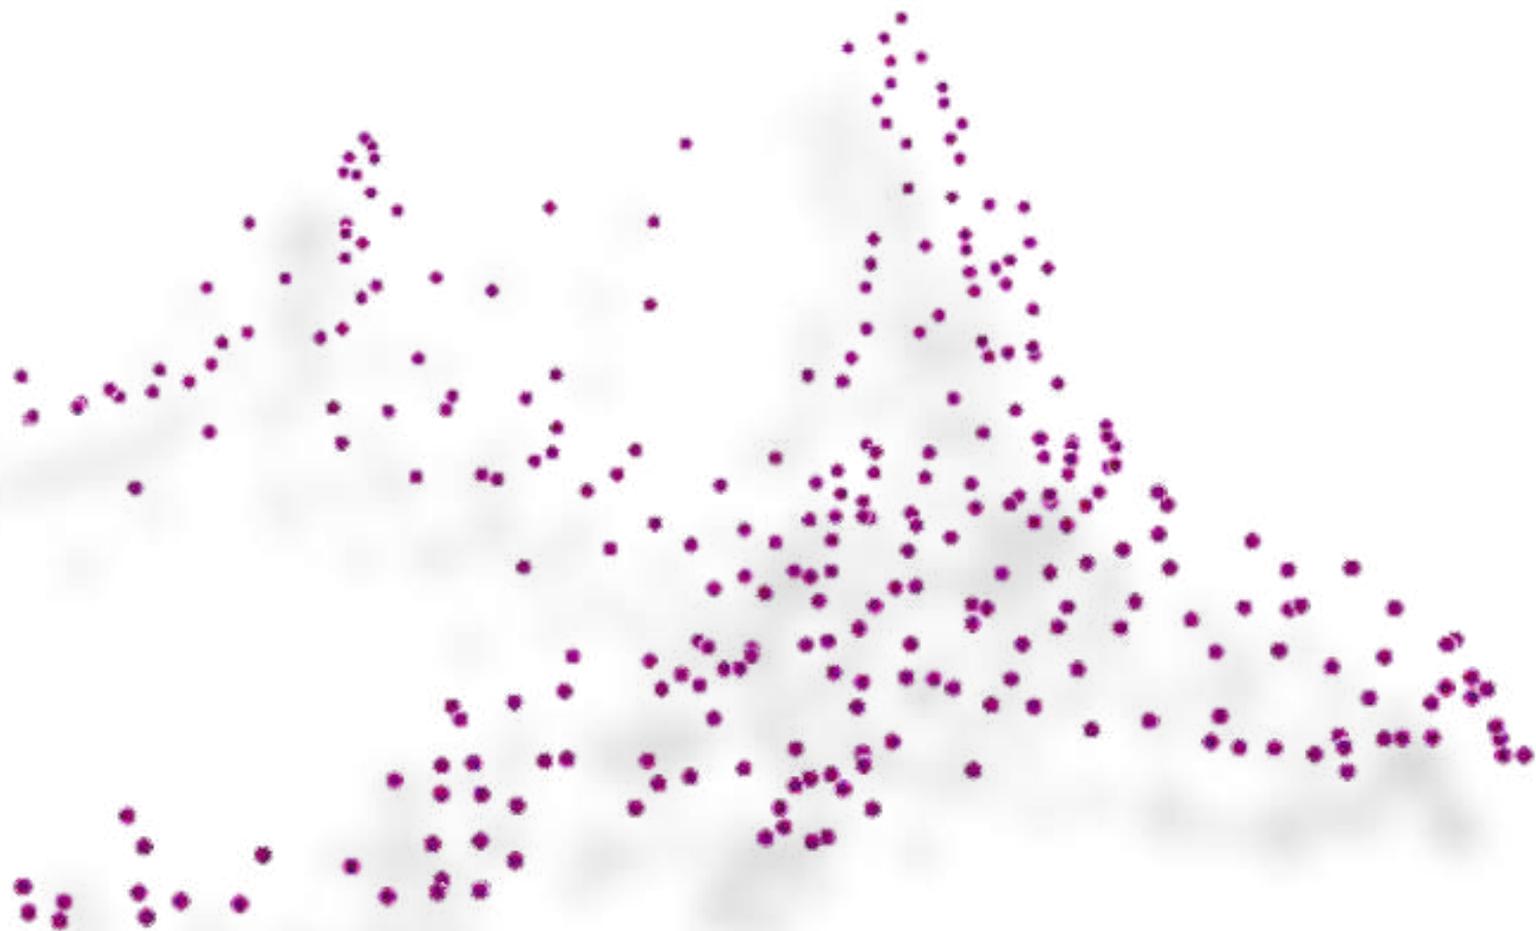

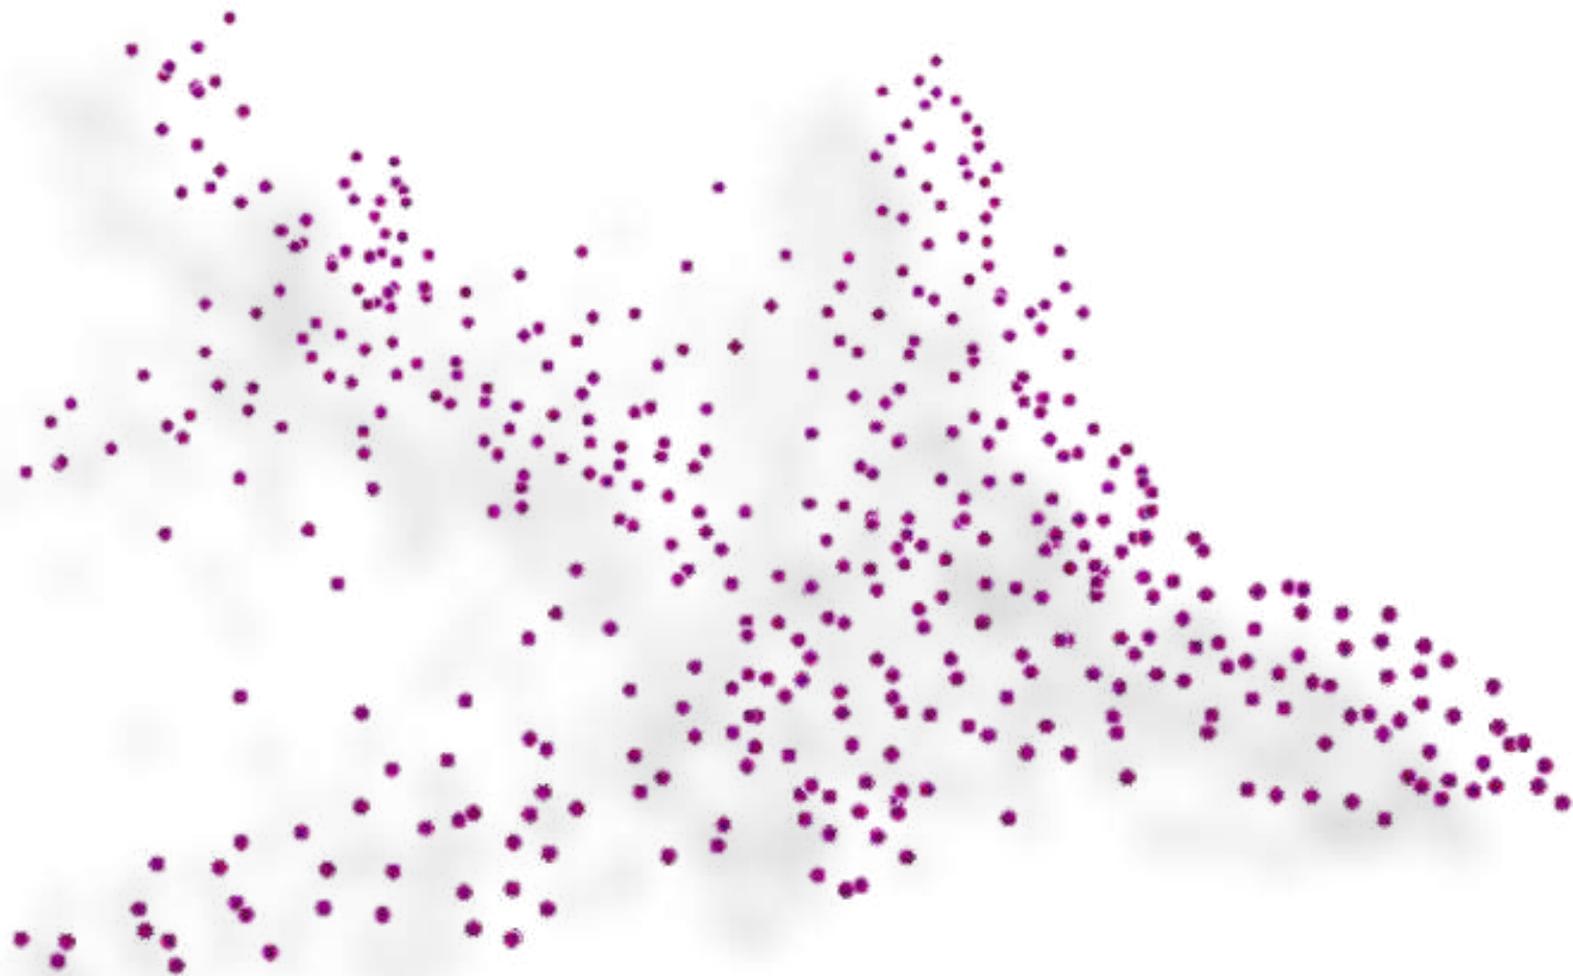

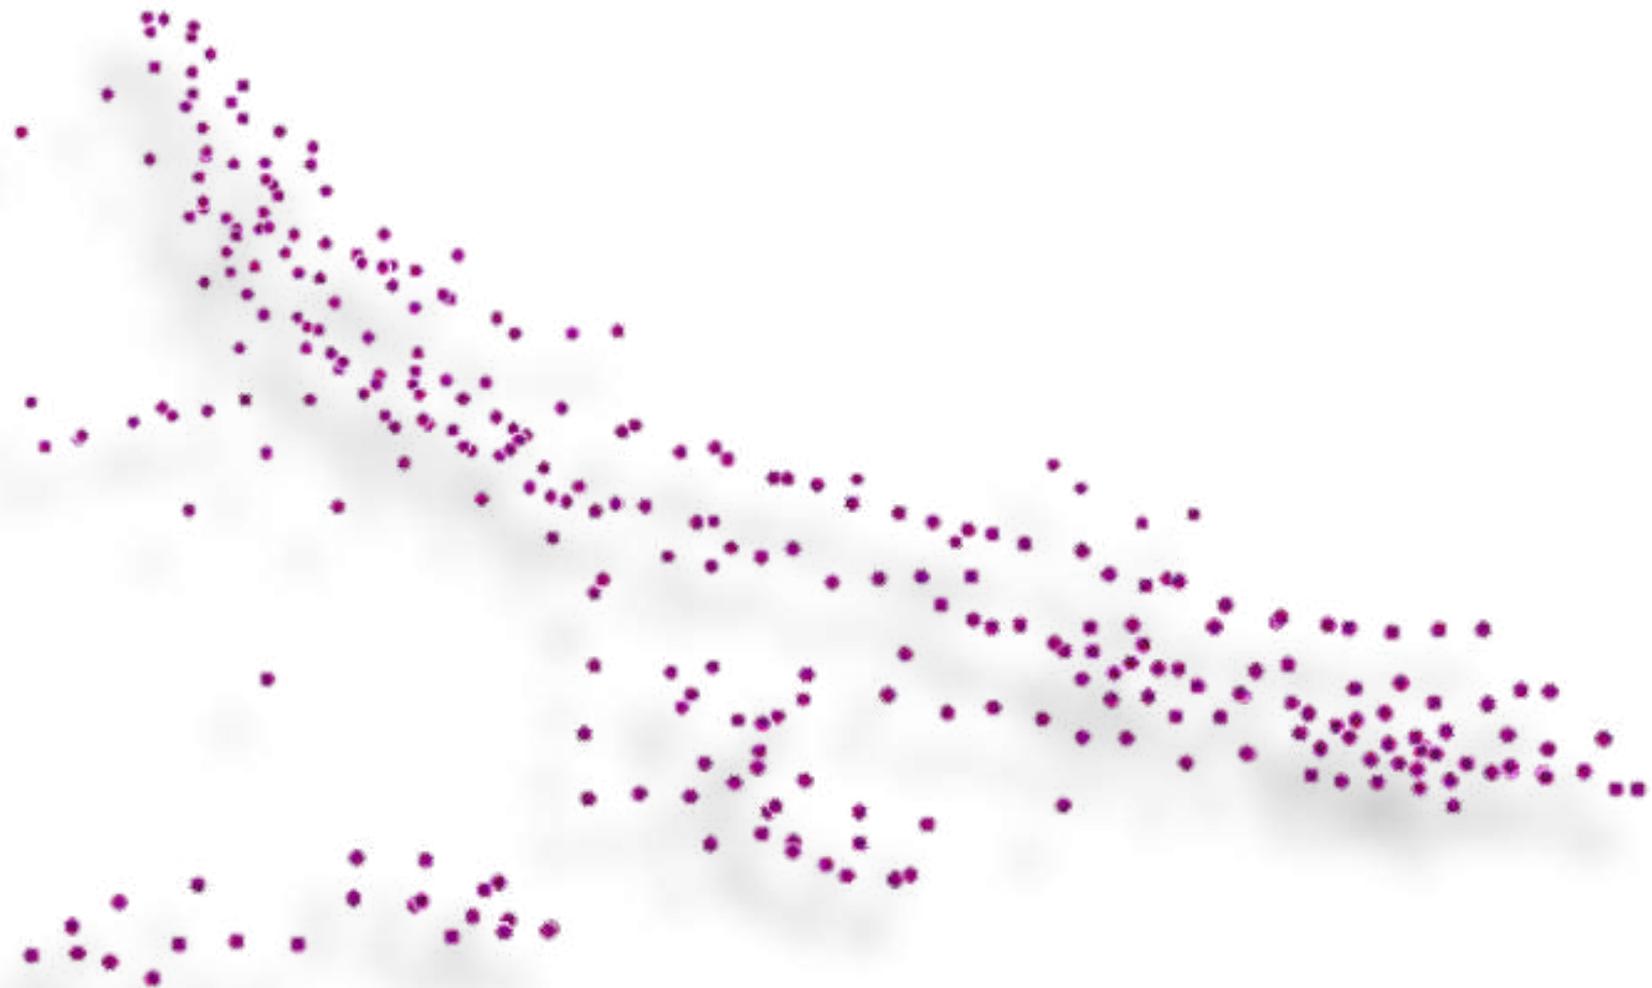

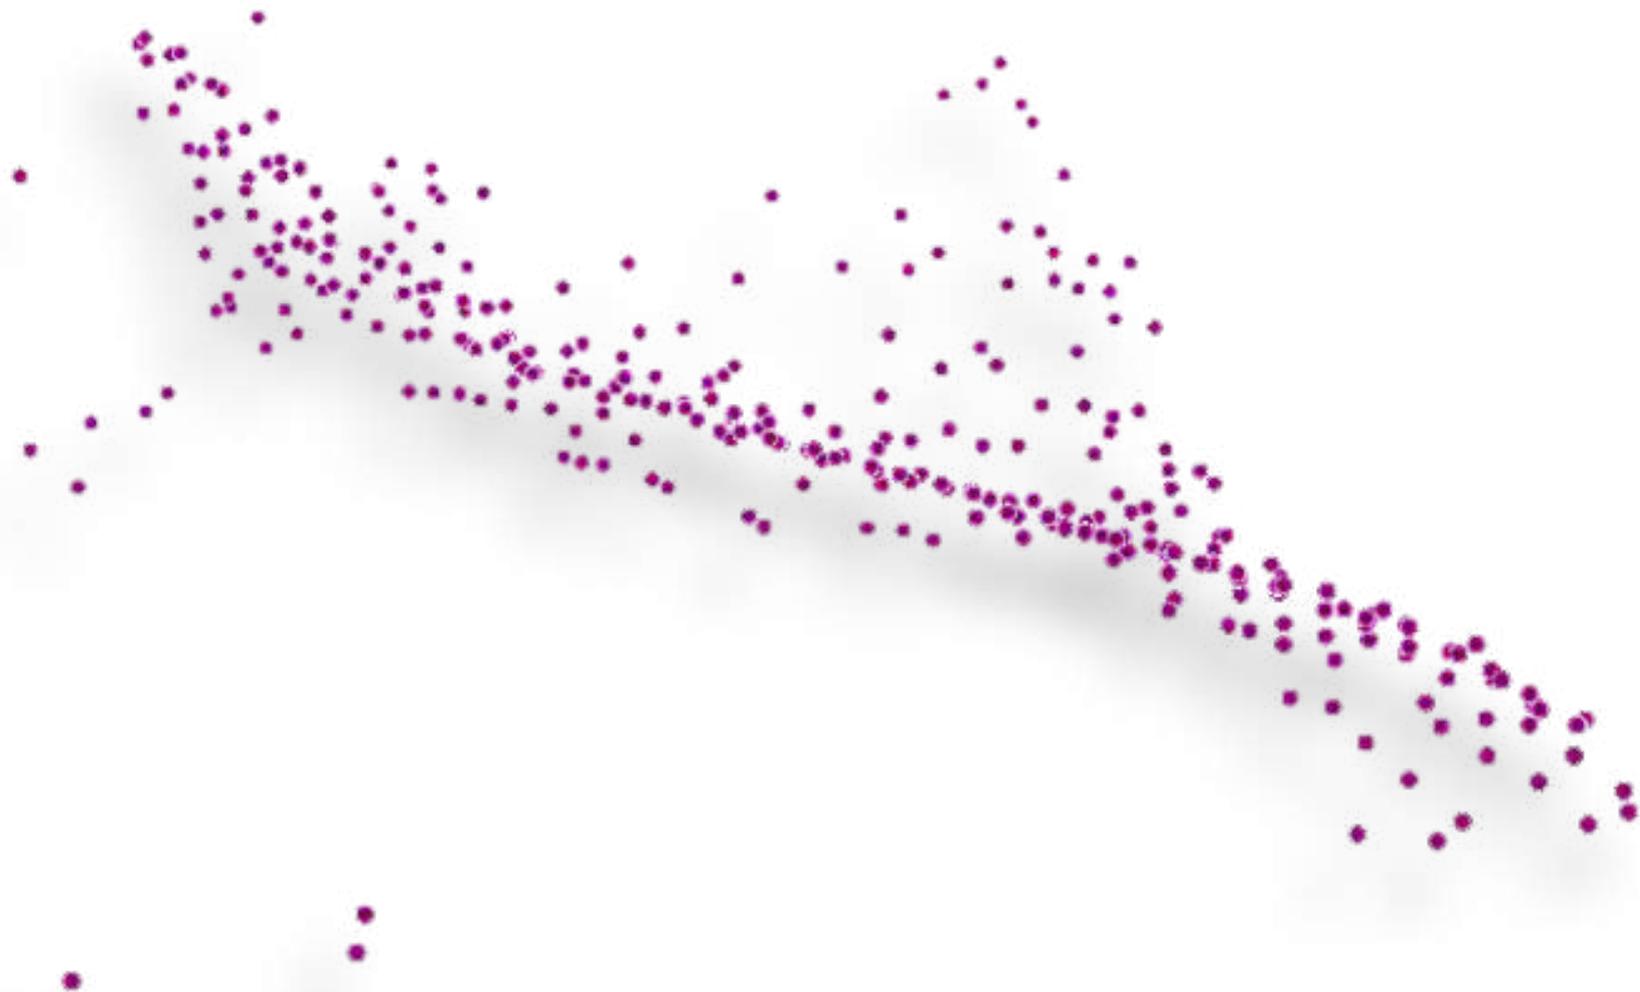

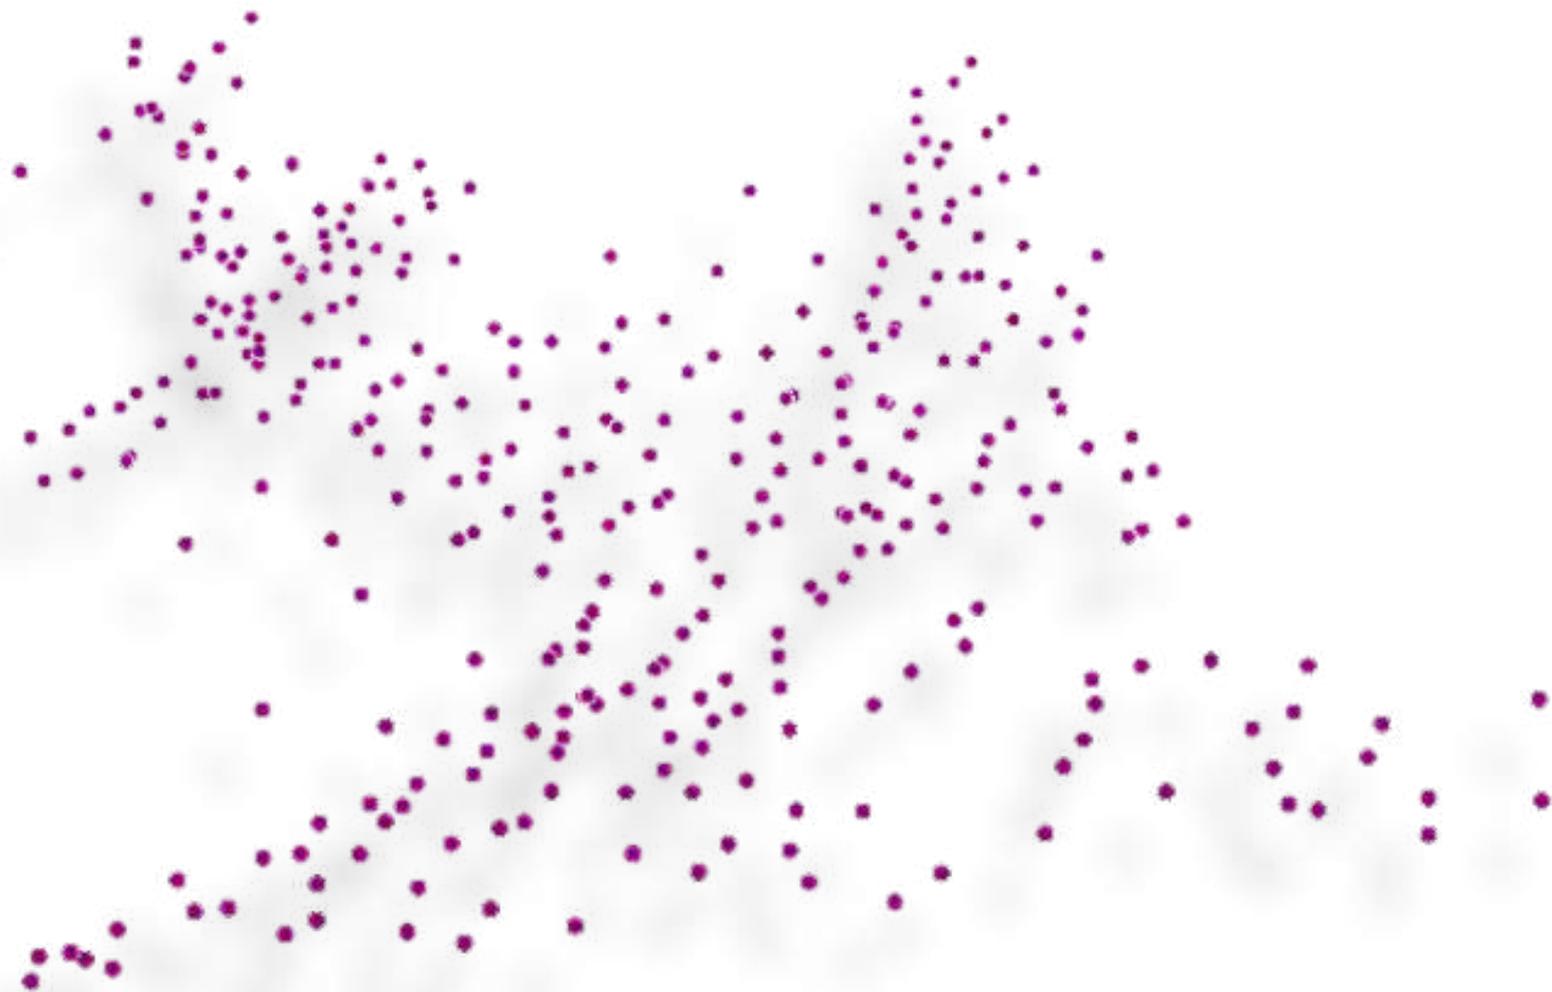

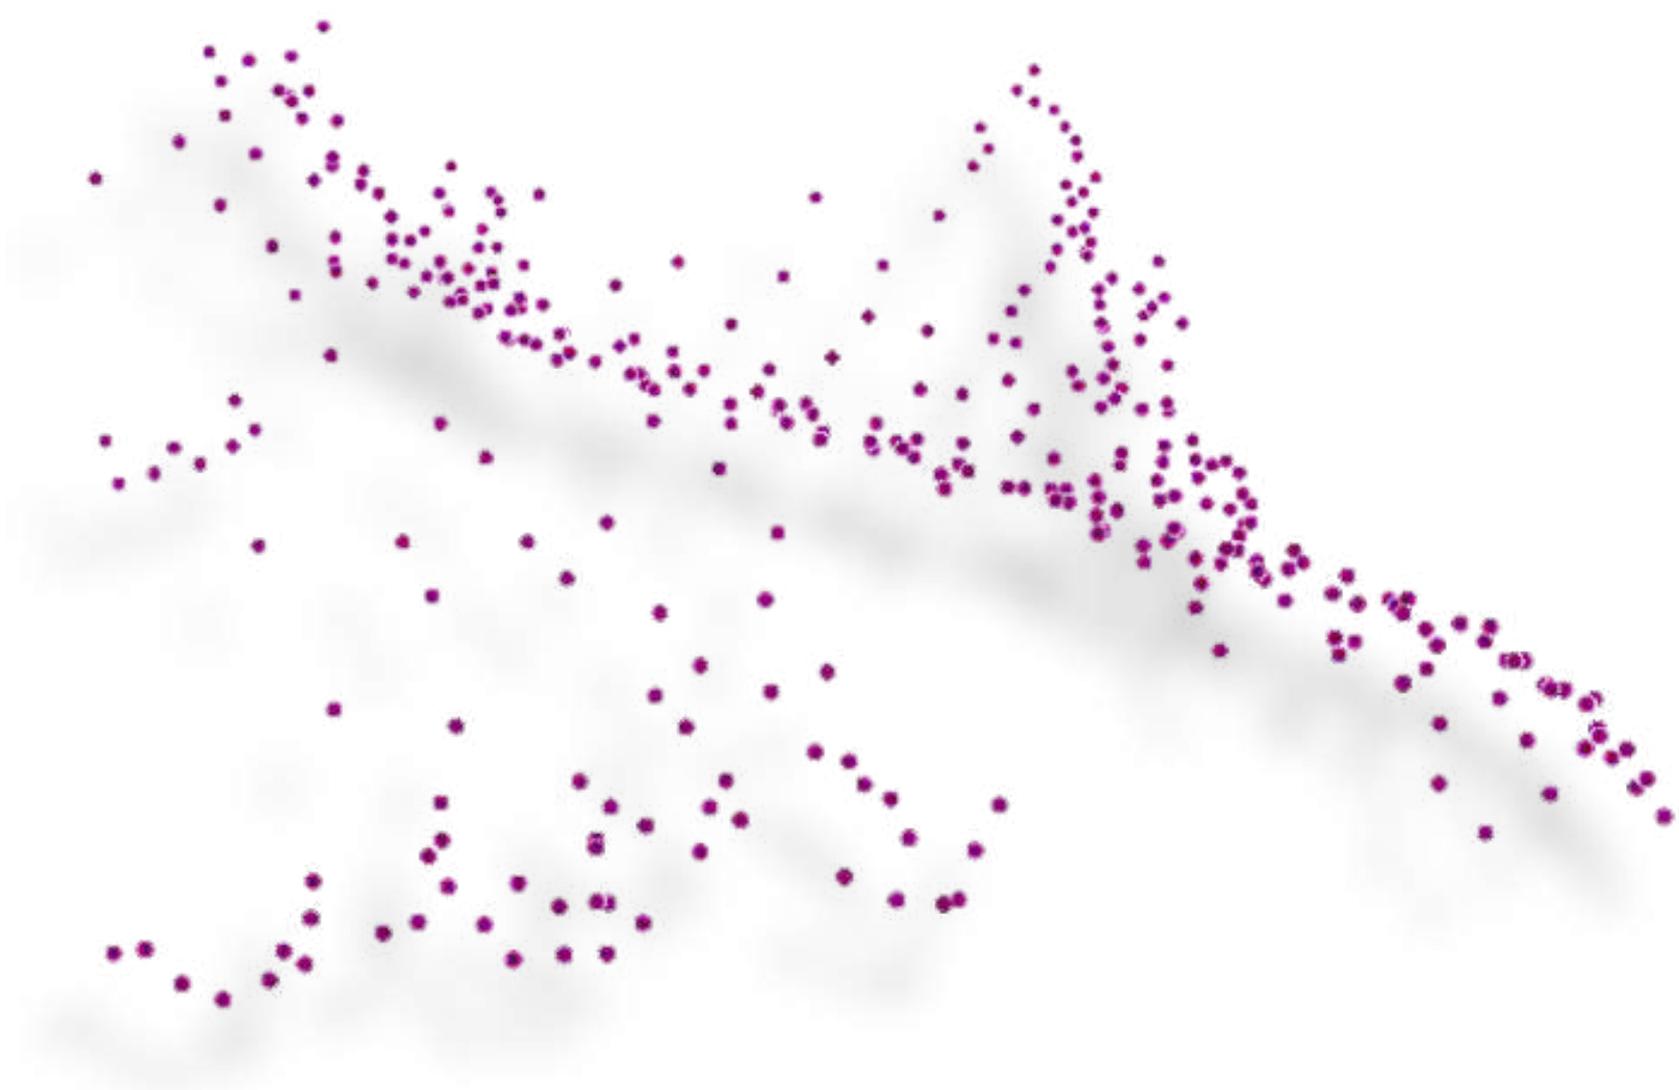

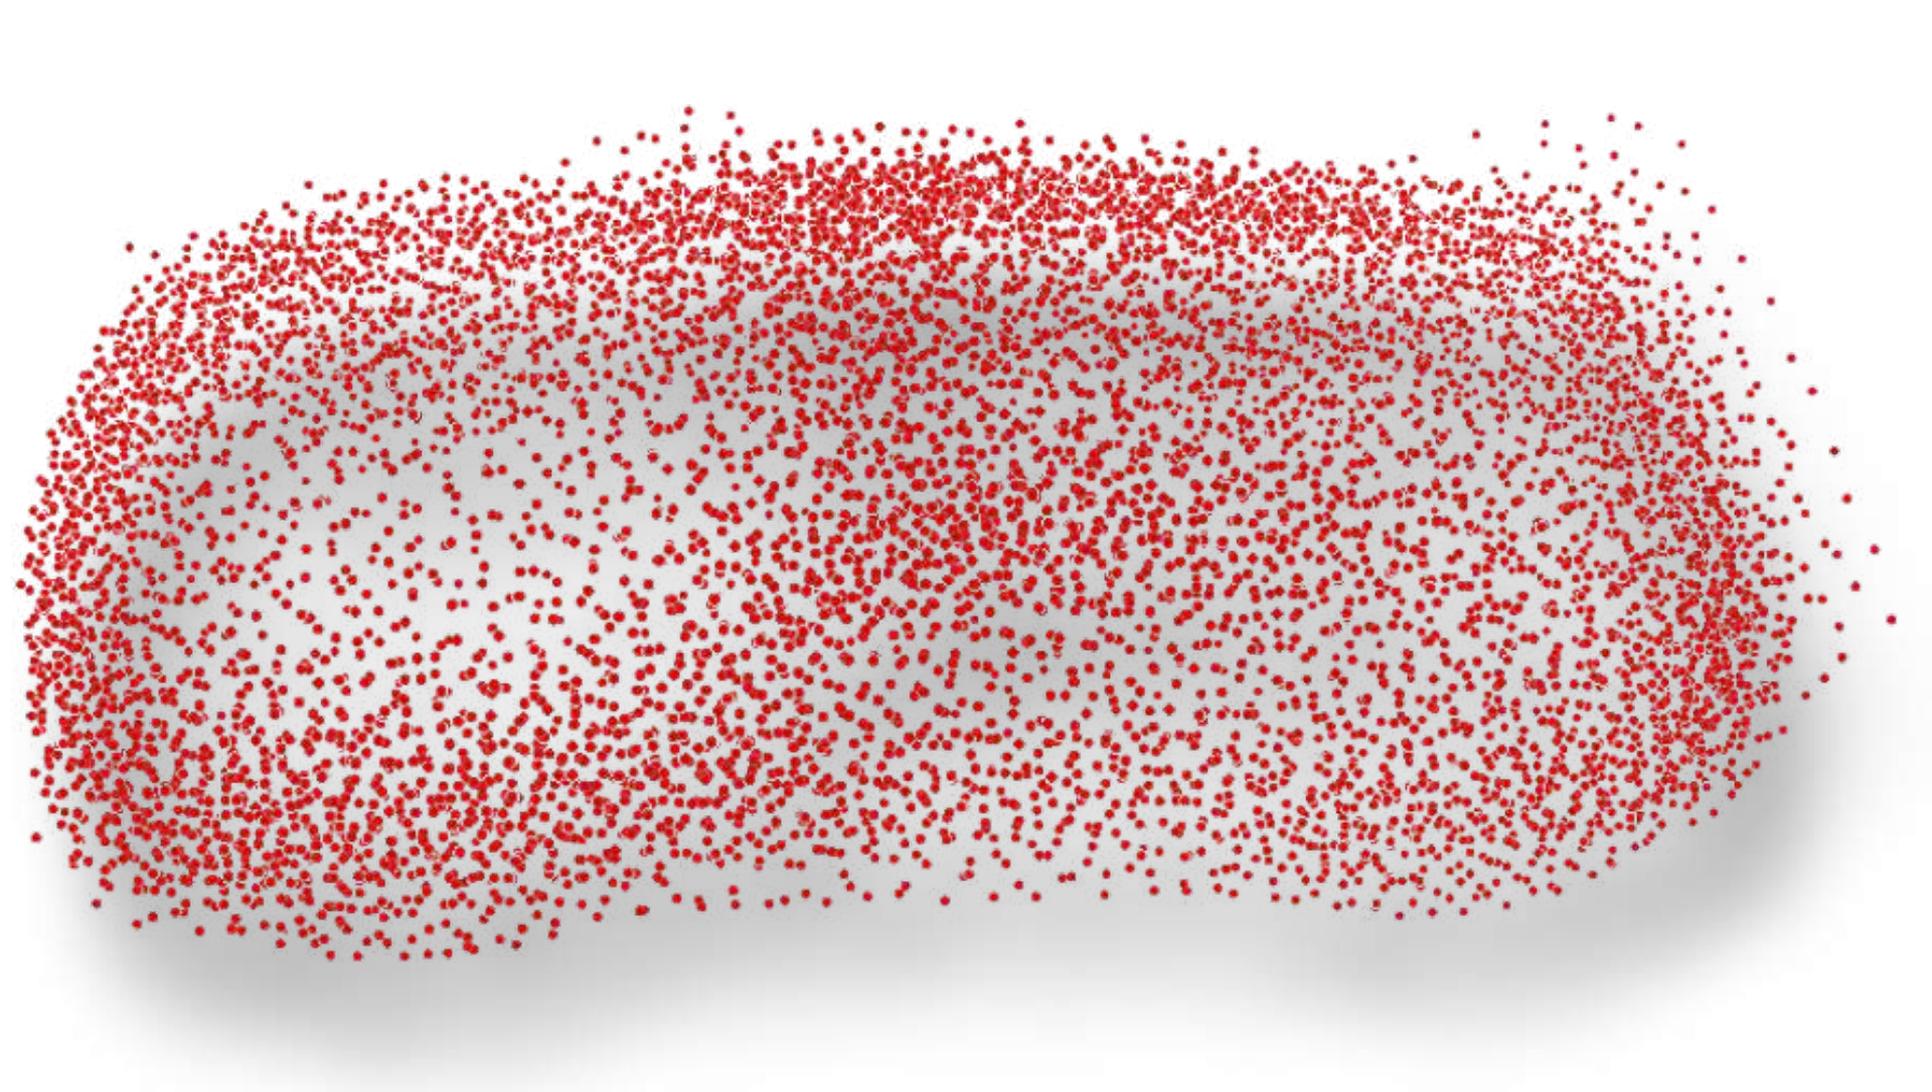

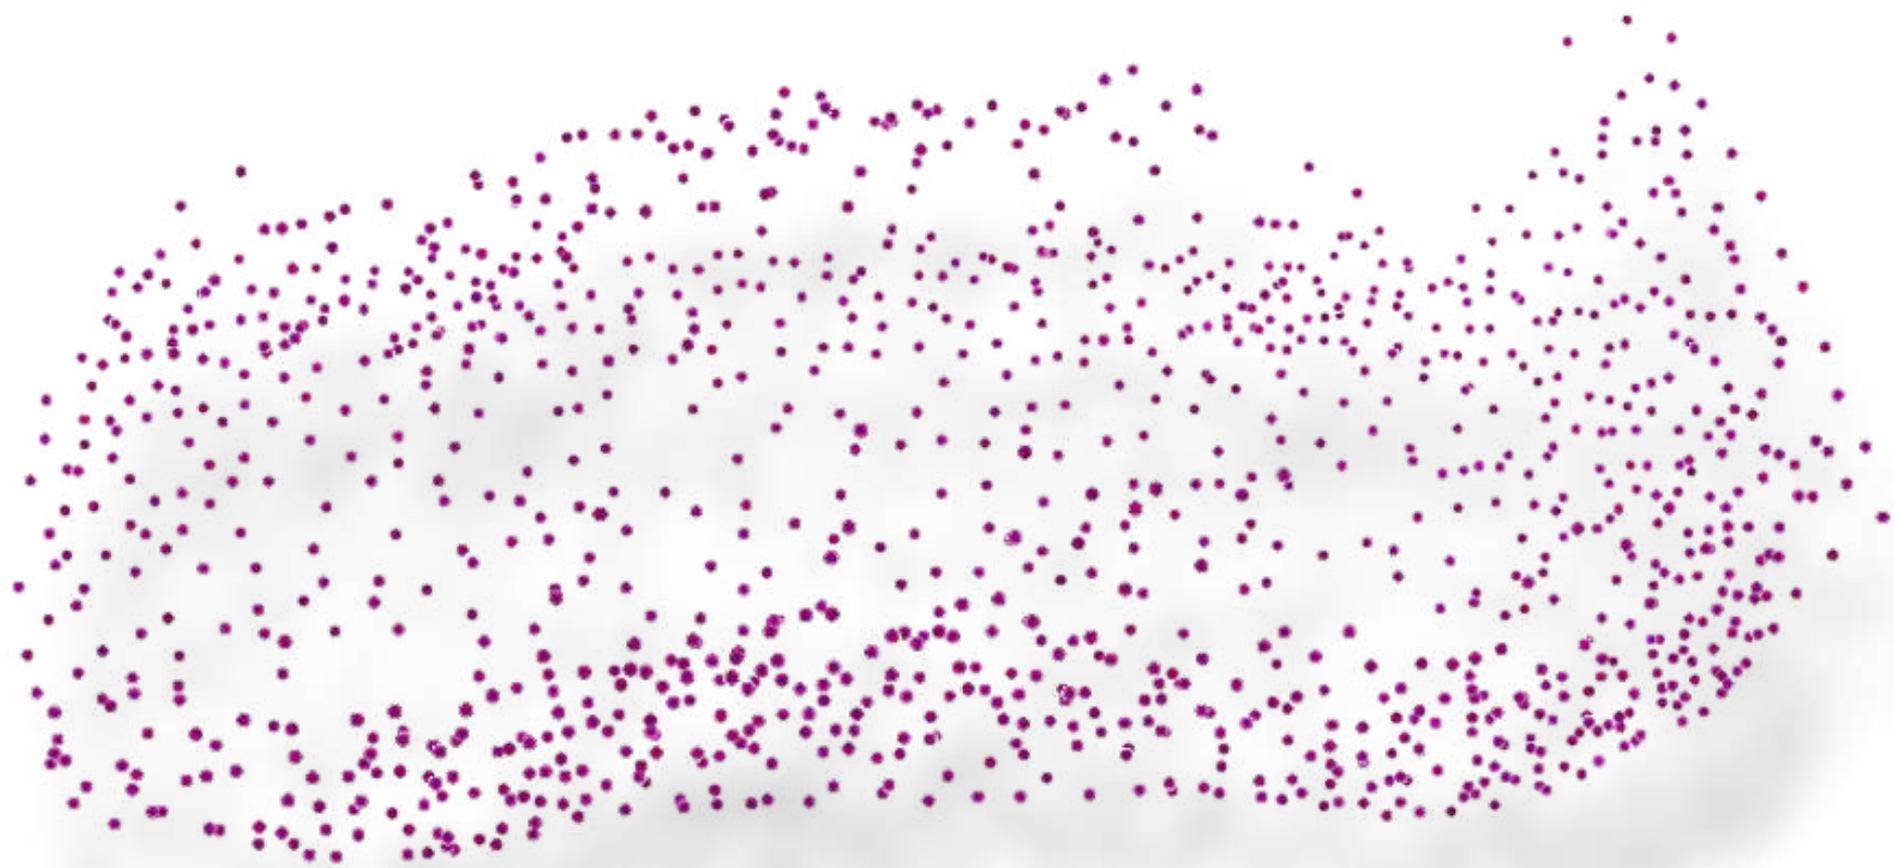

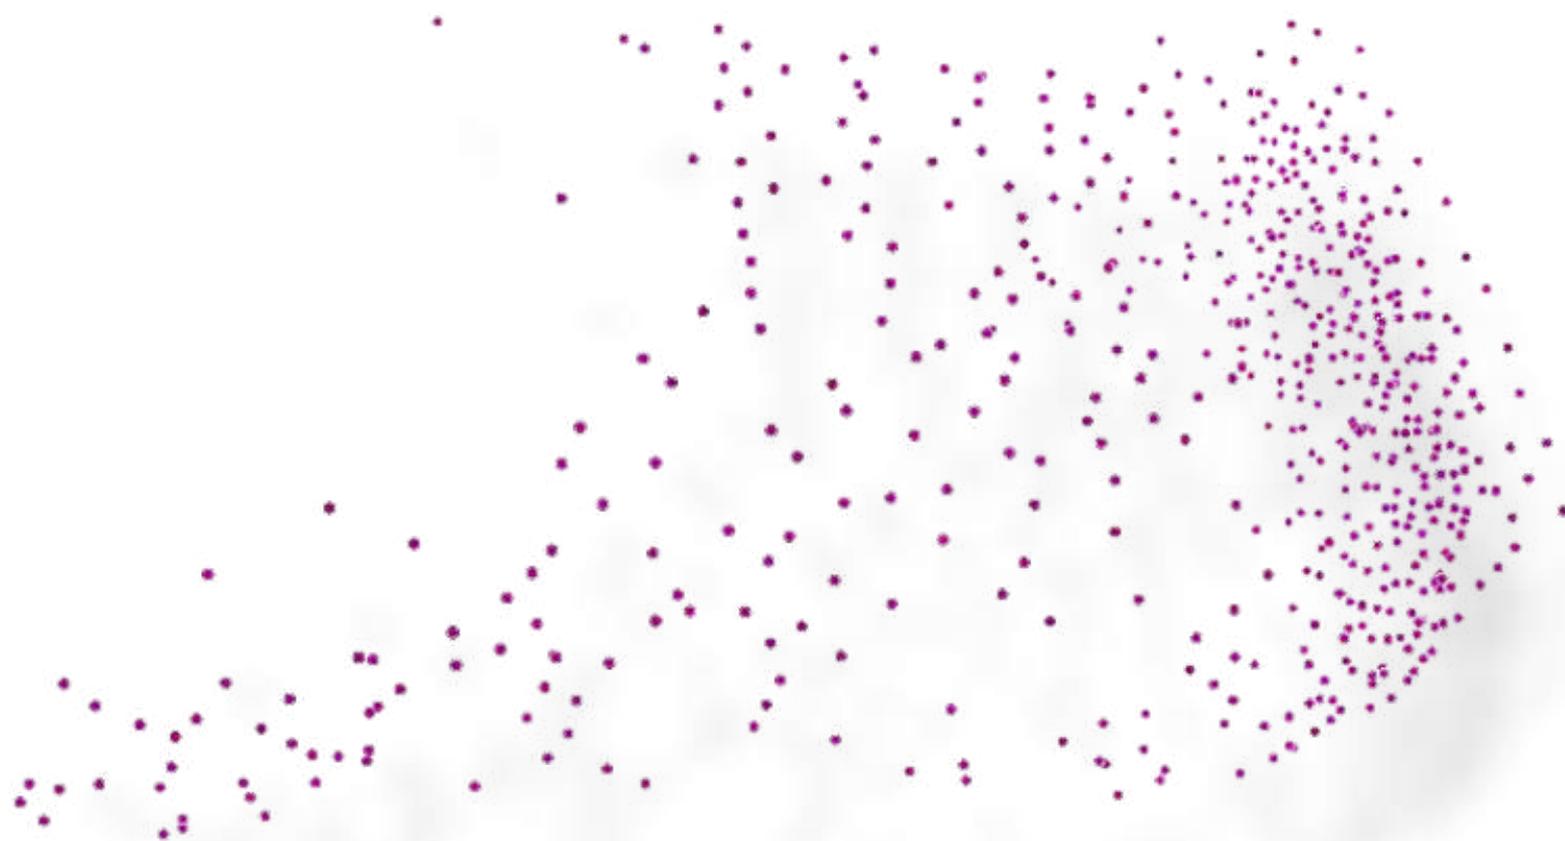

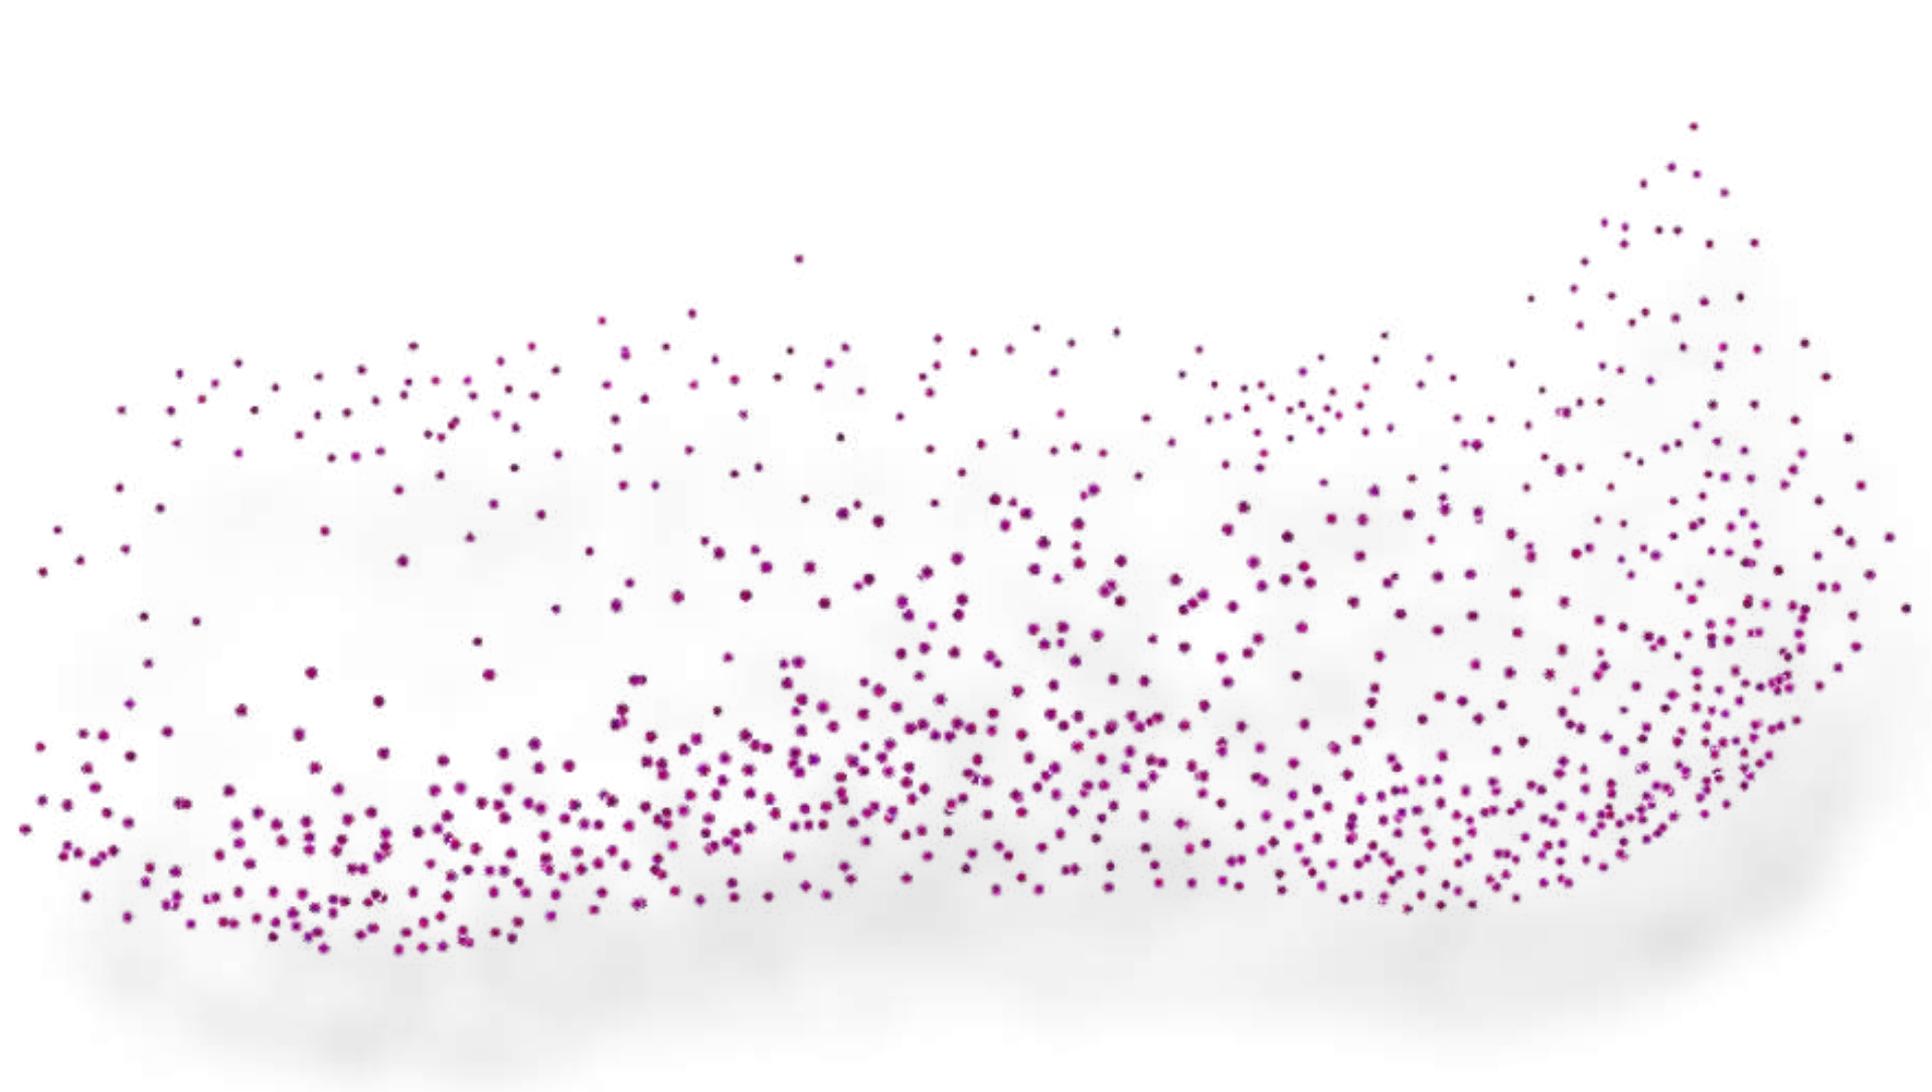

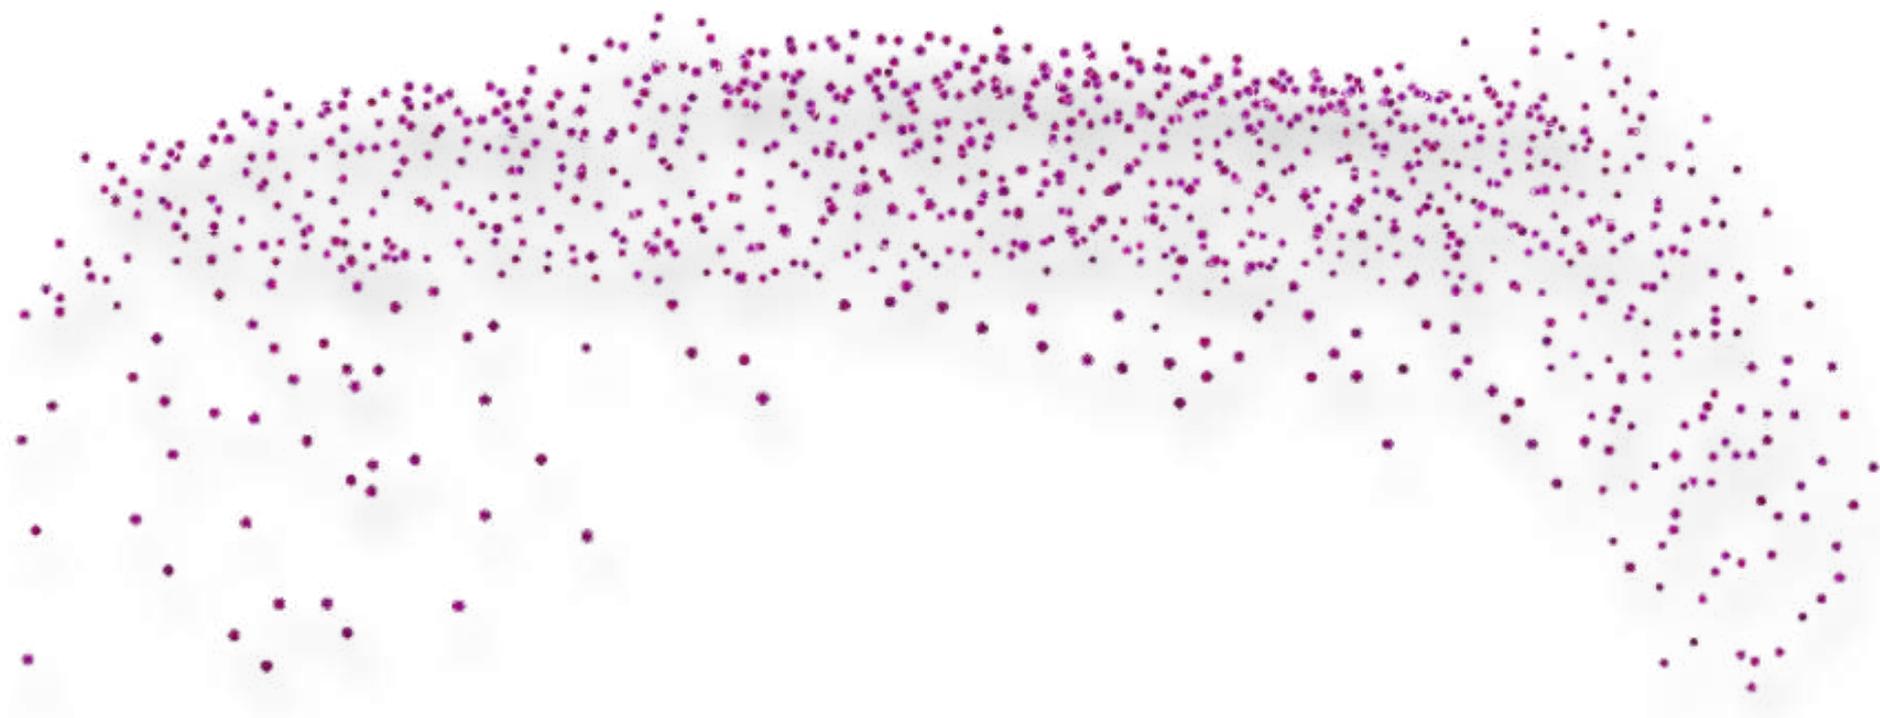

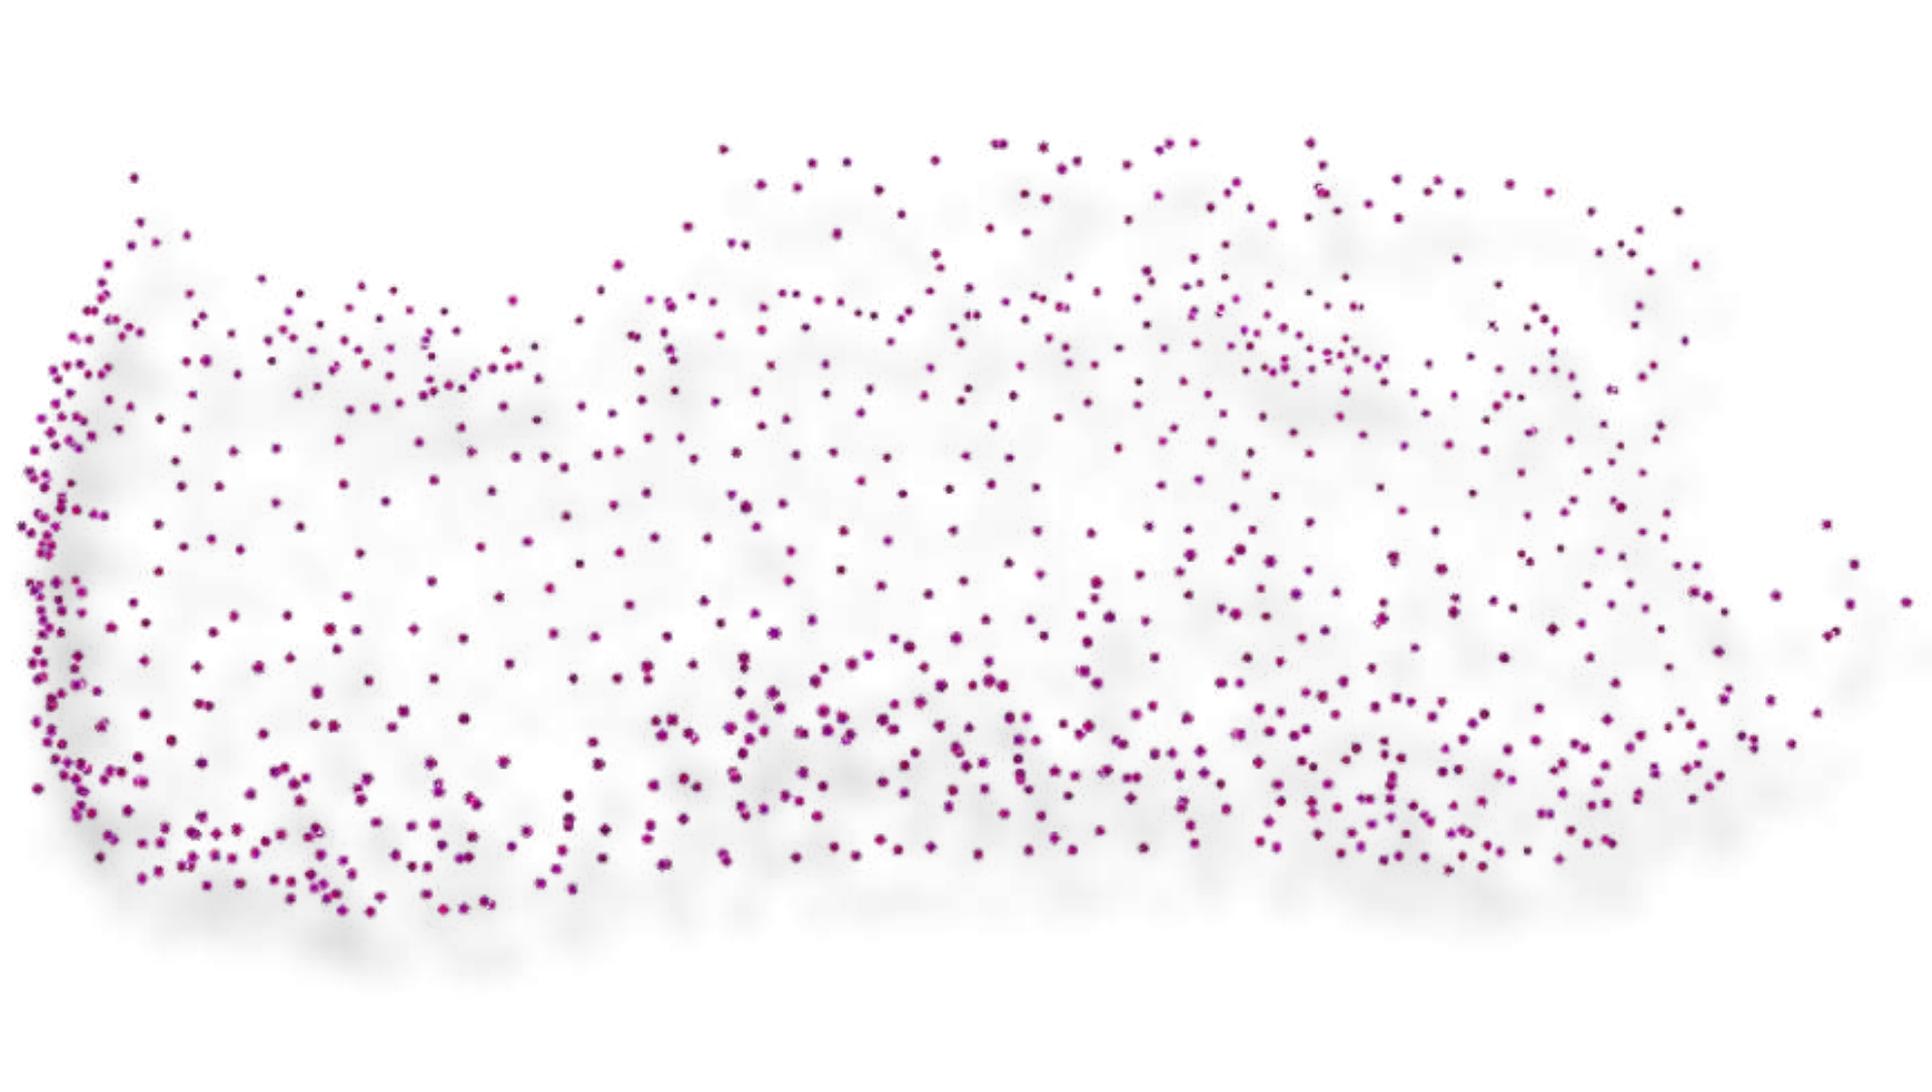

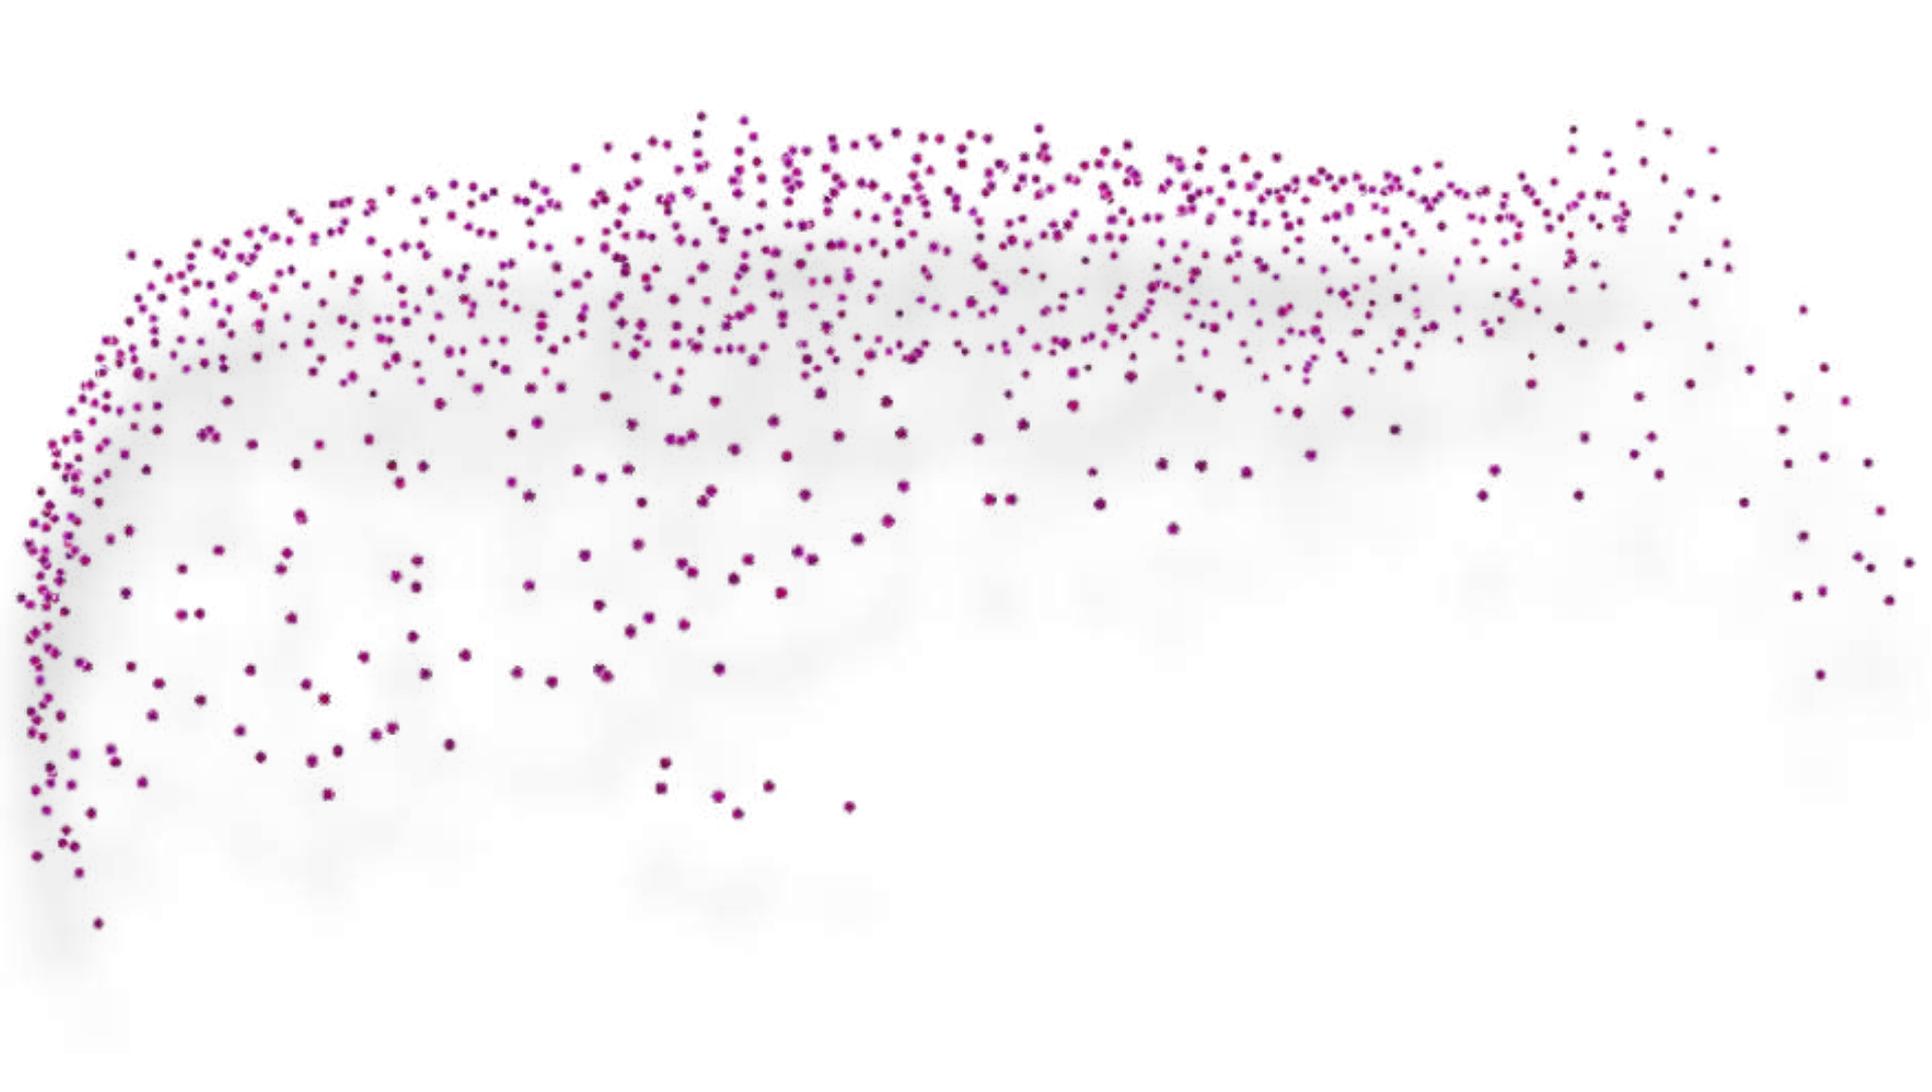

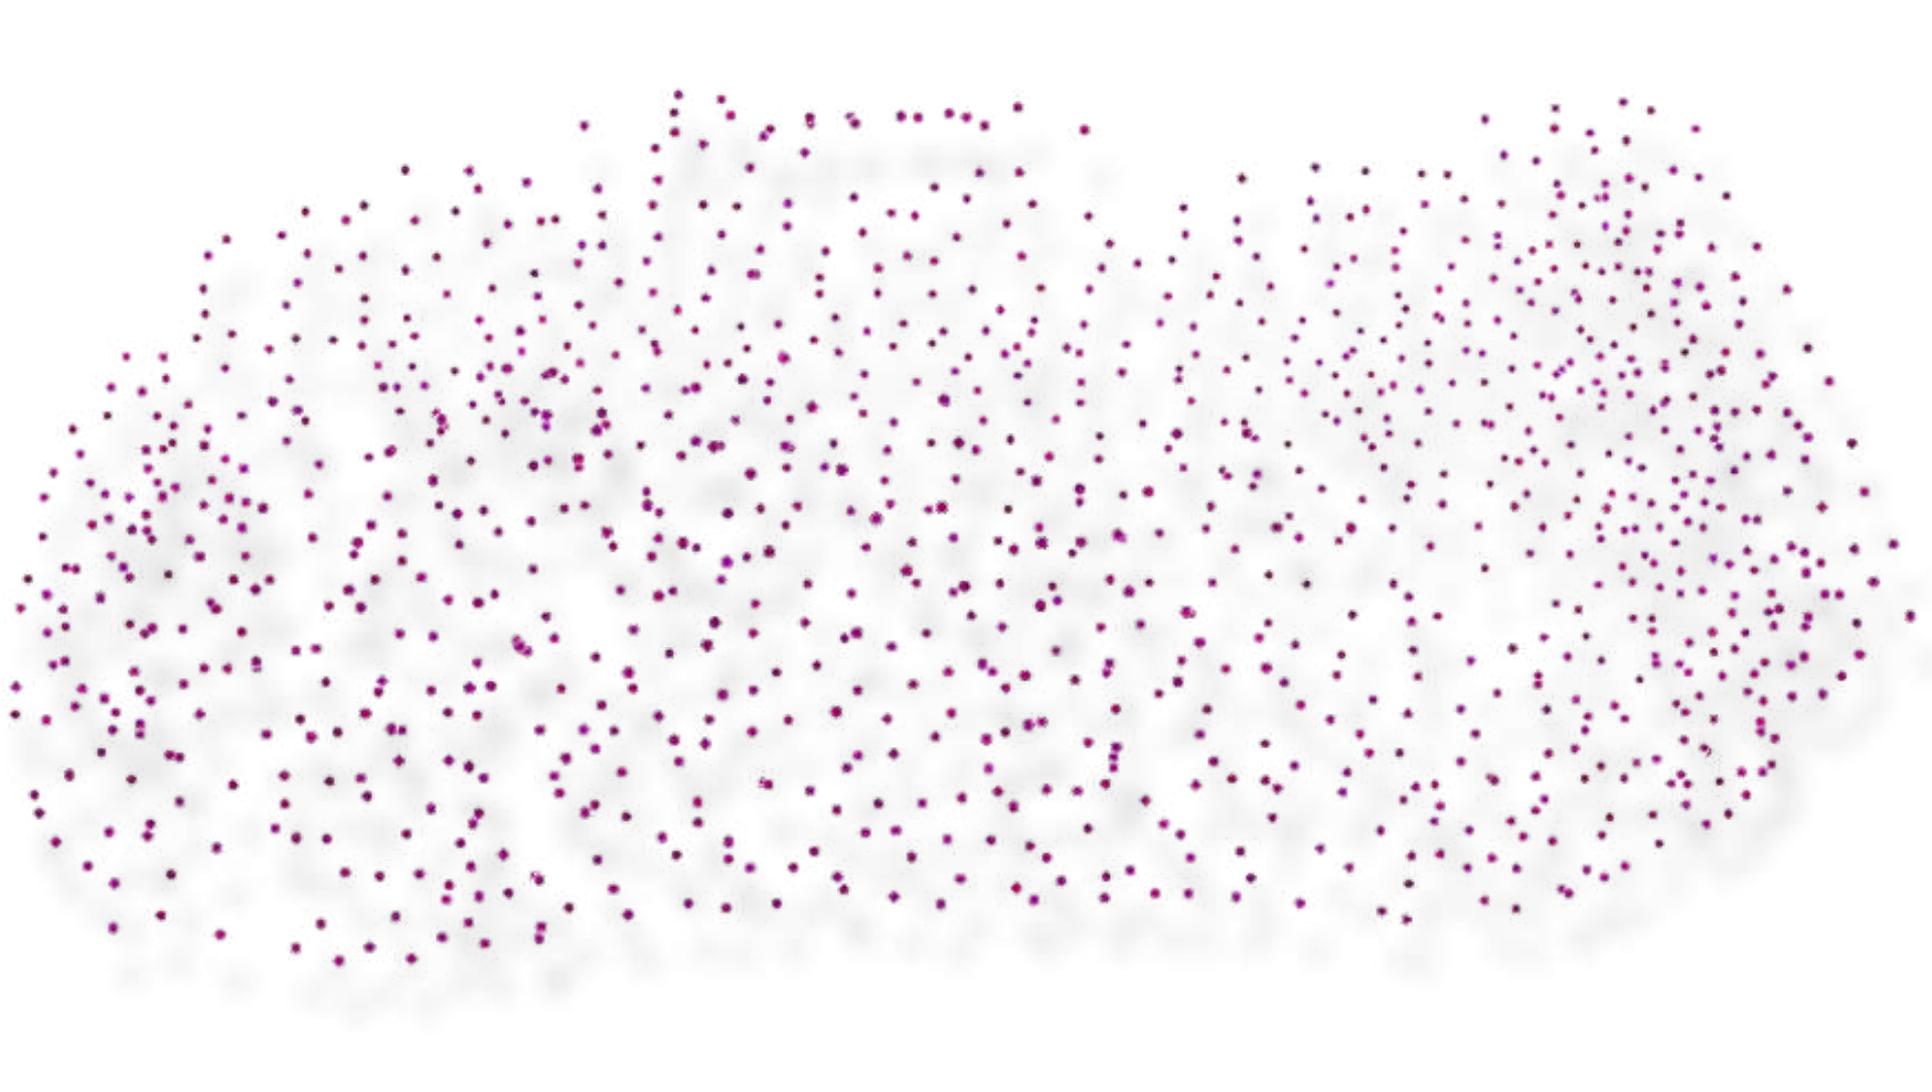

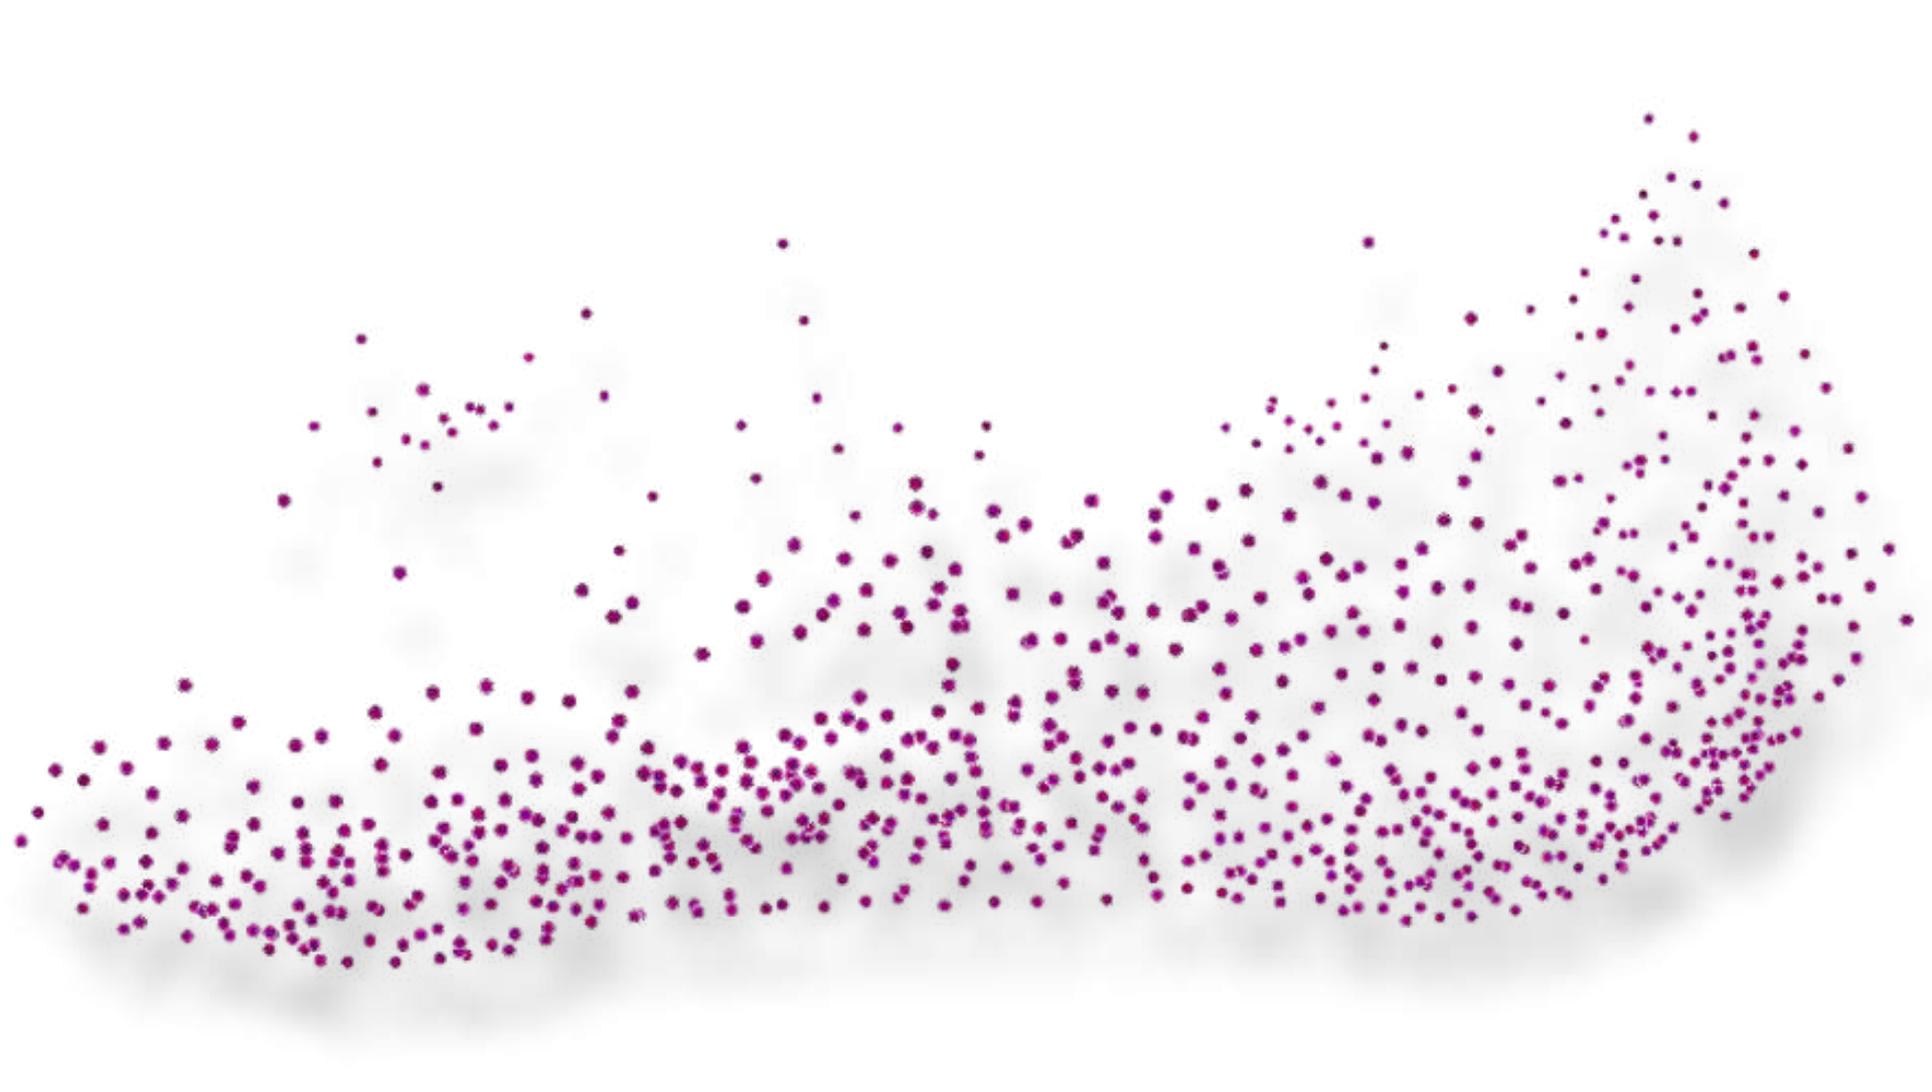

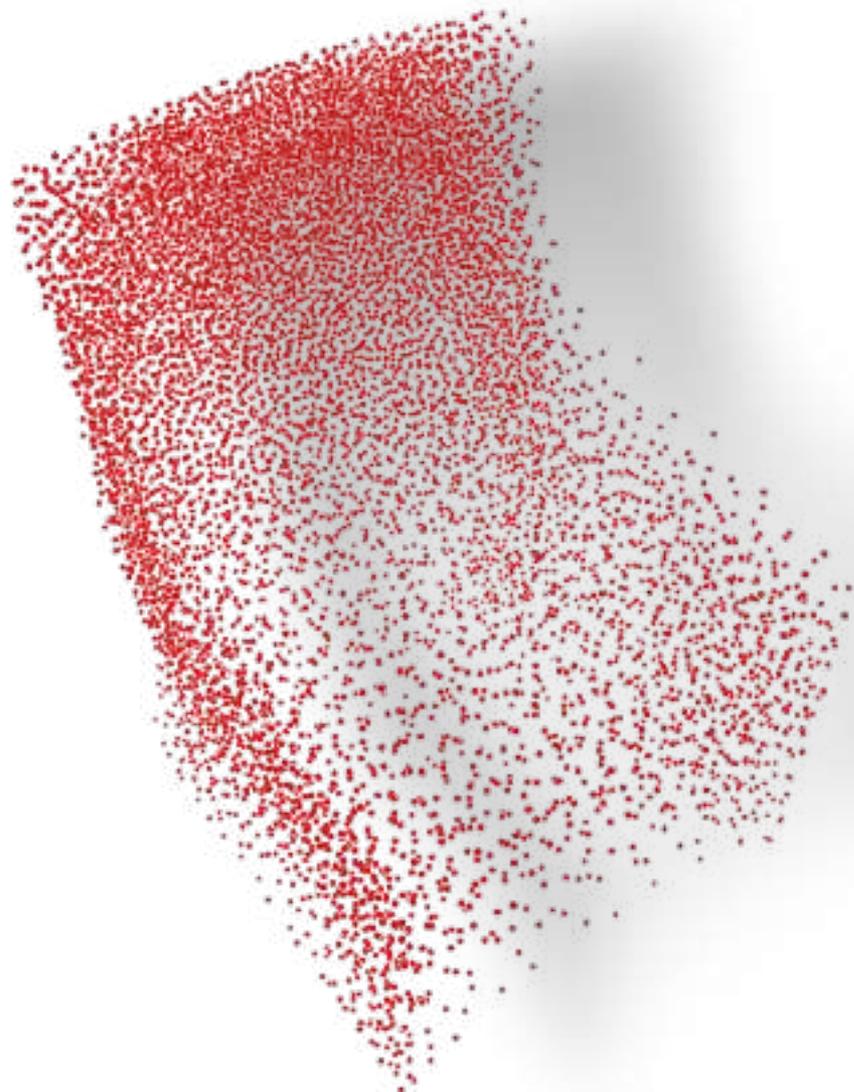

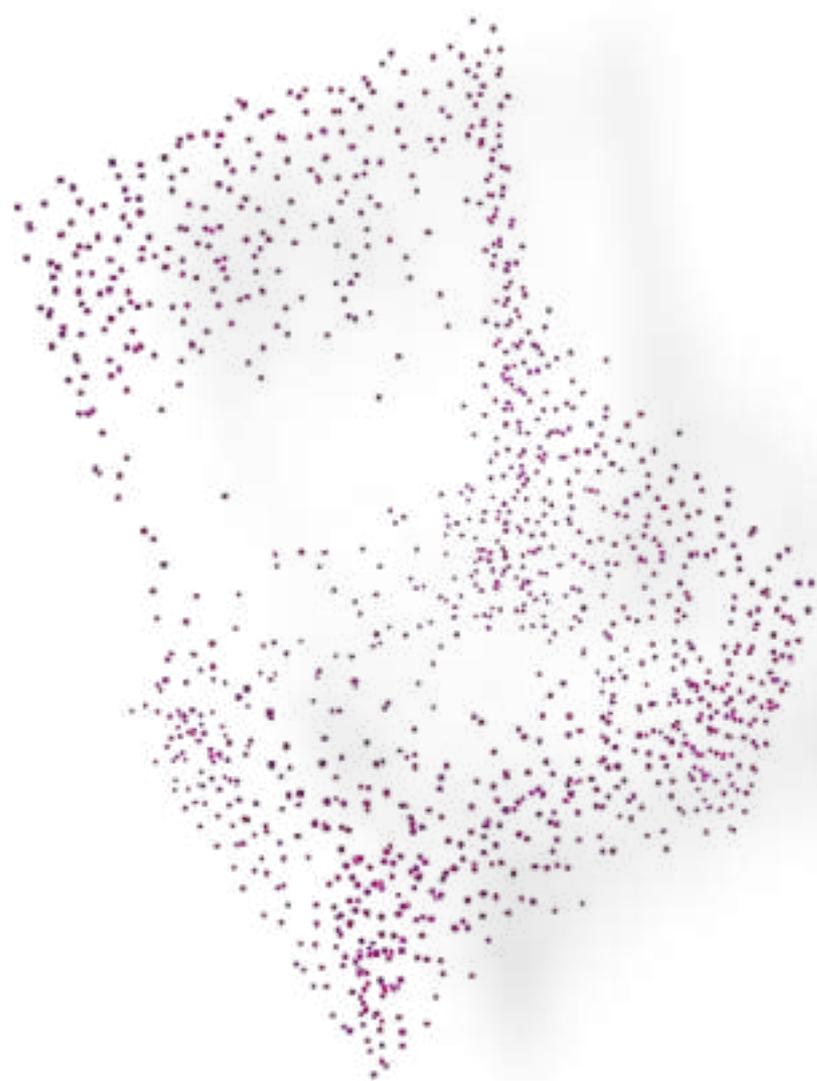

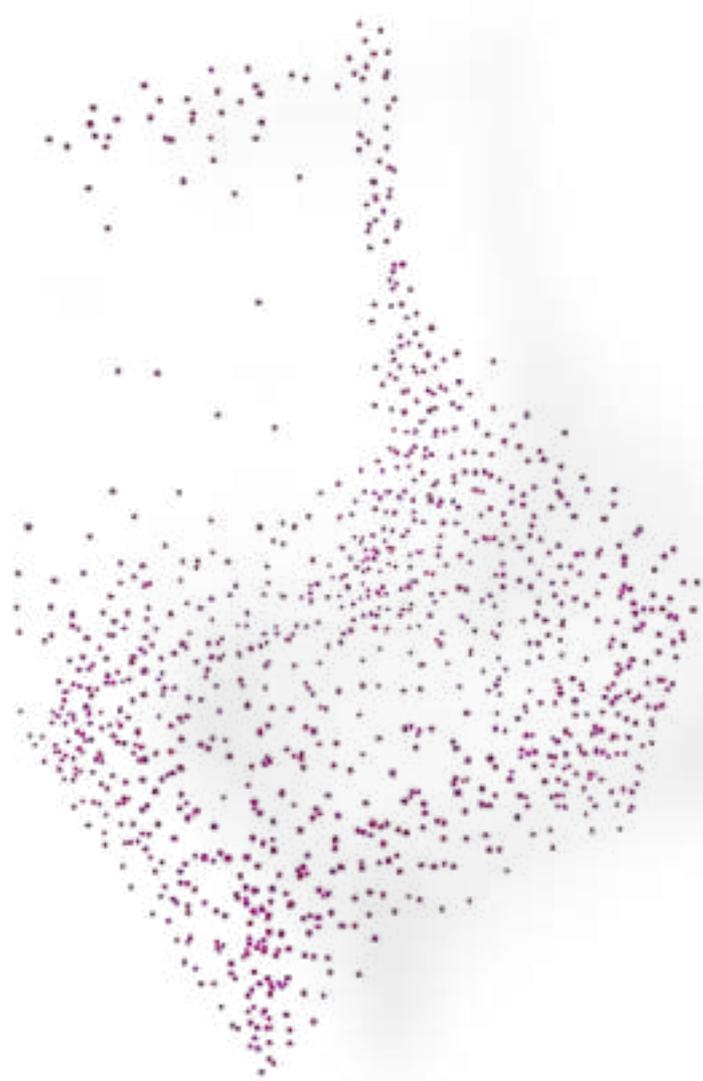

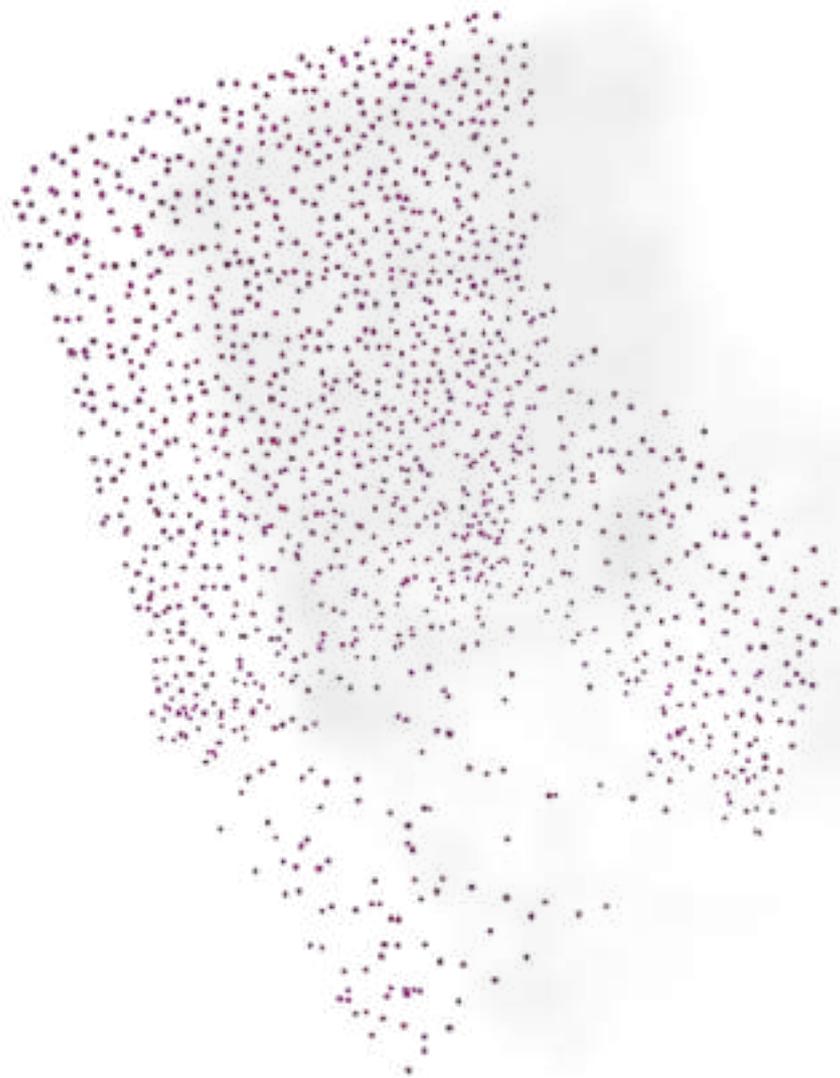

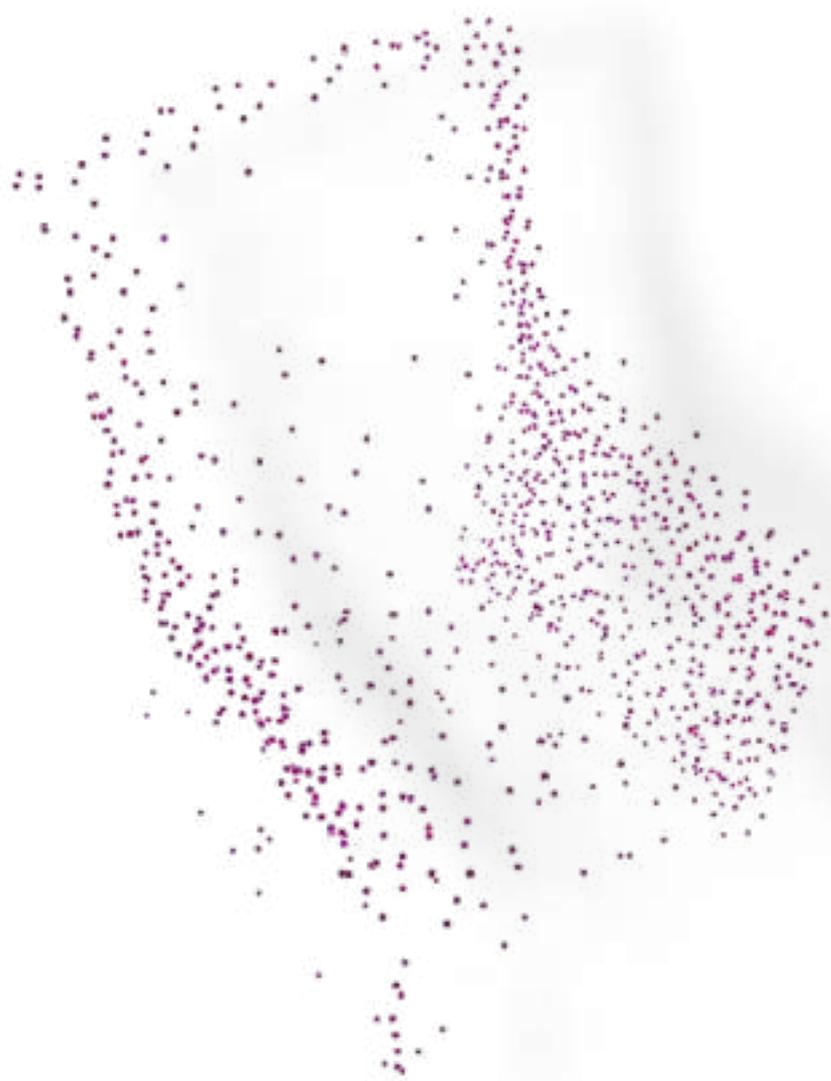

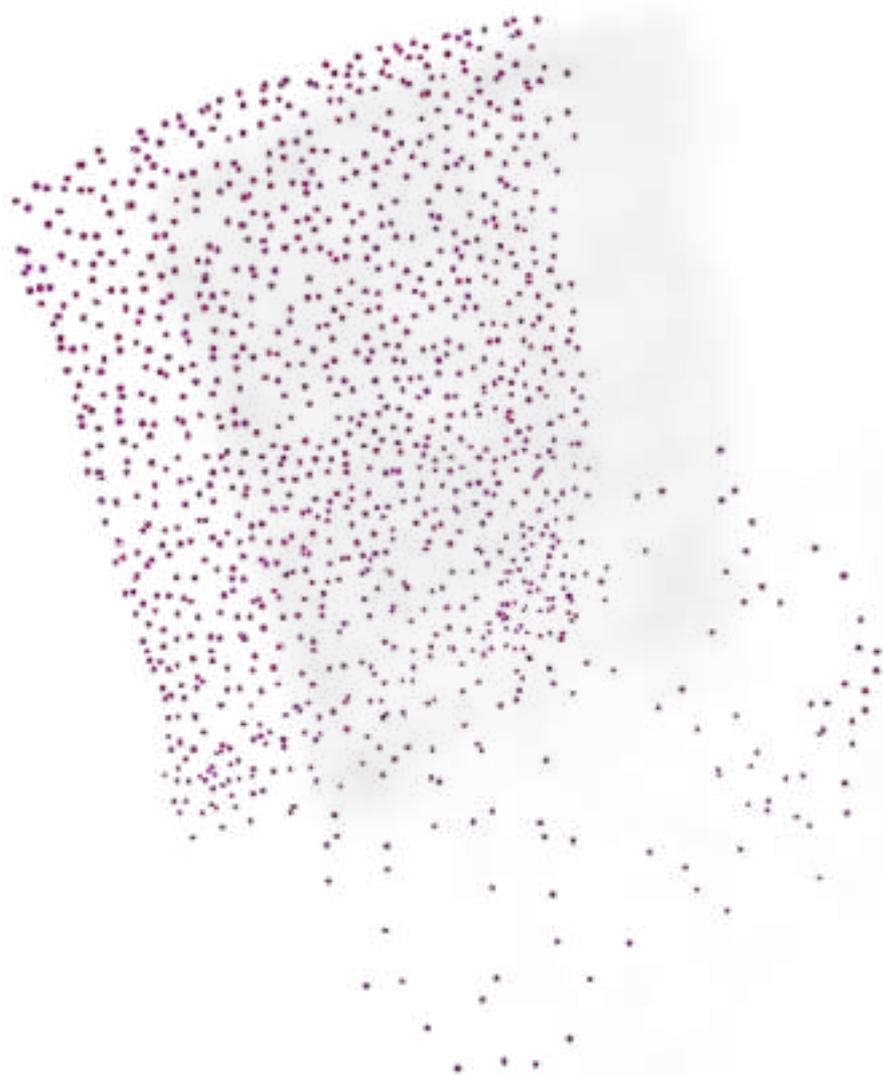

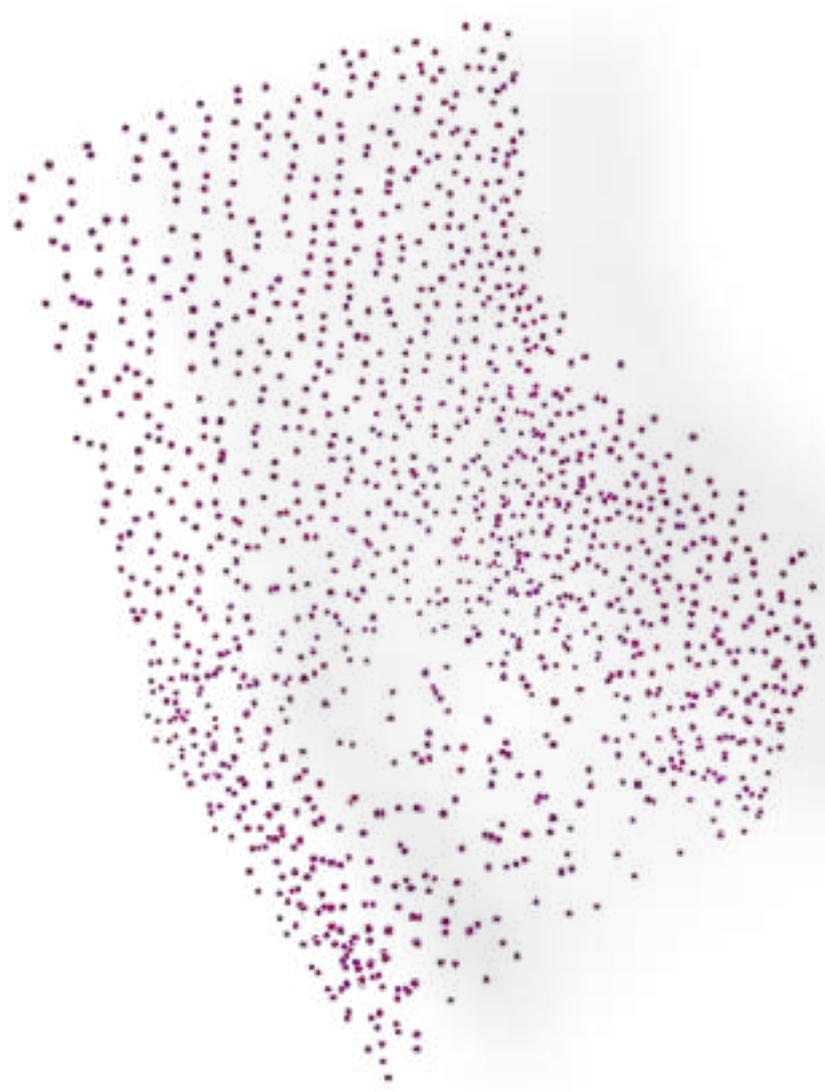

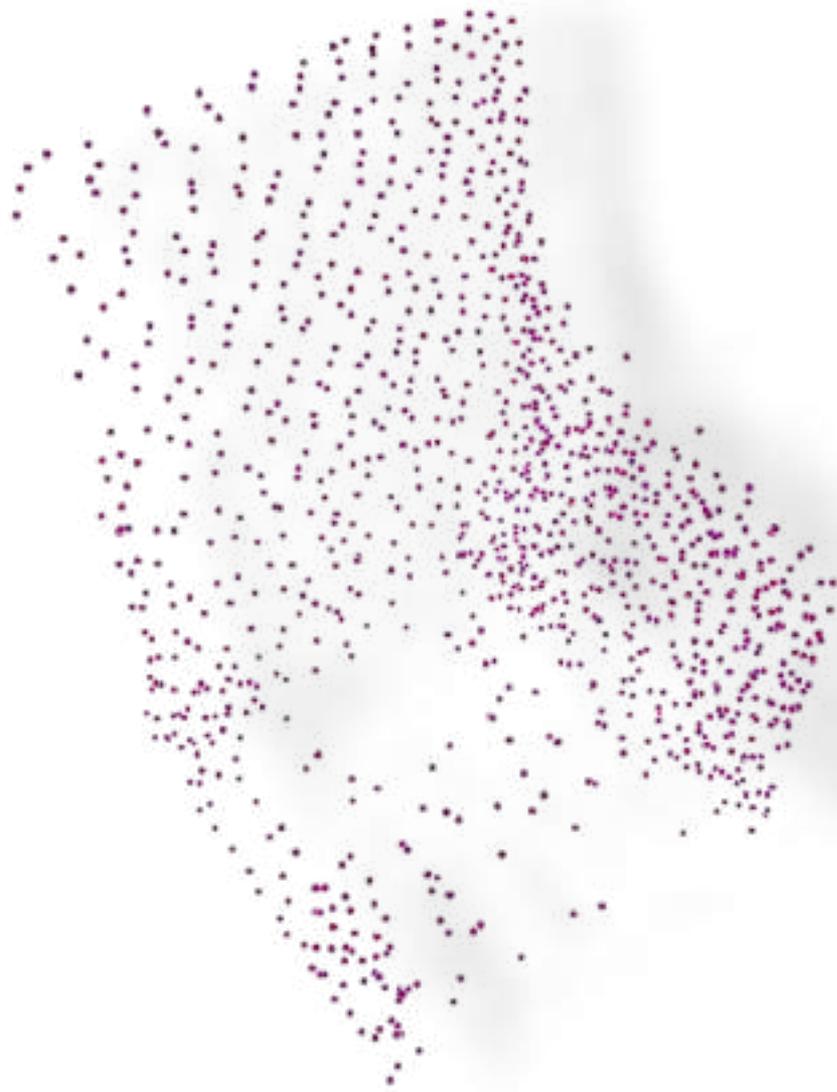

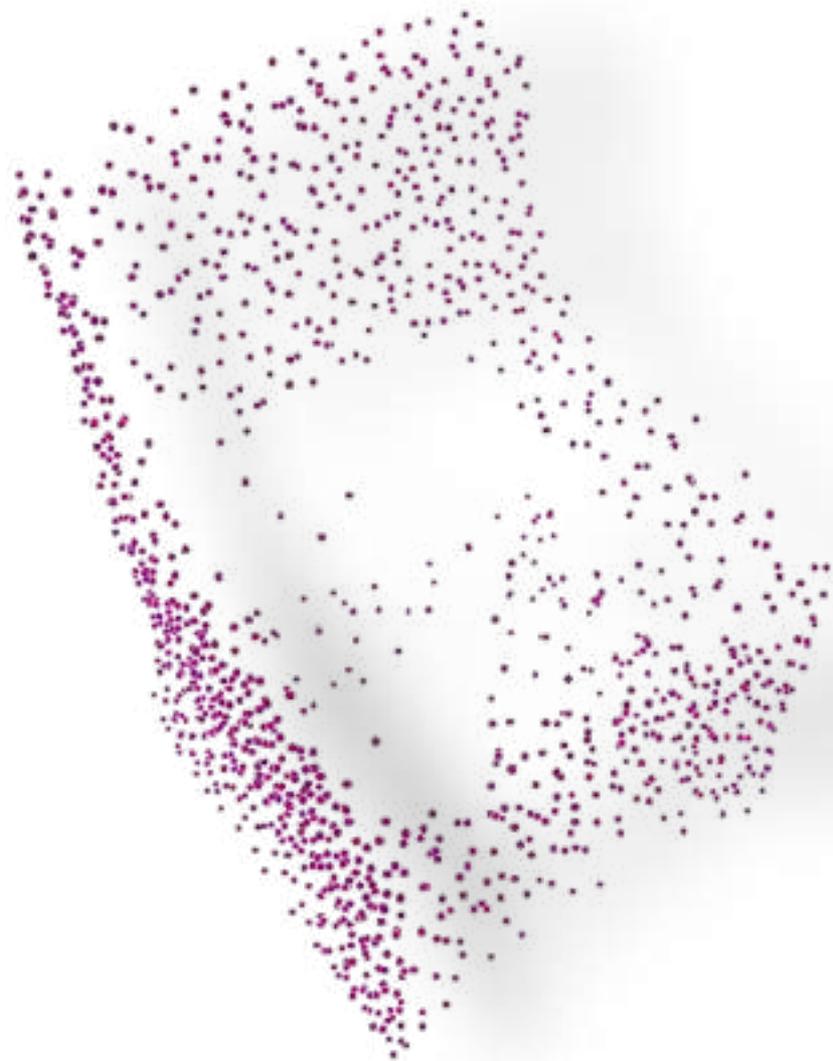

Supplement: Supplementary file 7 [file supp_syn.pdf]
