# Supplementary material for: ACL-SPC: Adaptive Closed-Loop system for Self-Supervised Point Cloud Completion
Source: arXiv:2303.01979 source file (2023-03-28)

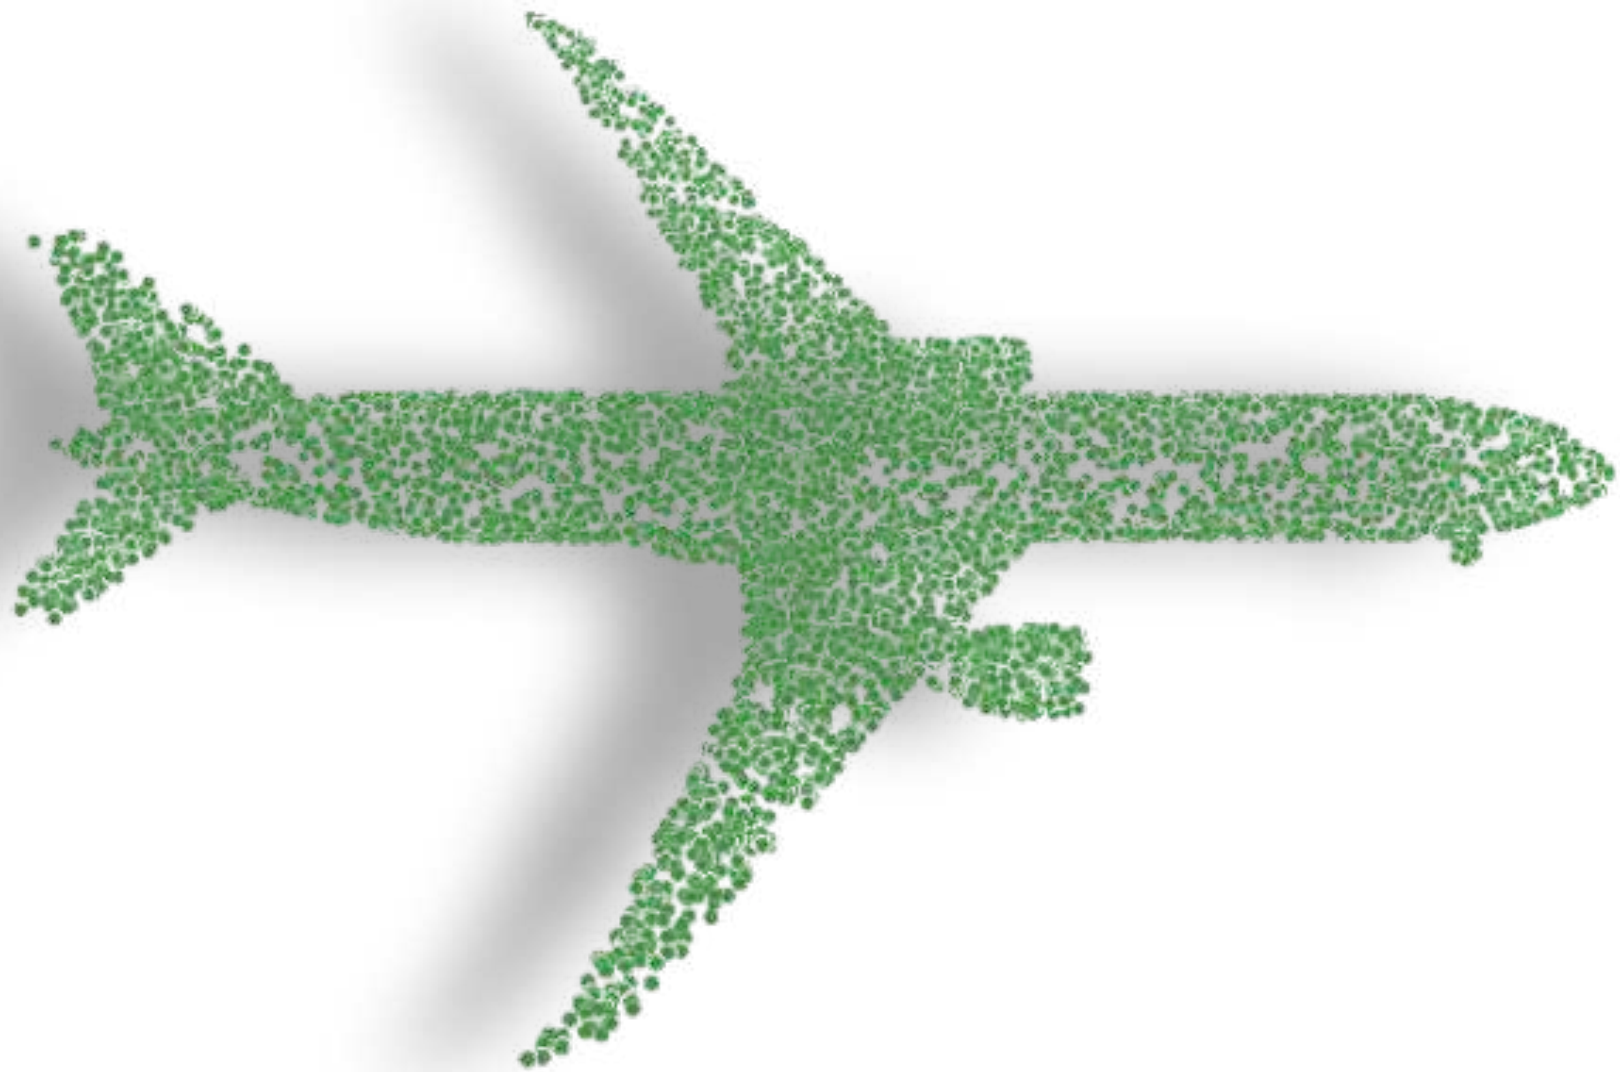

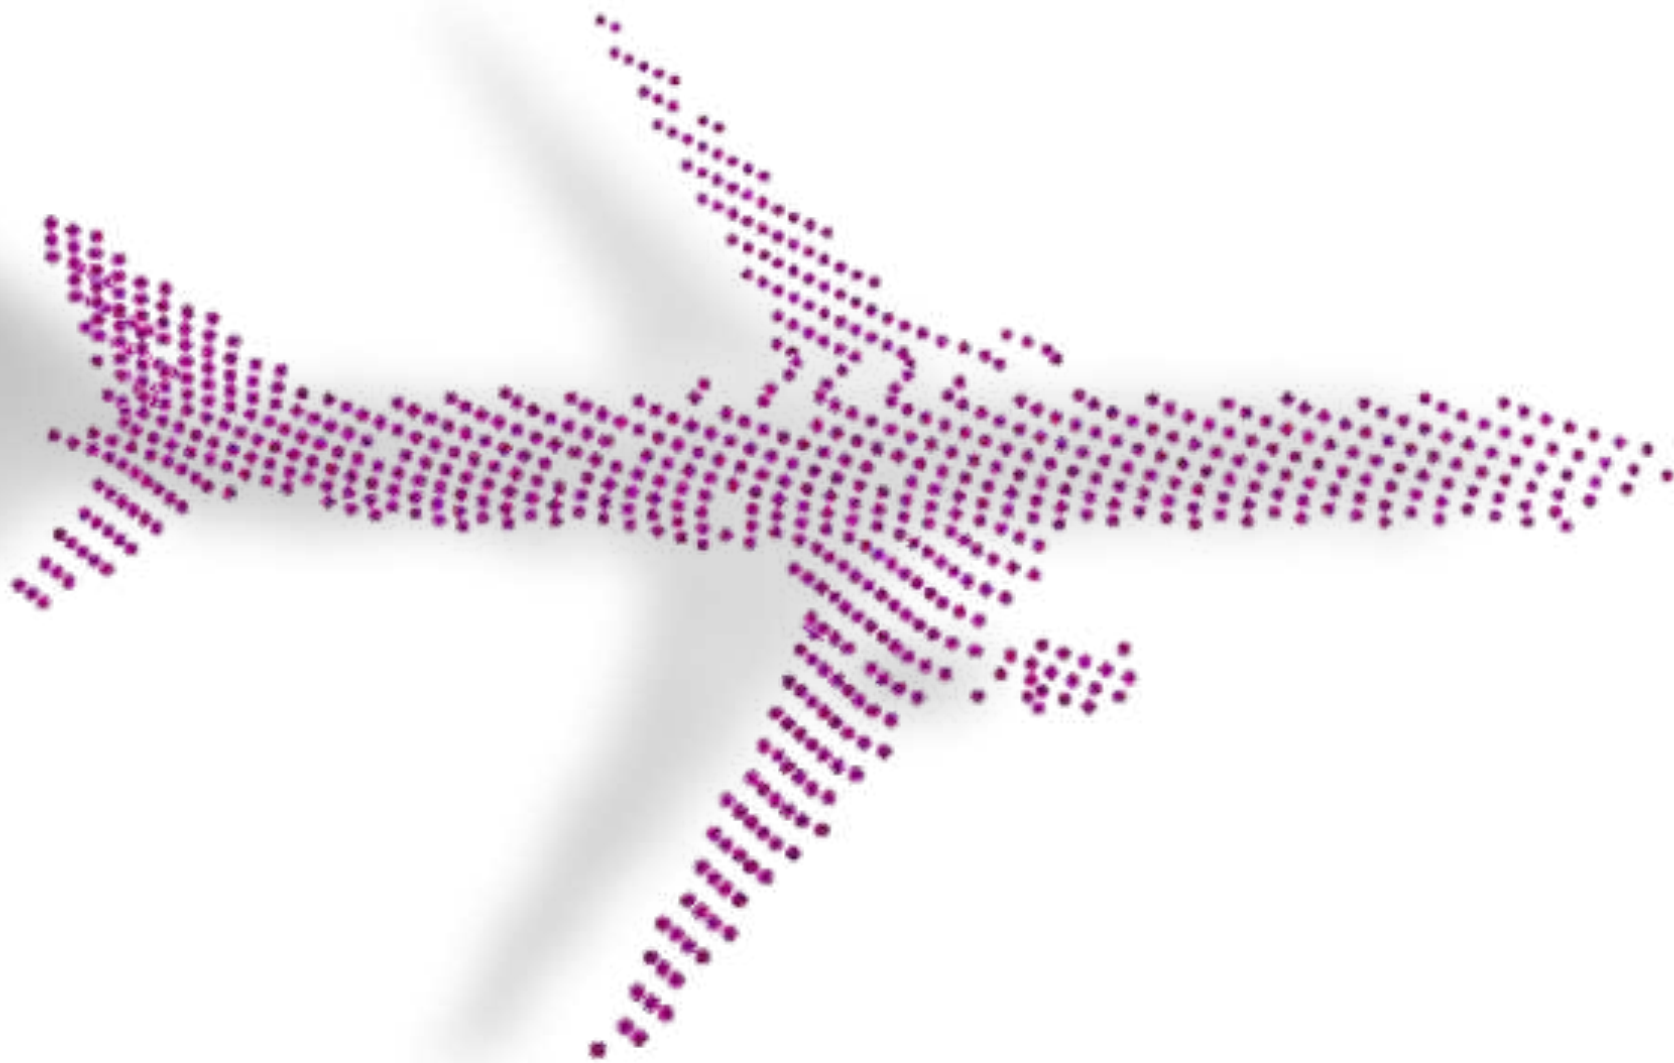

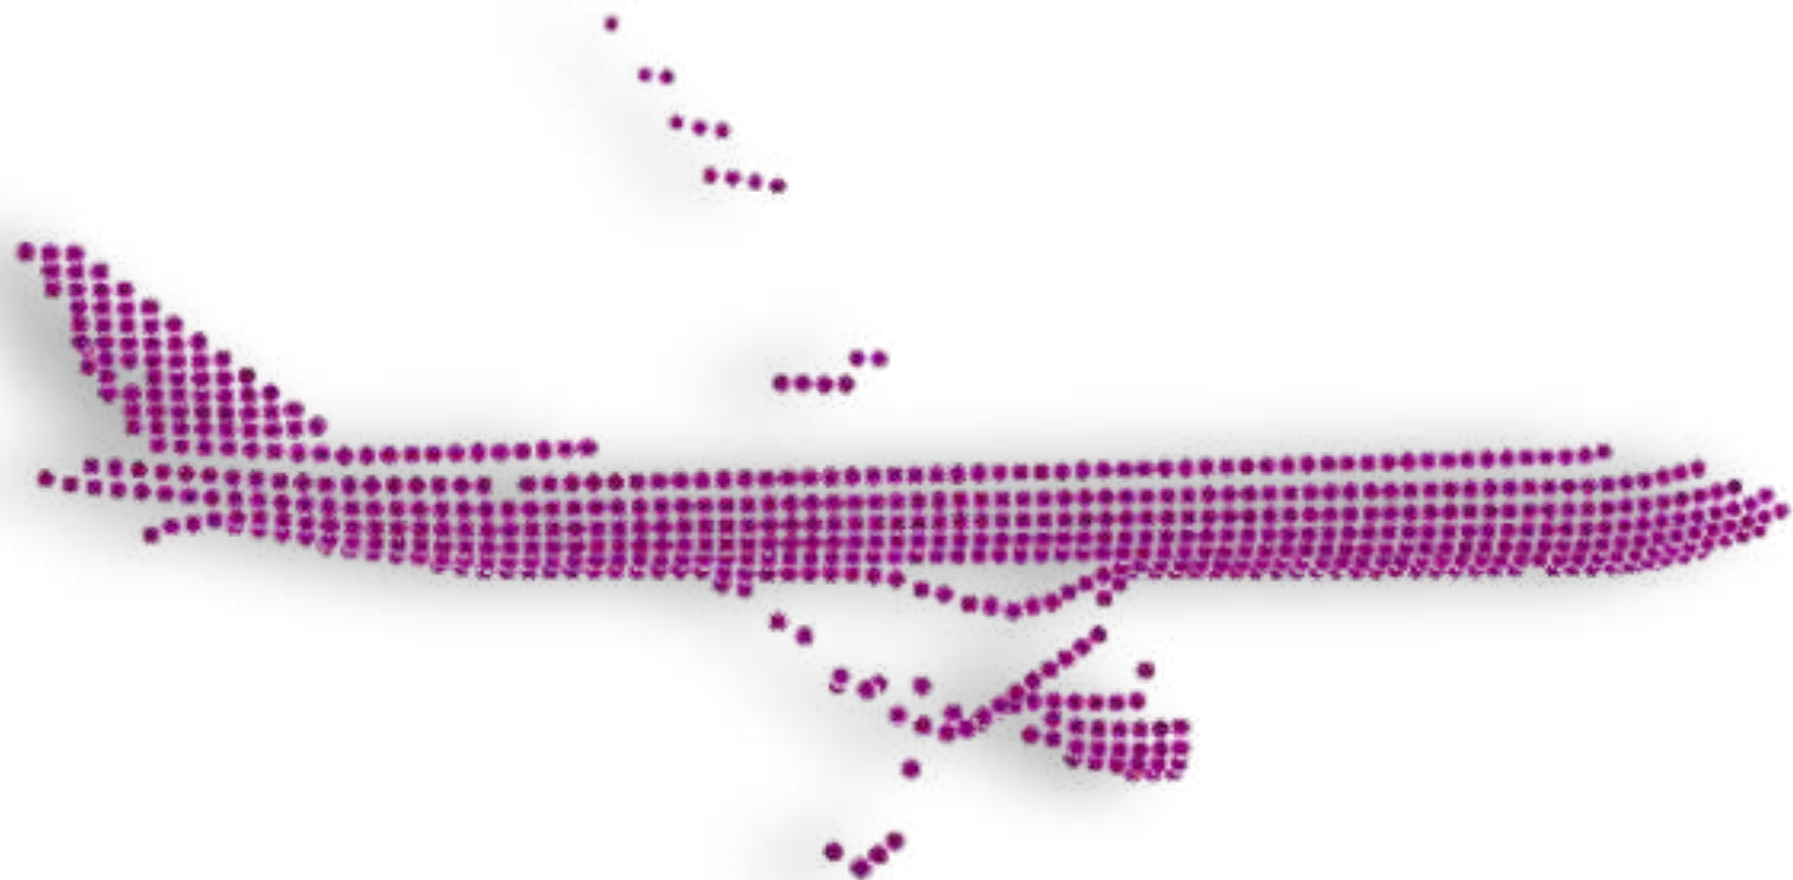

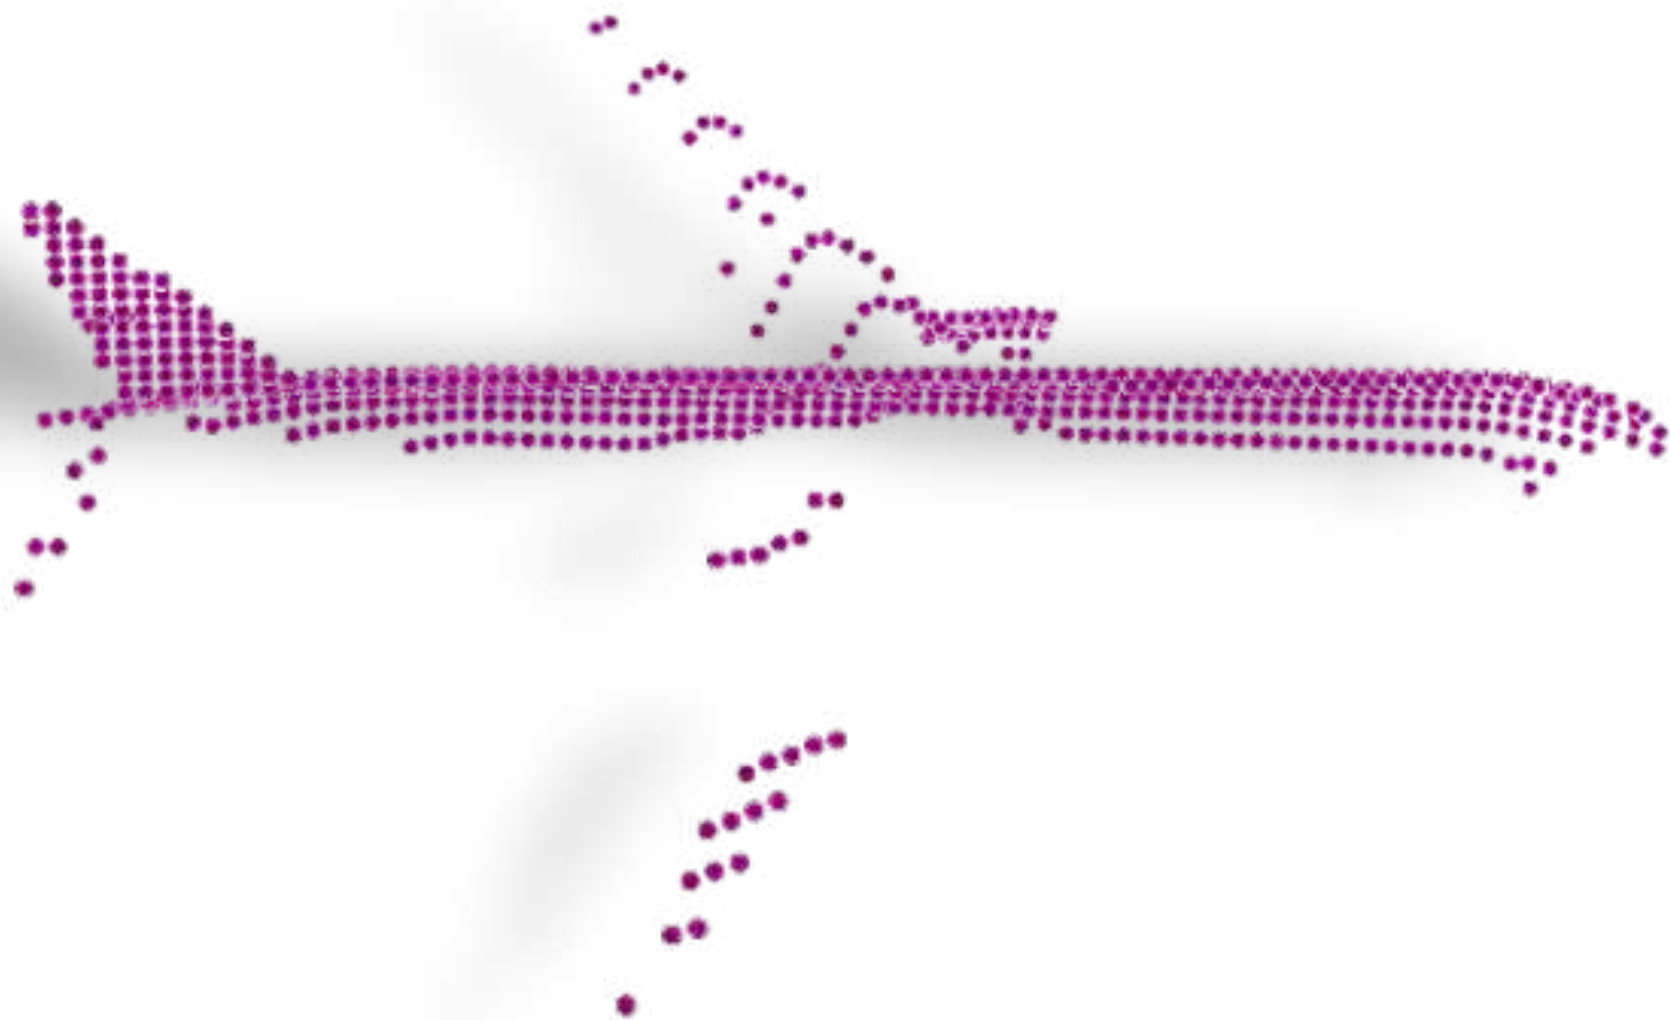

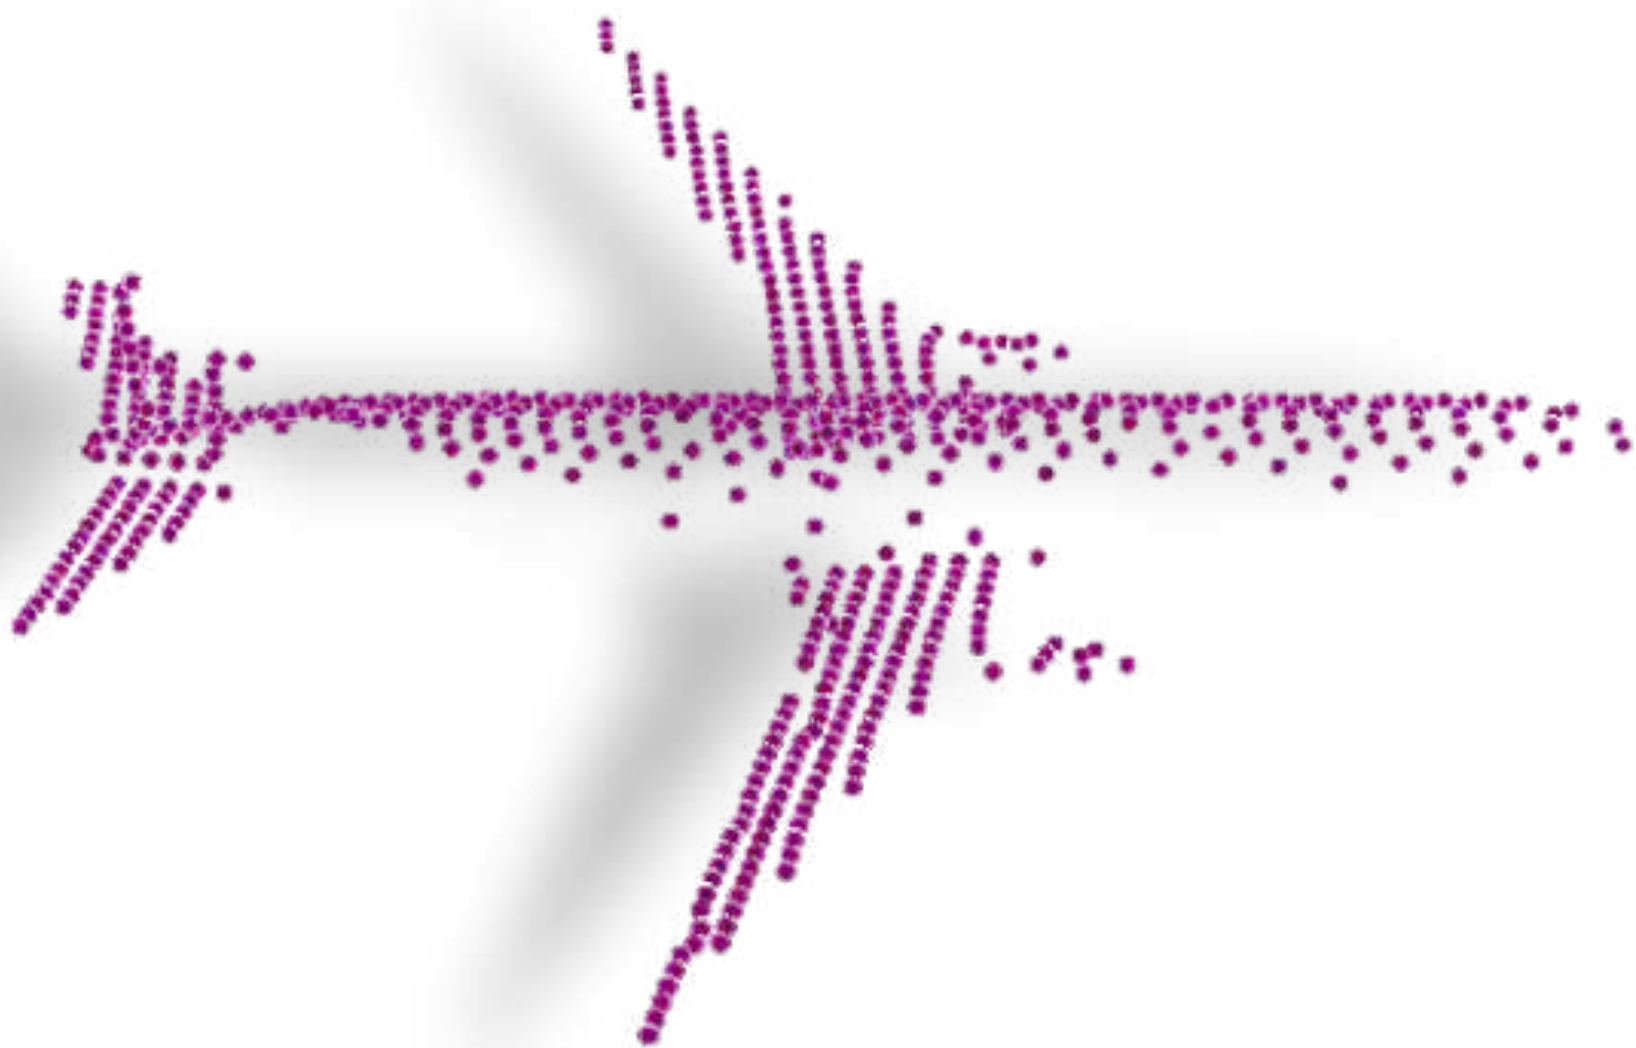

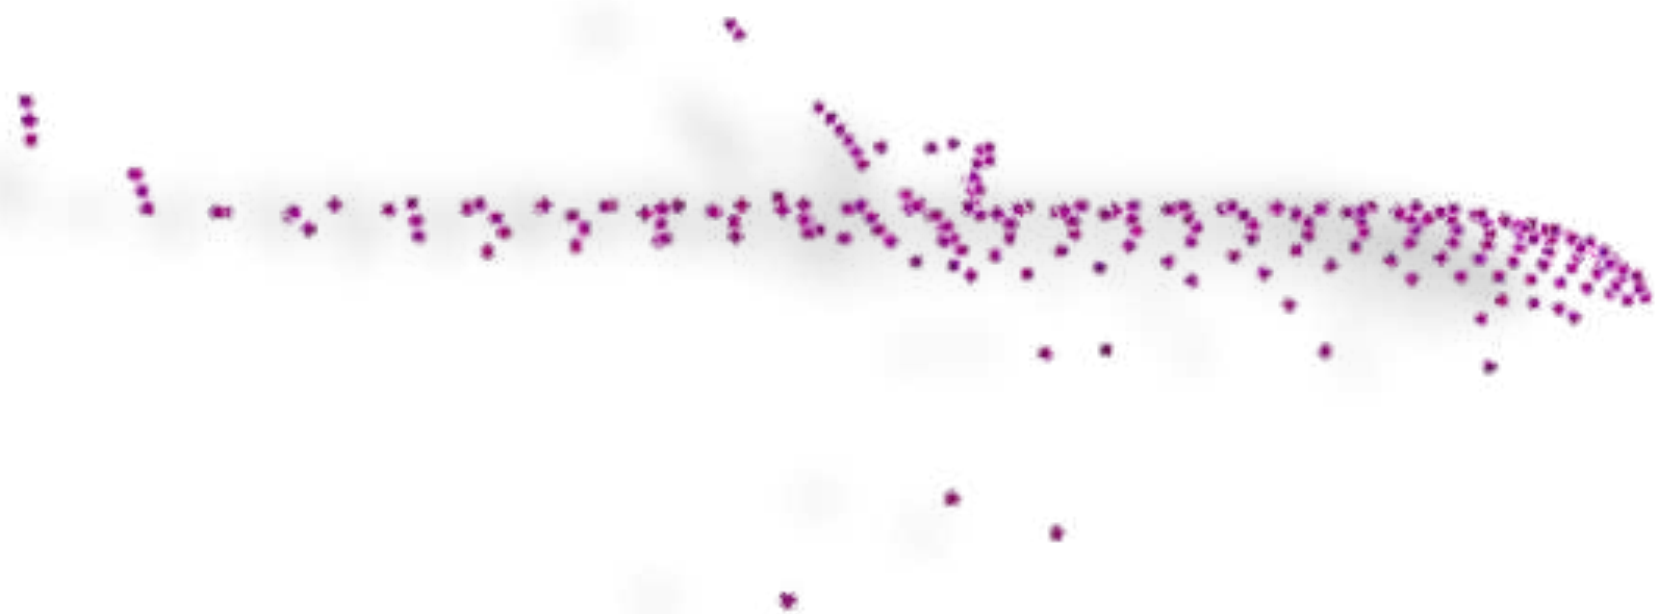

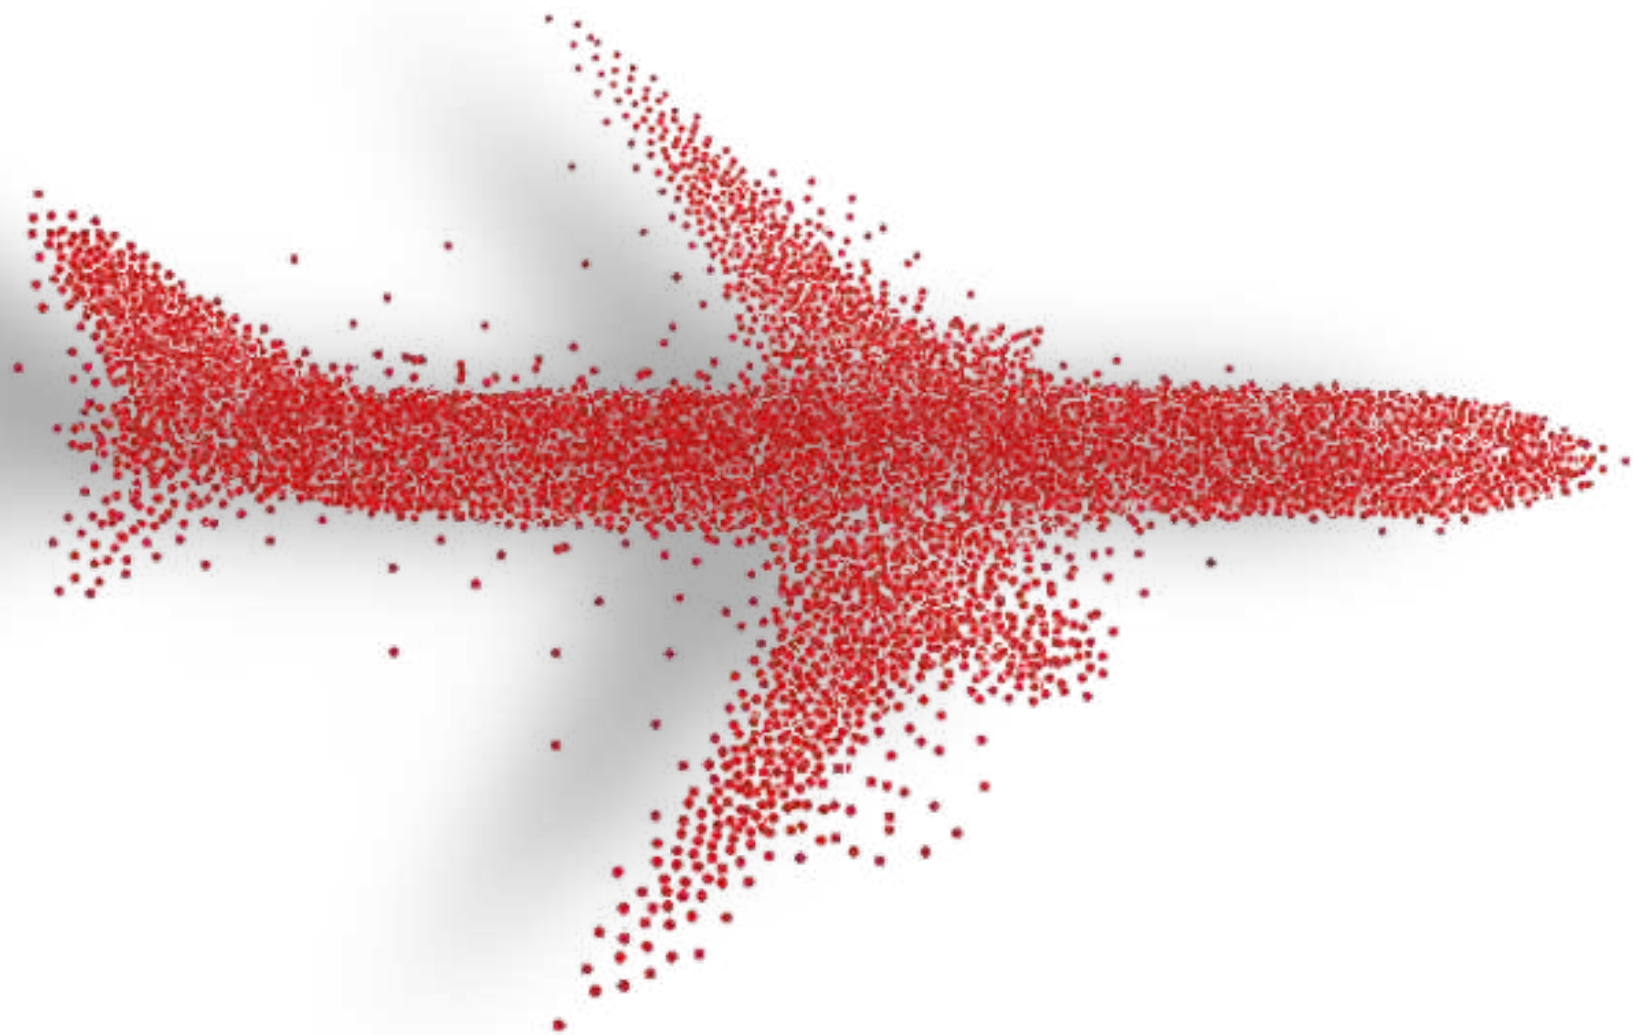



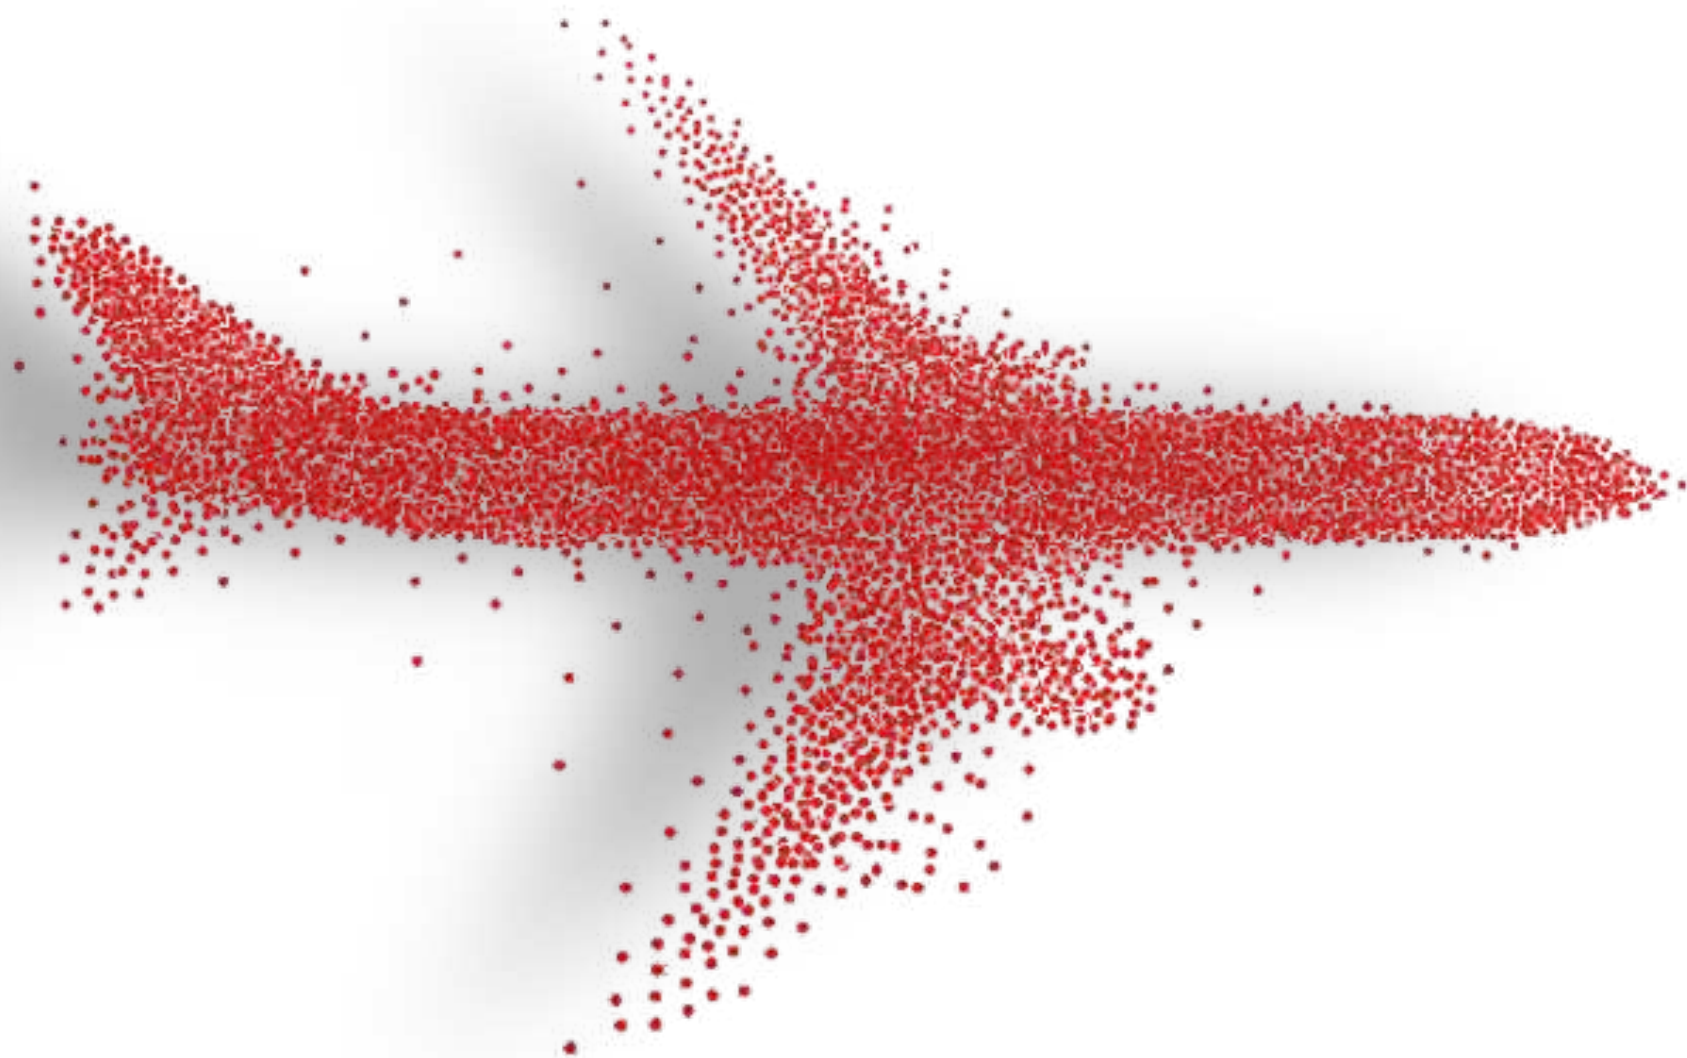



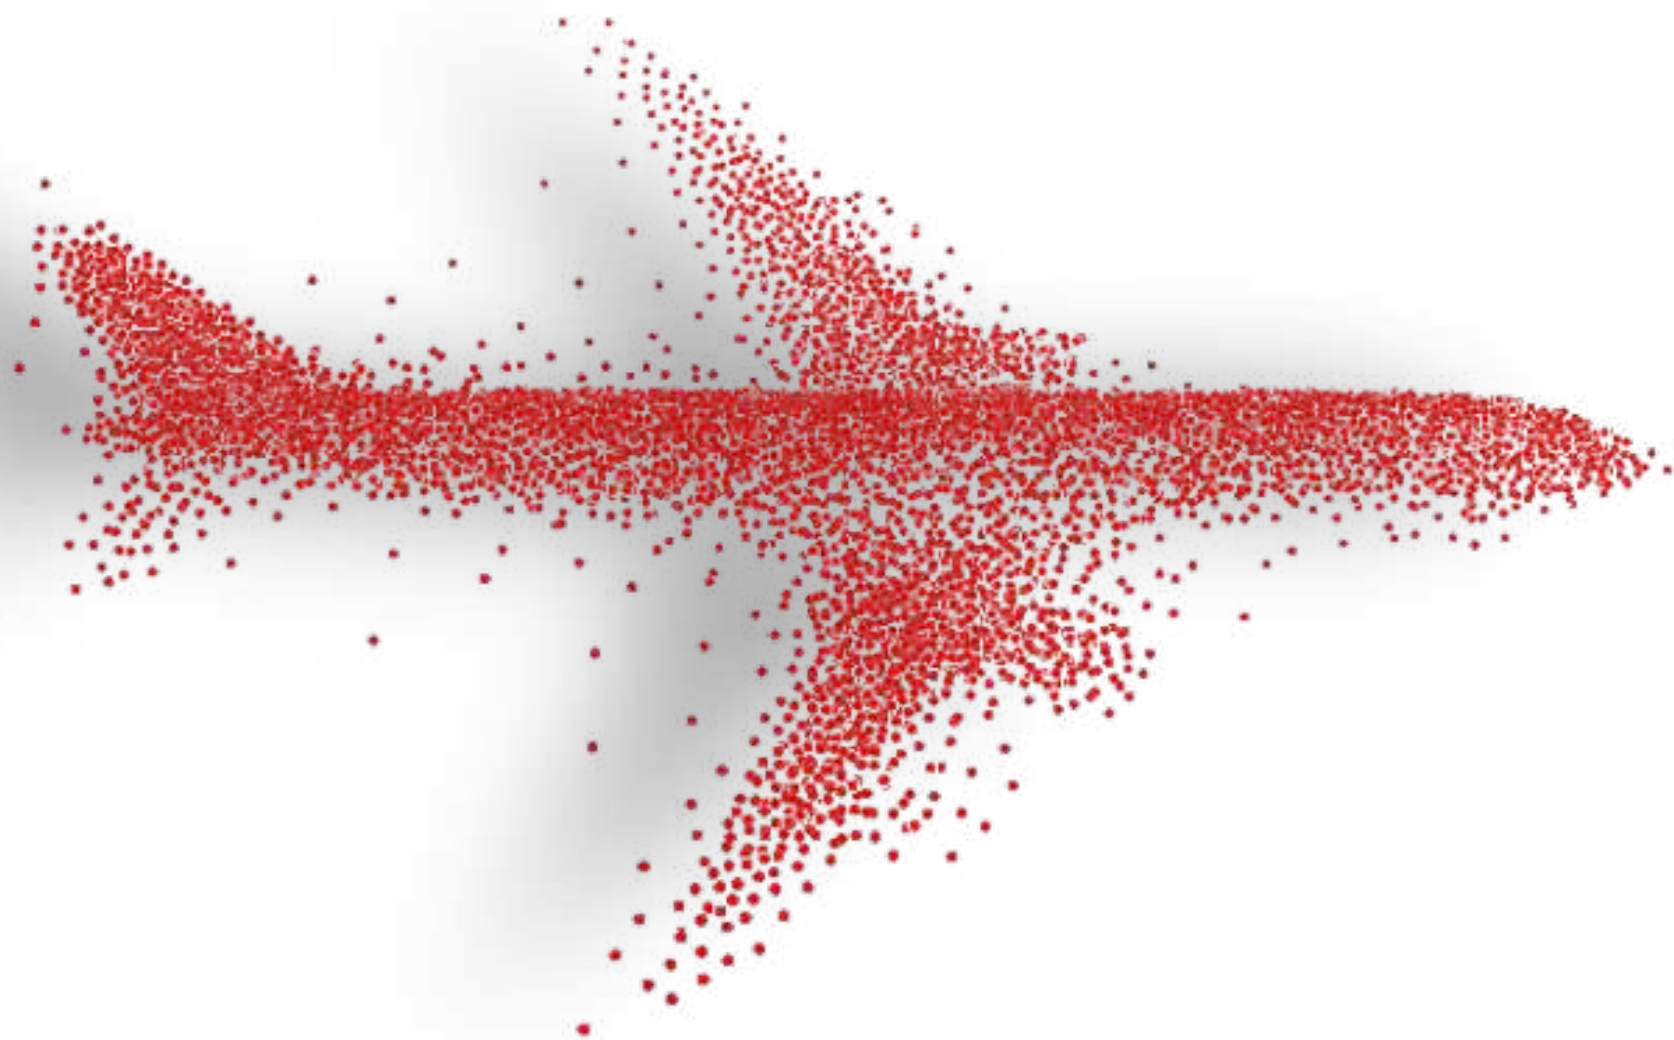

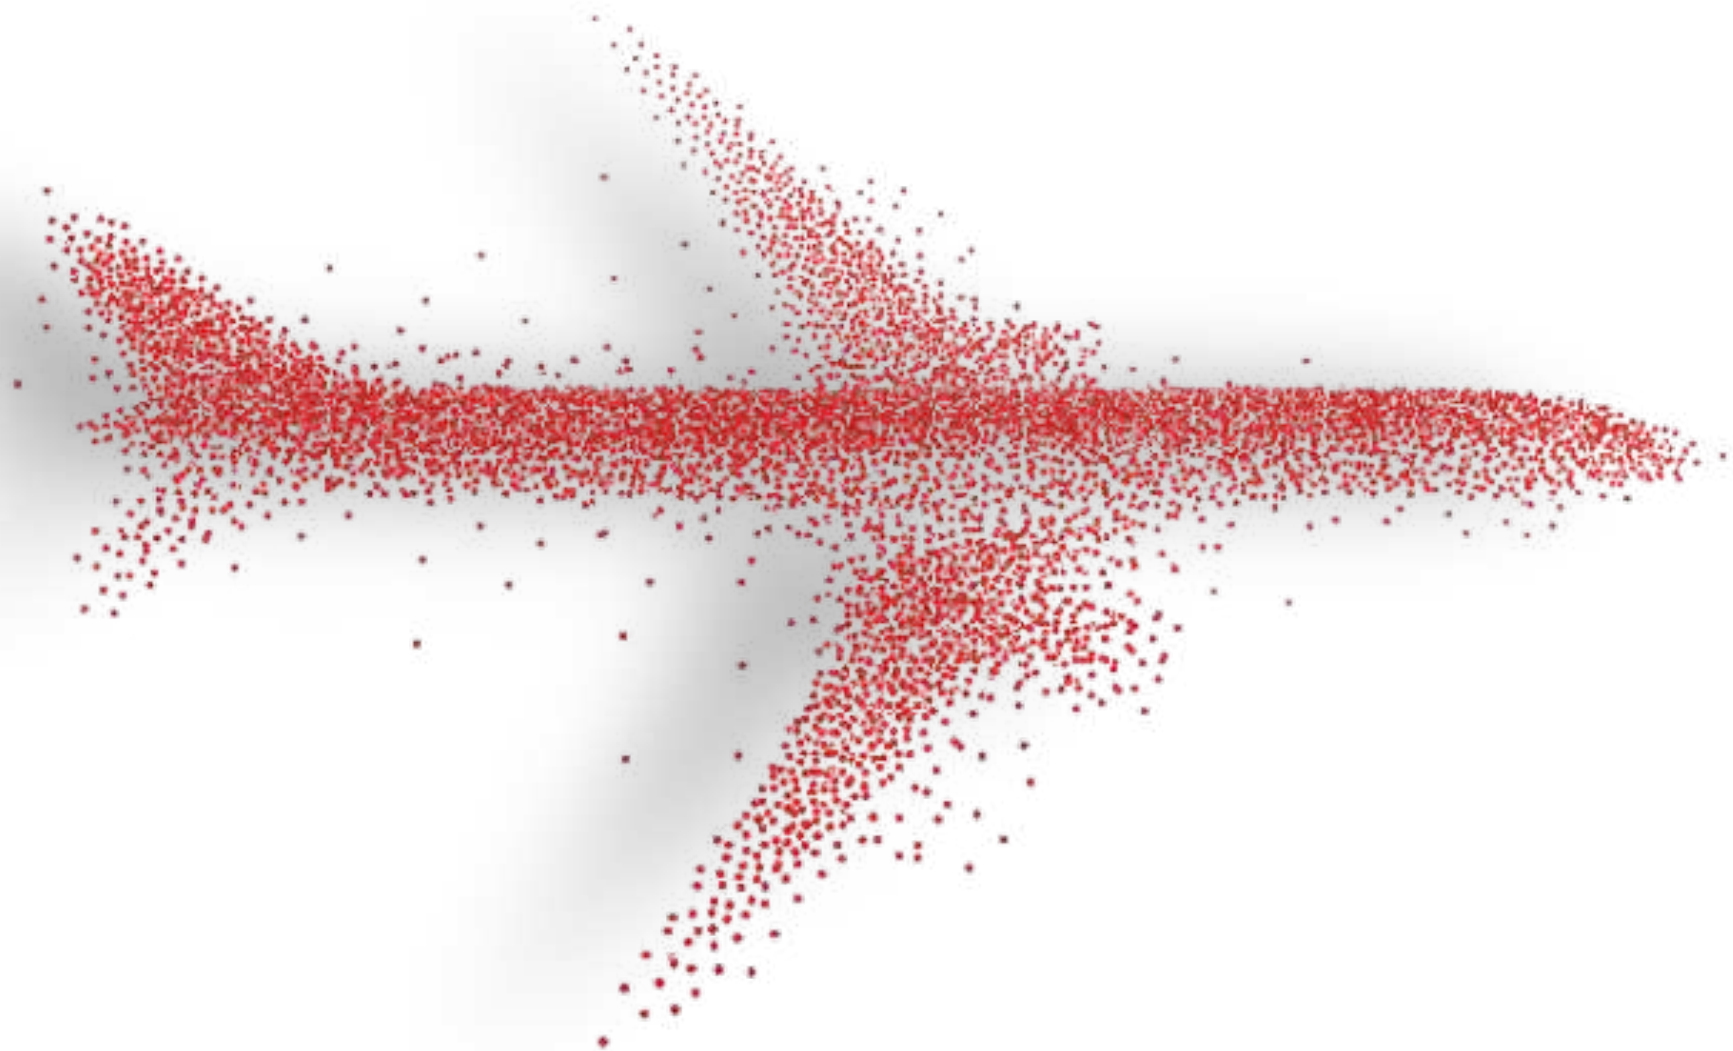

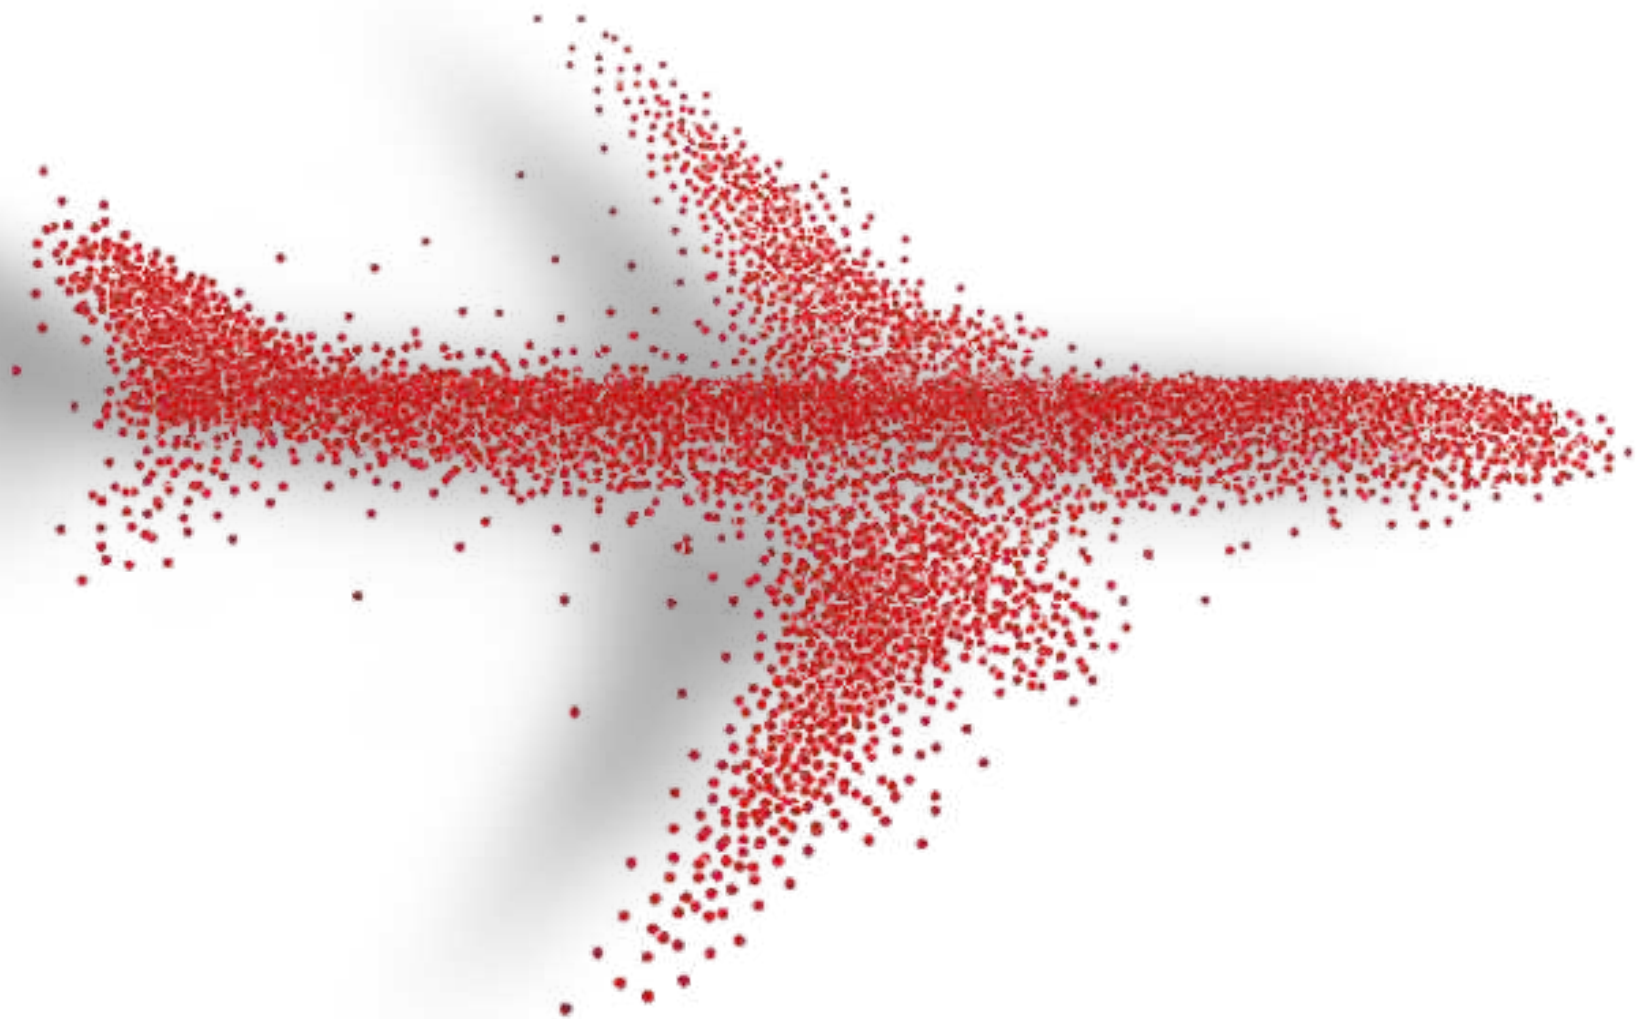

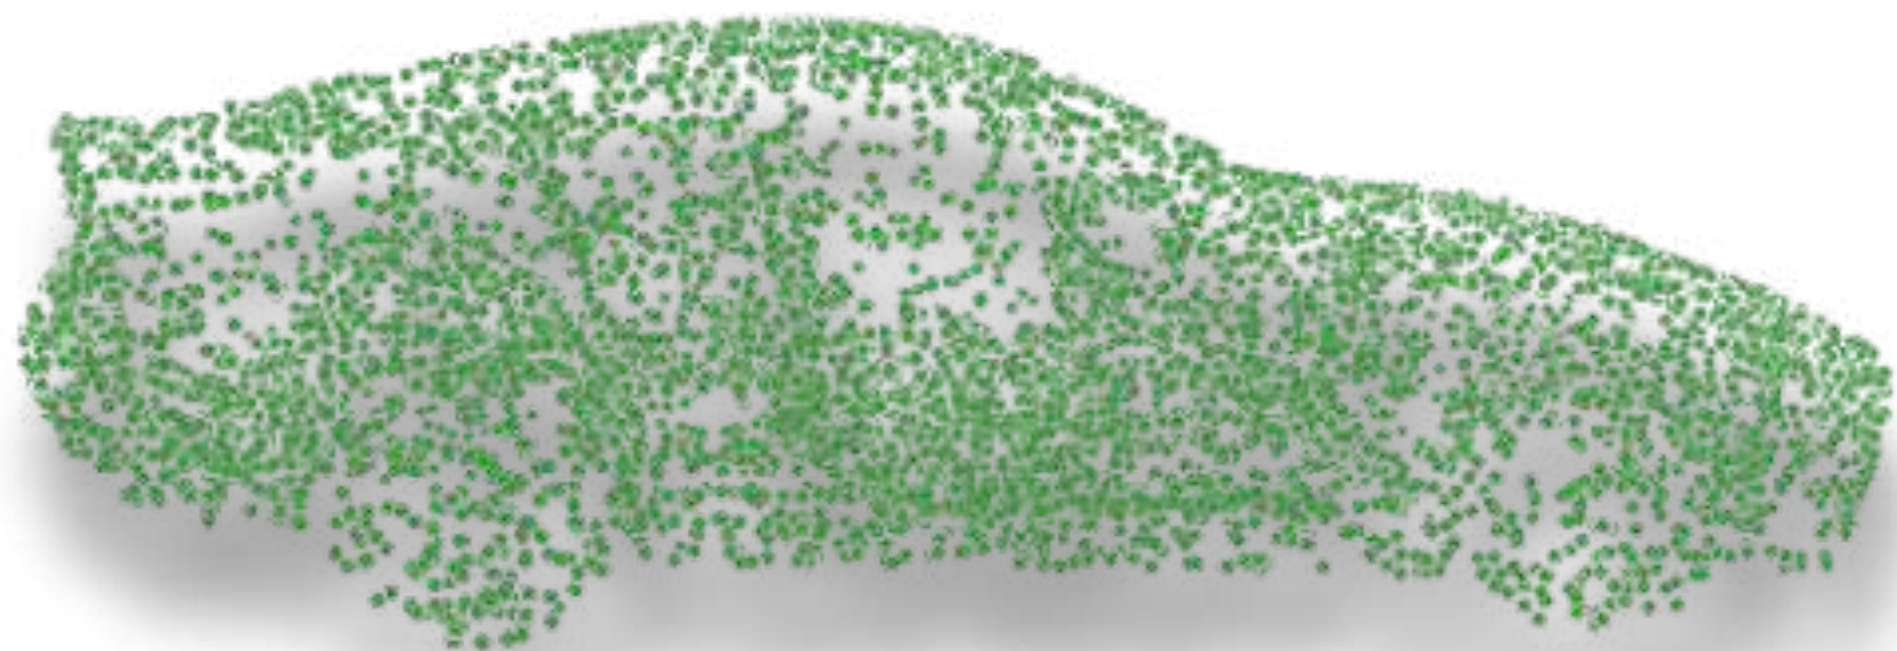



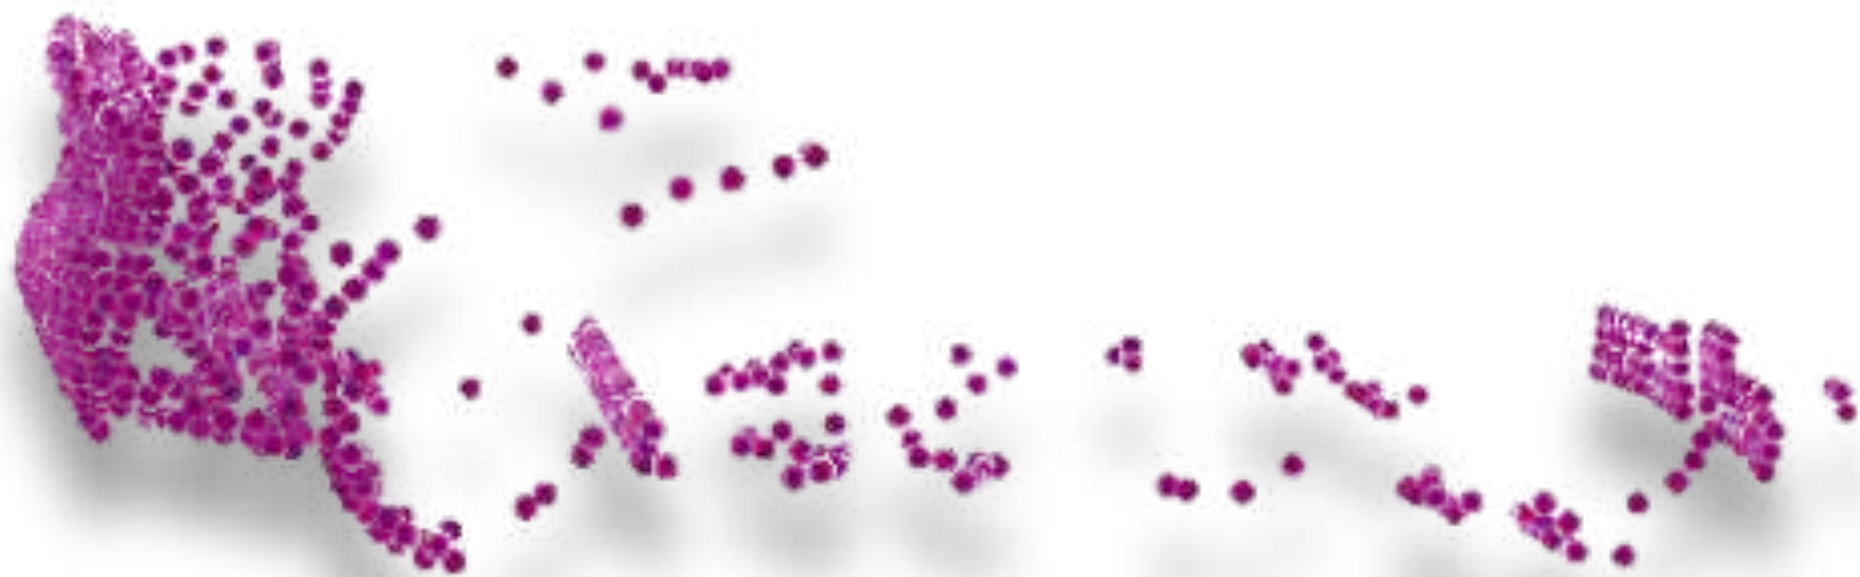

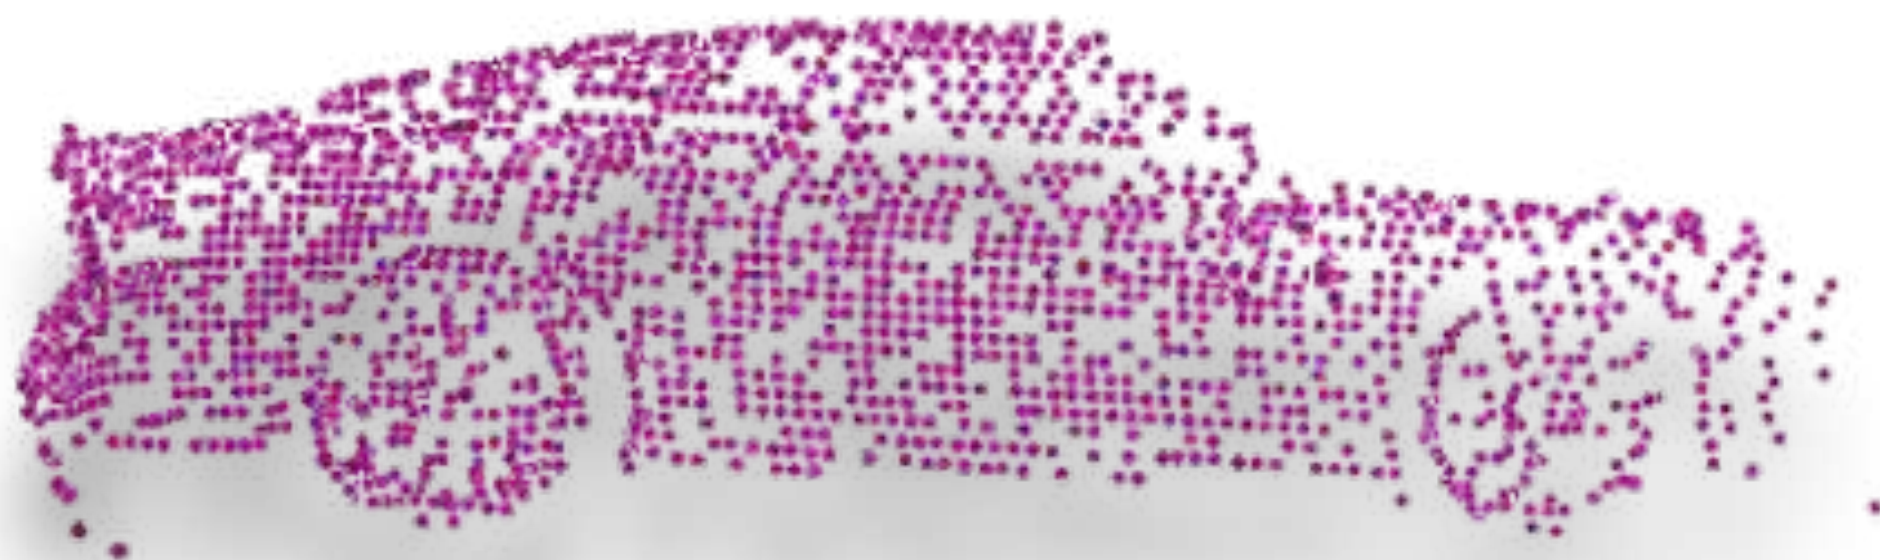



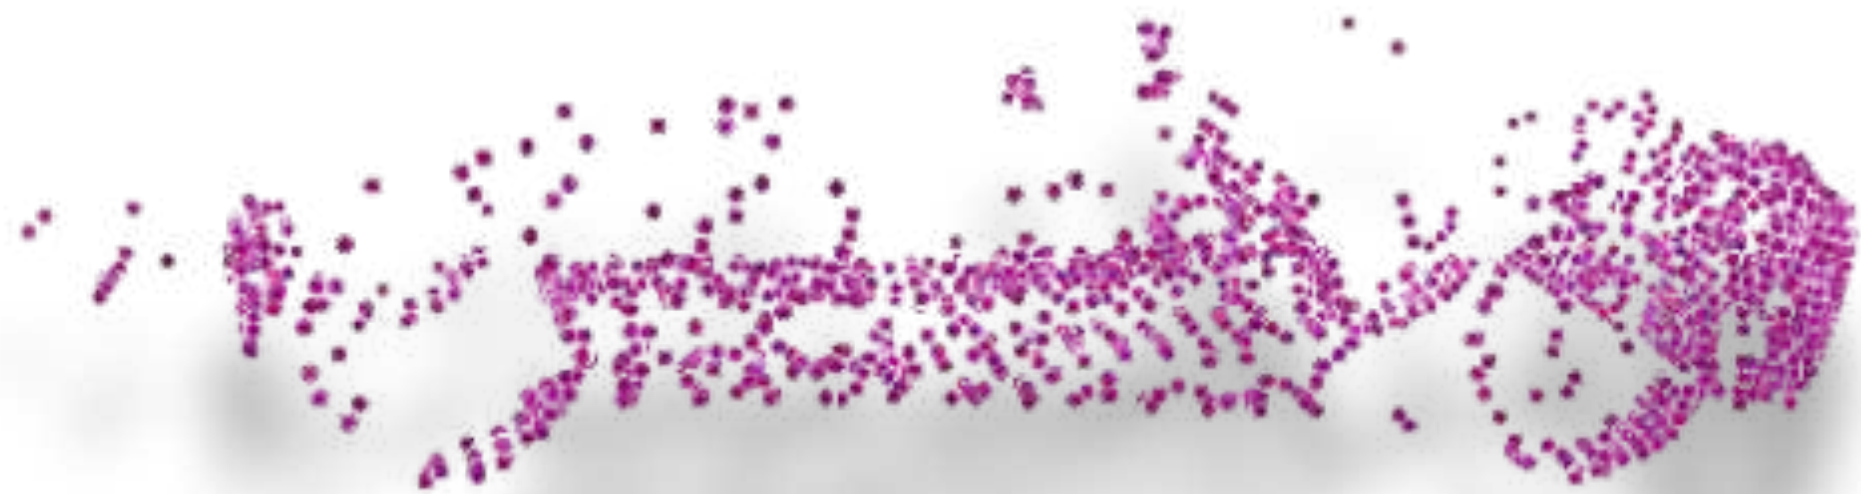

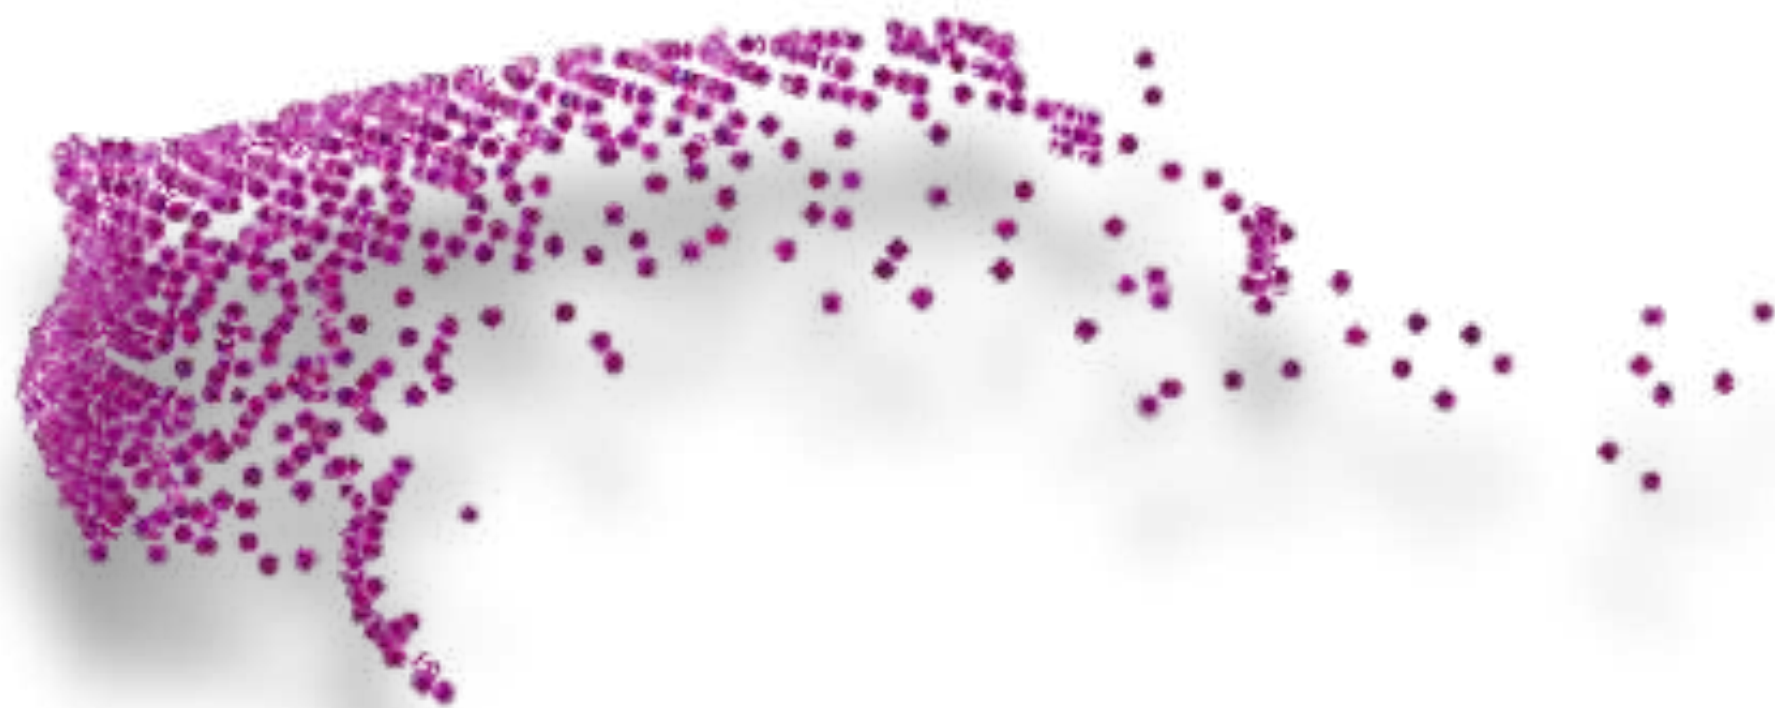

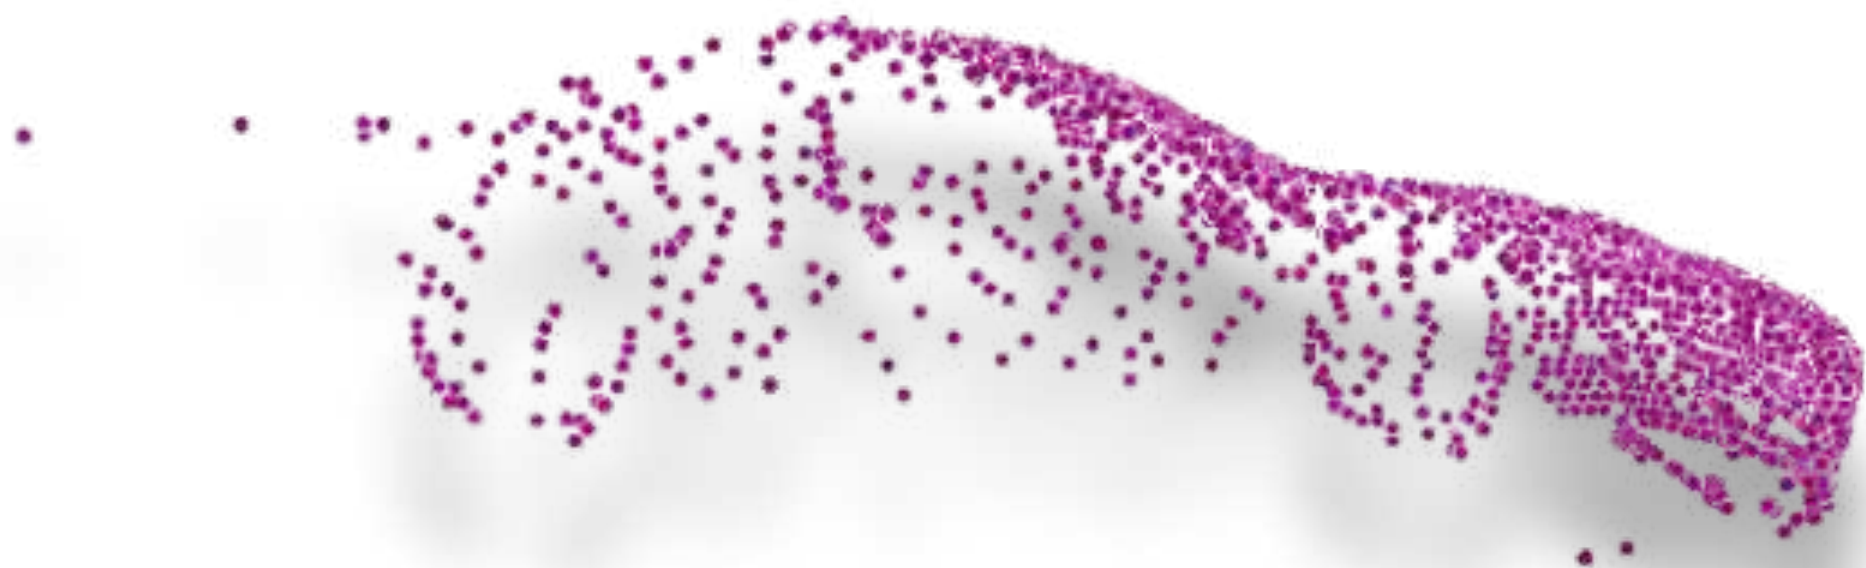

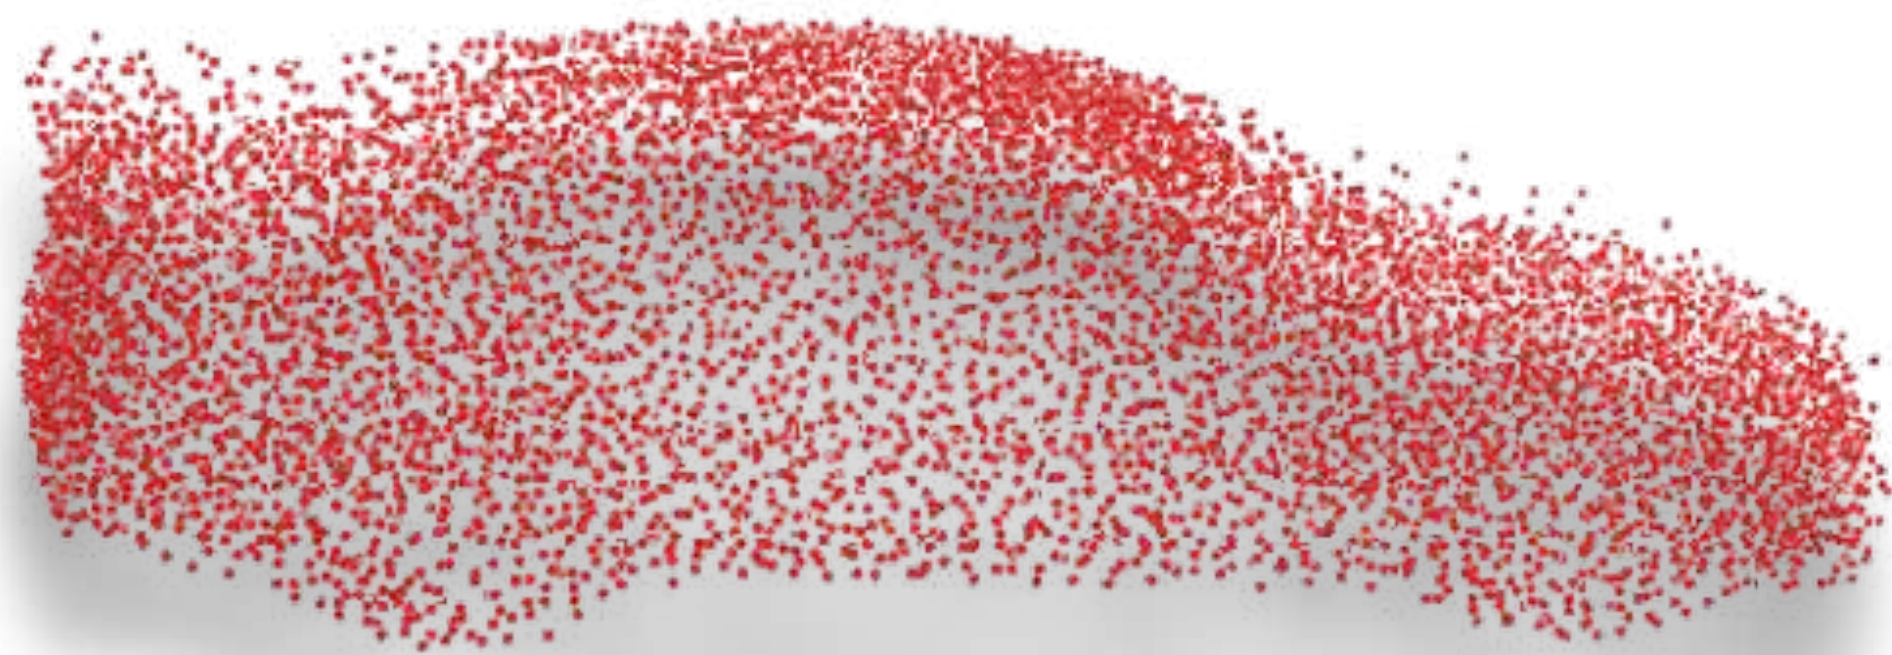



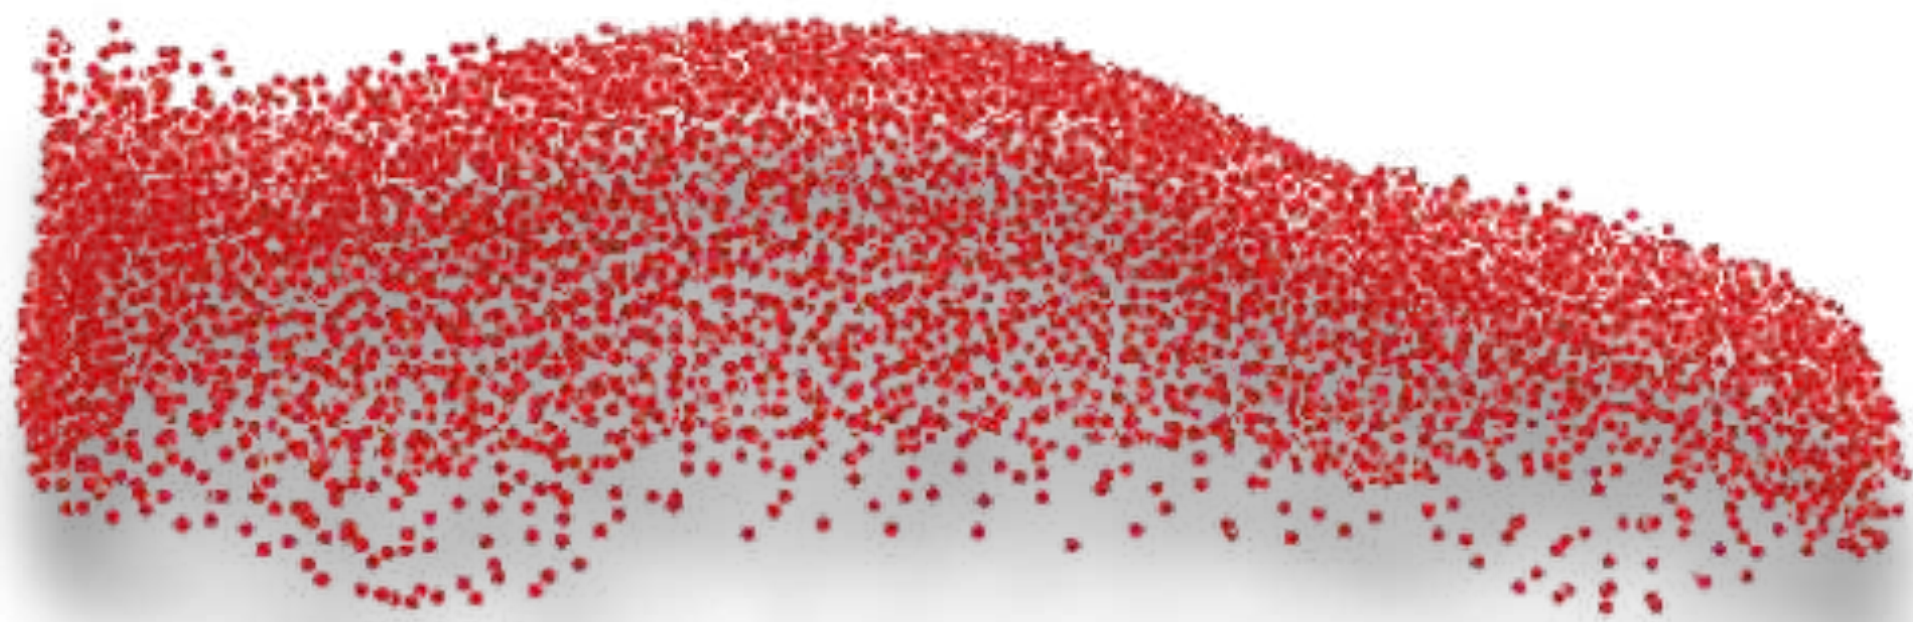

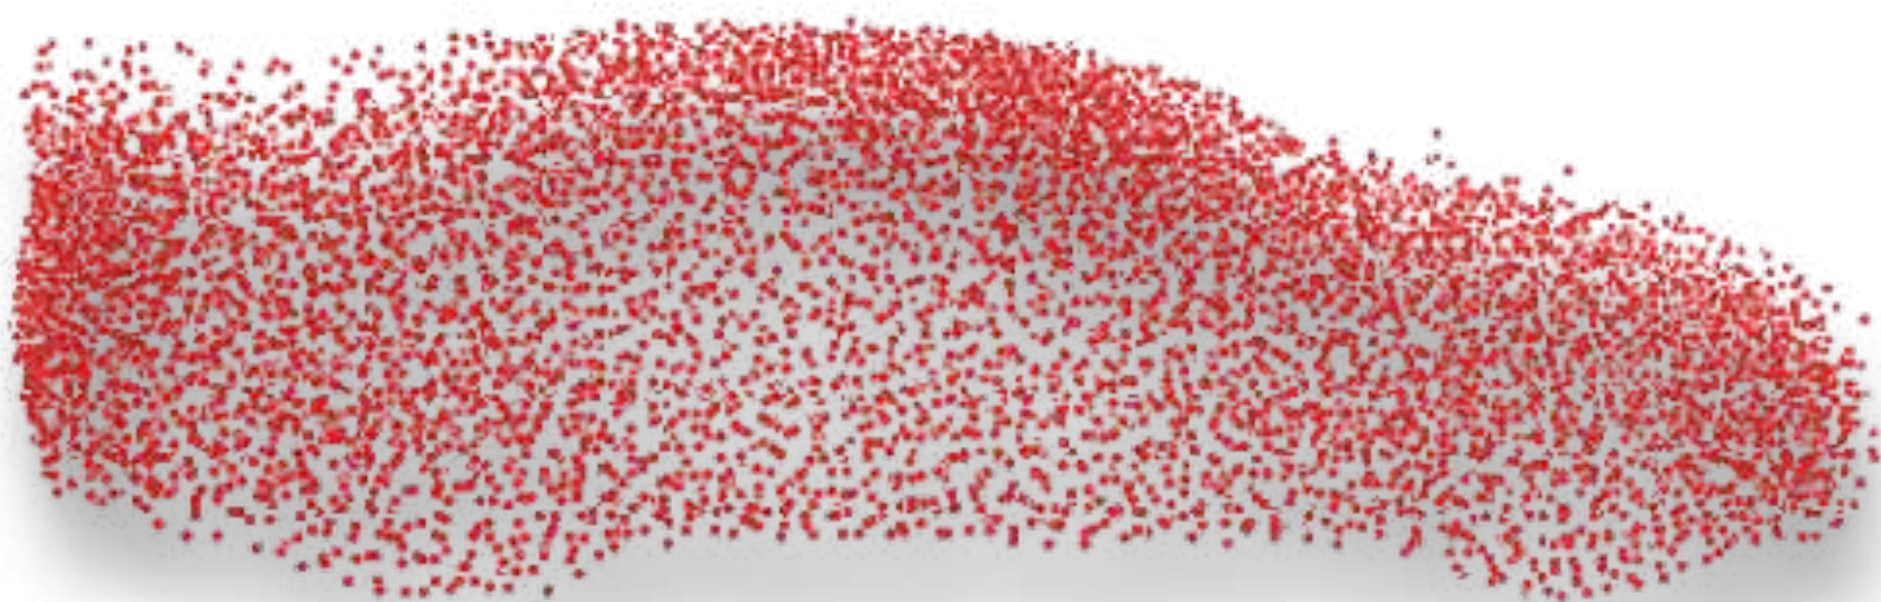



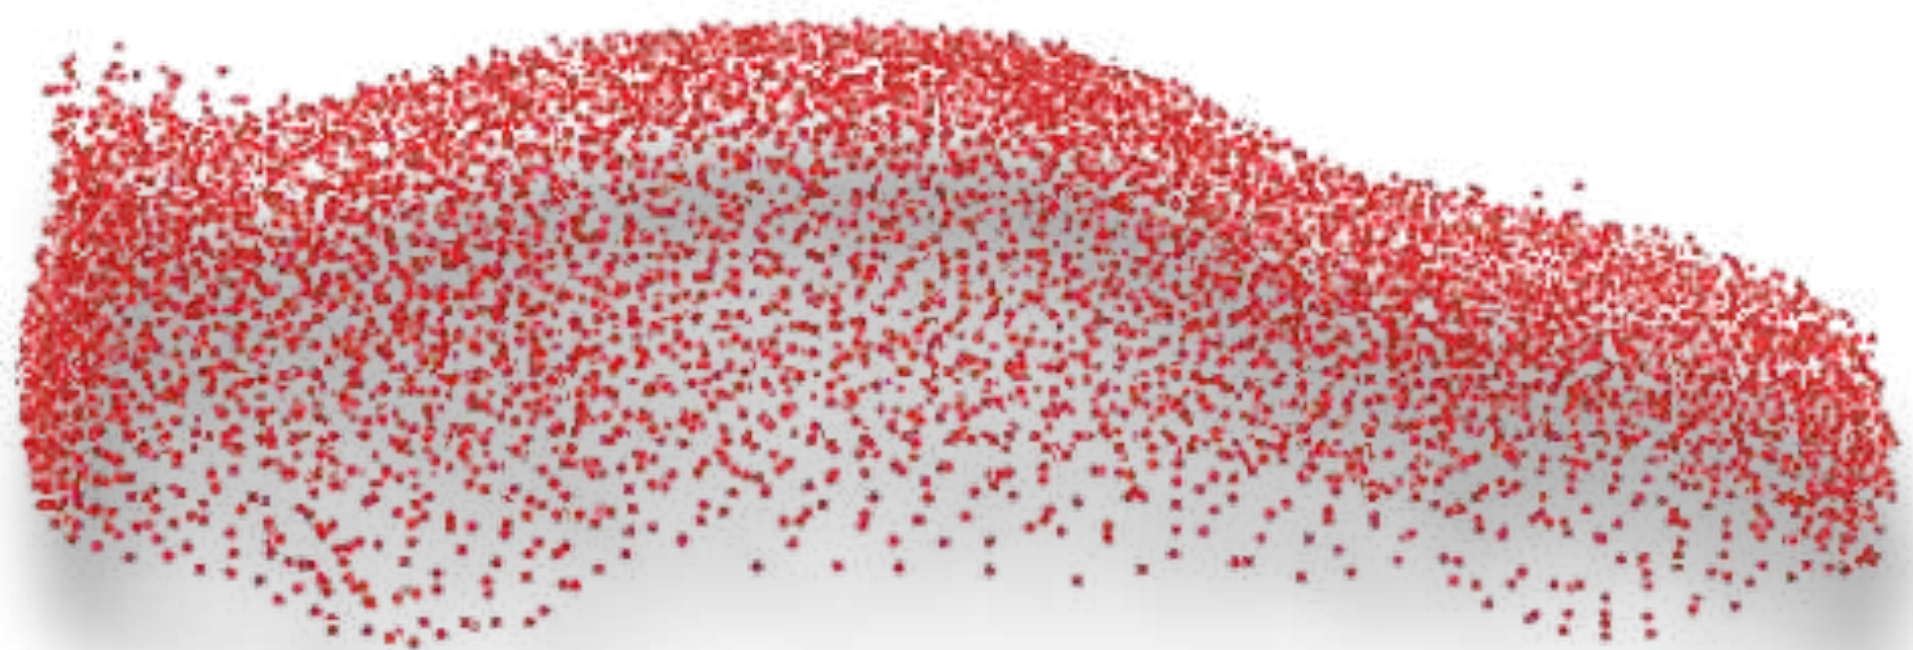

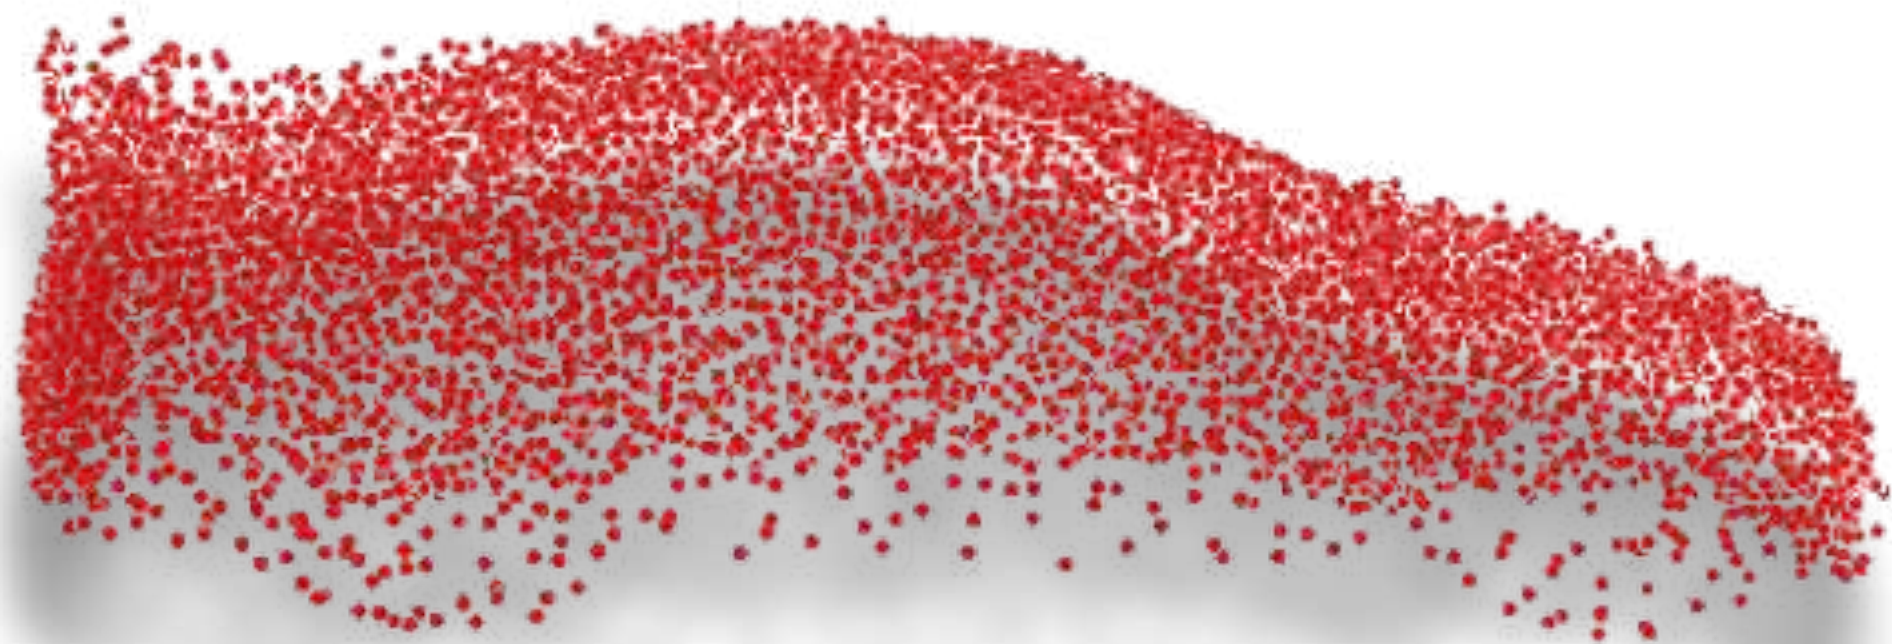

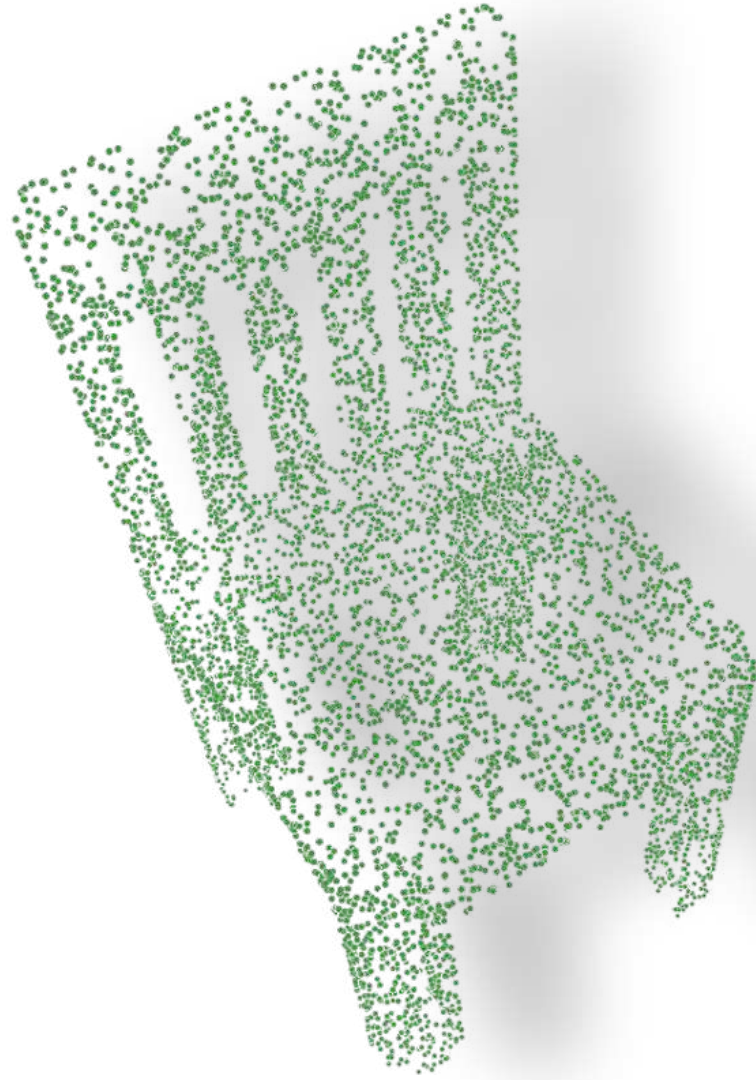

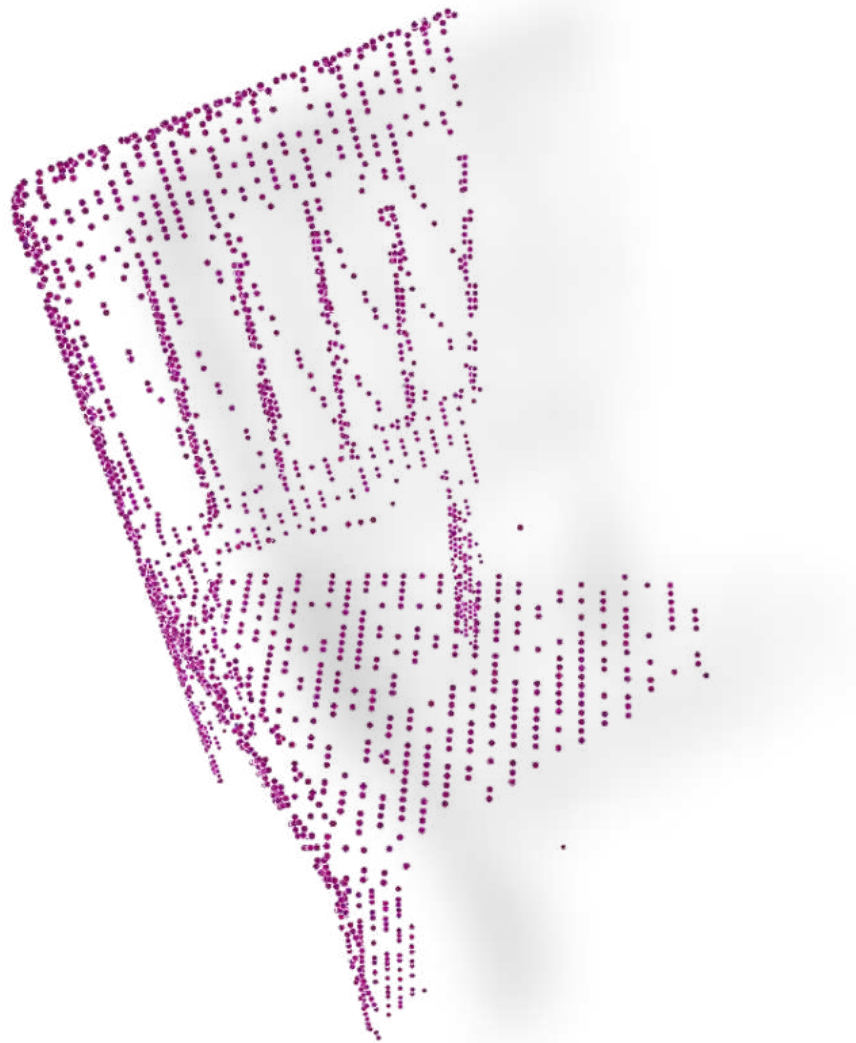





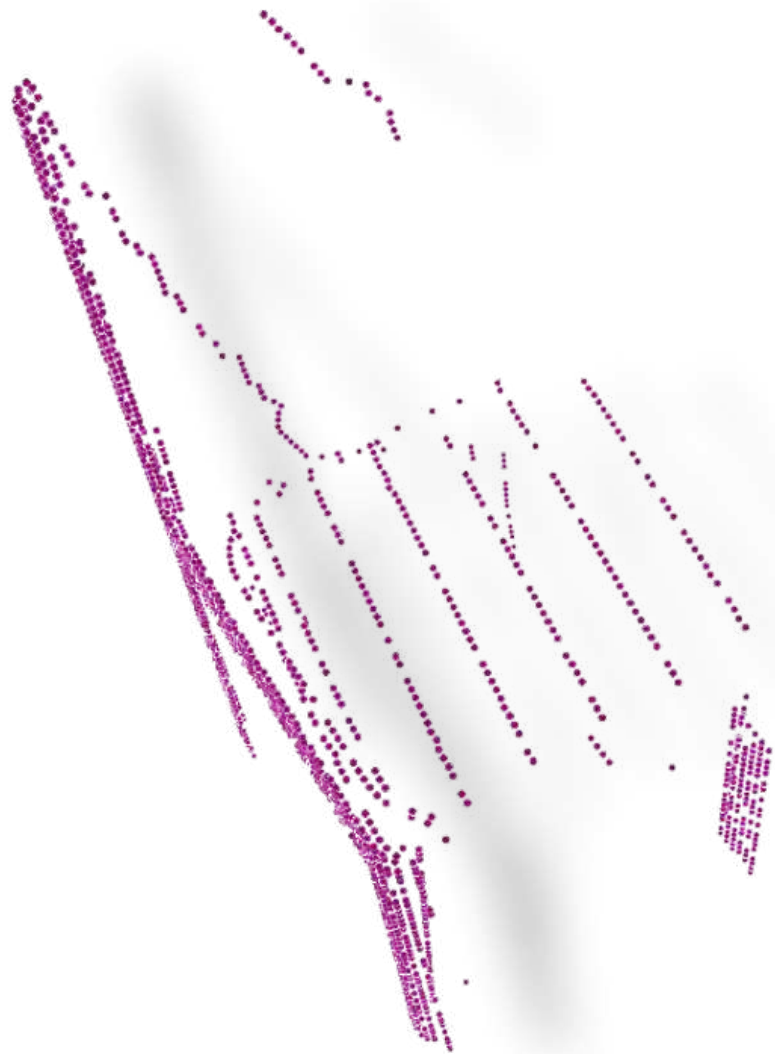



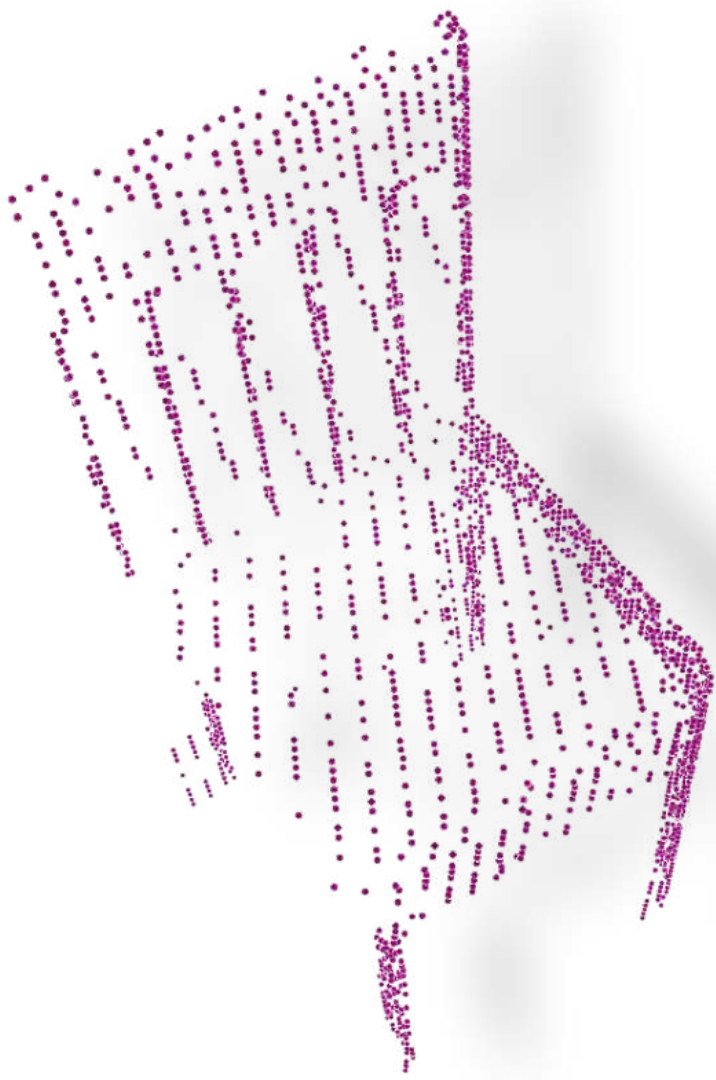

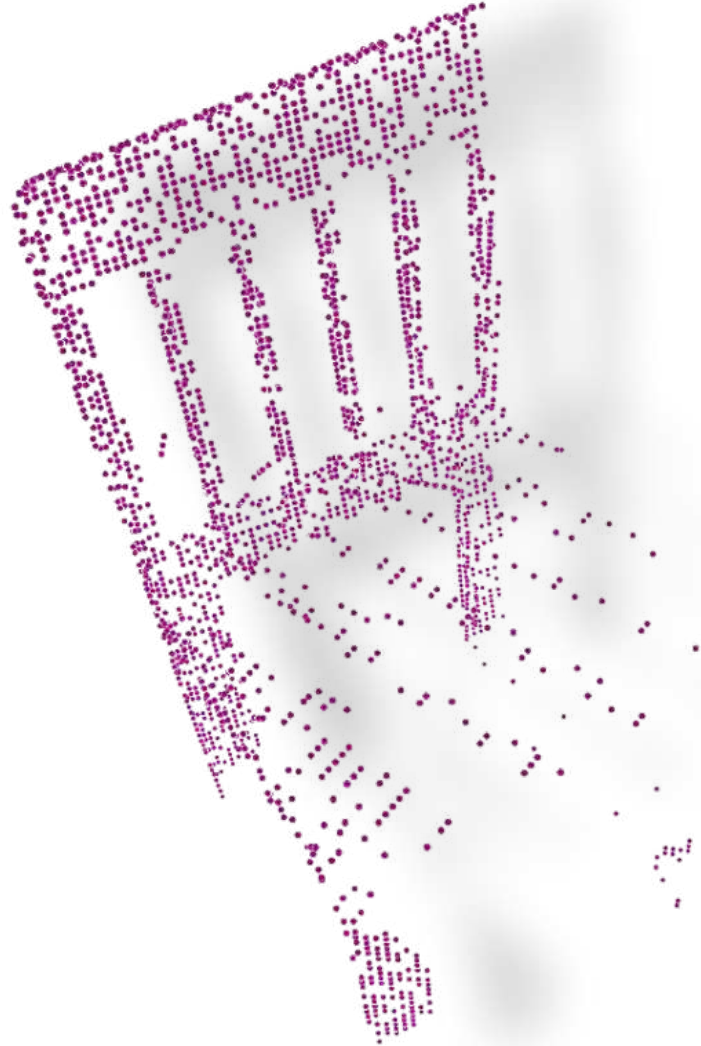

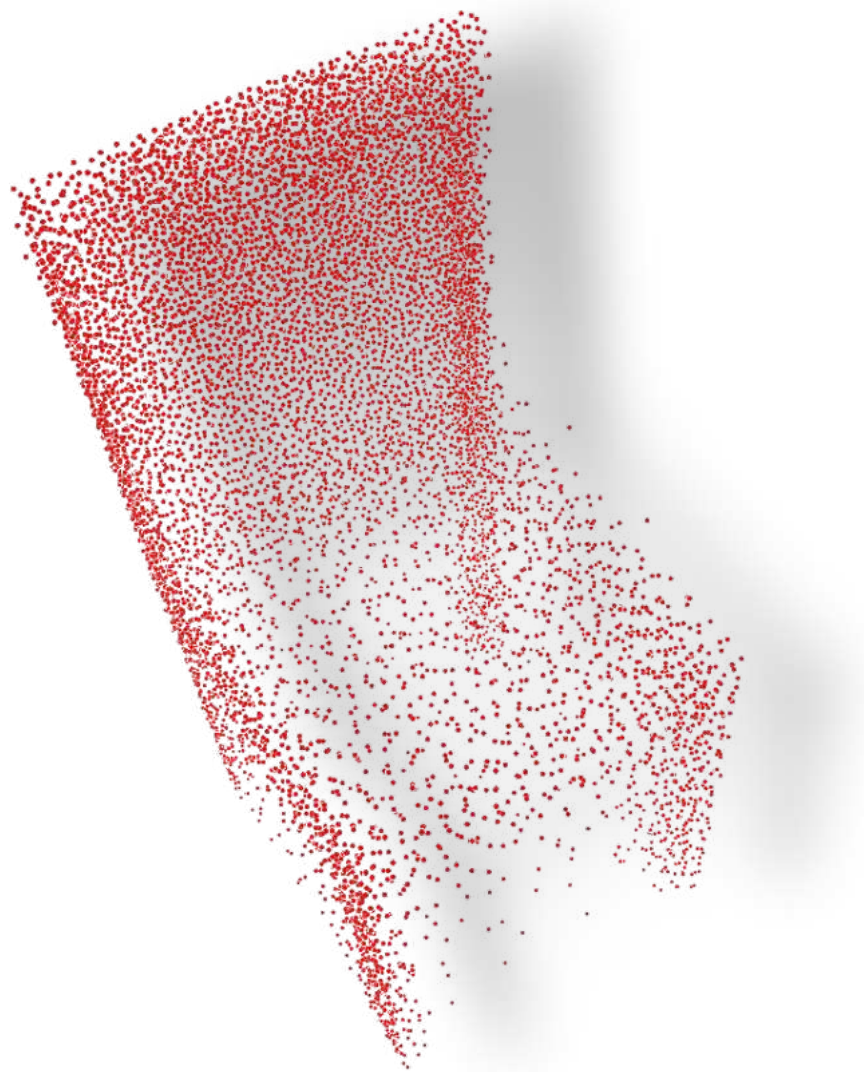

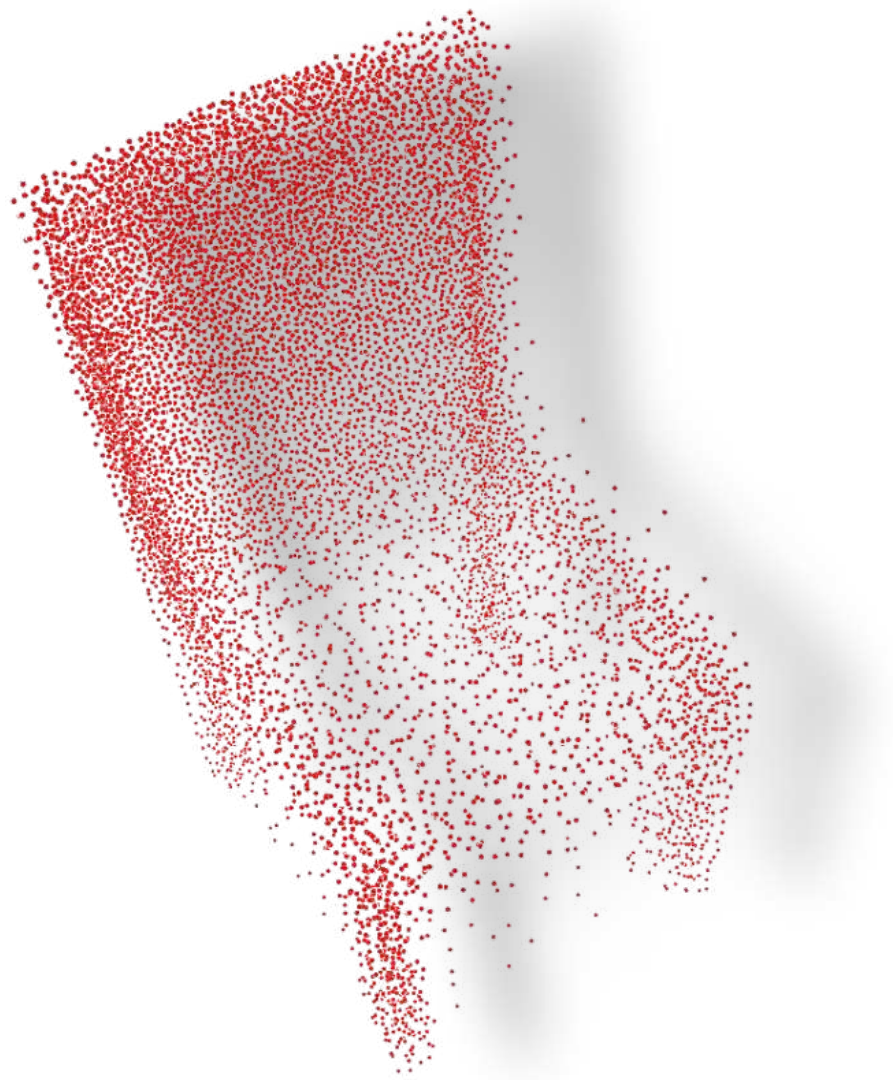

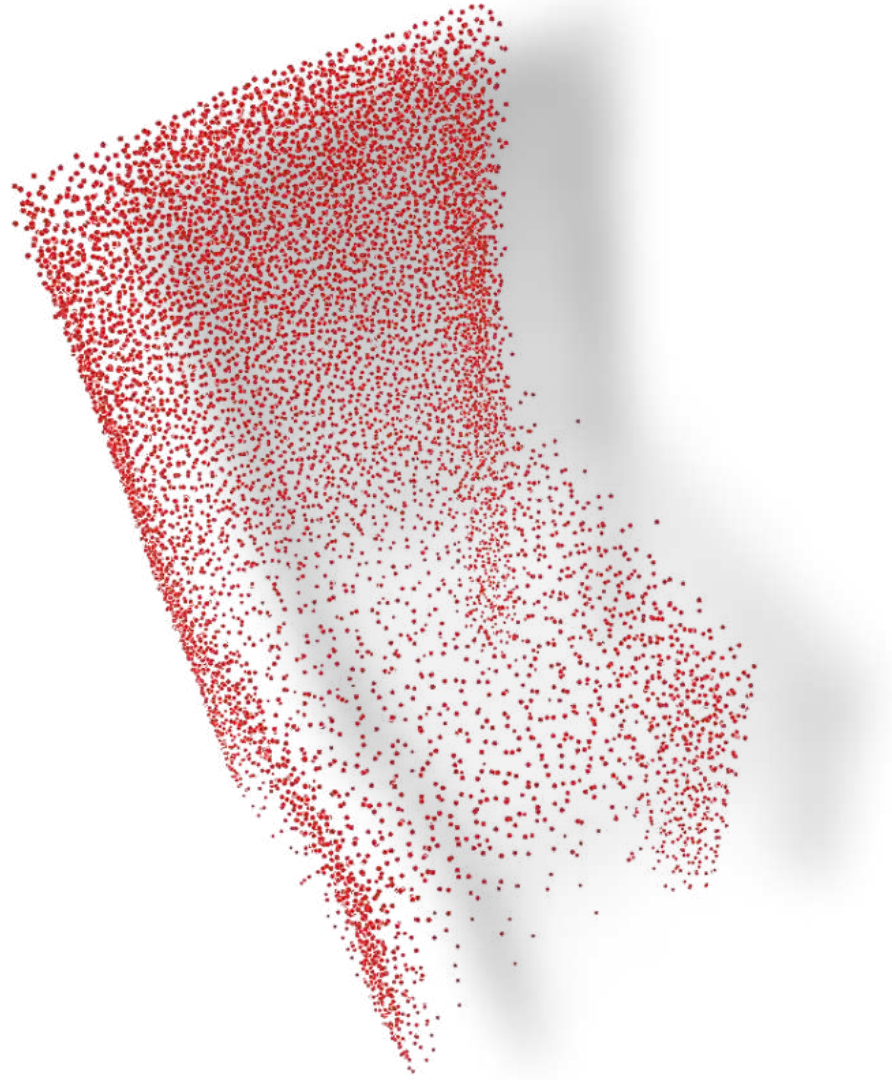



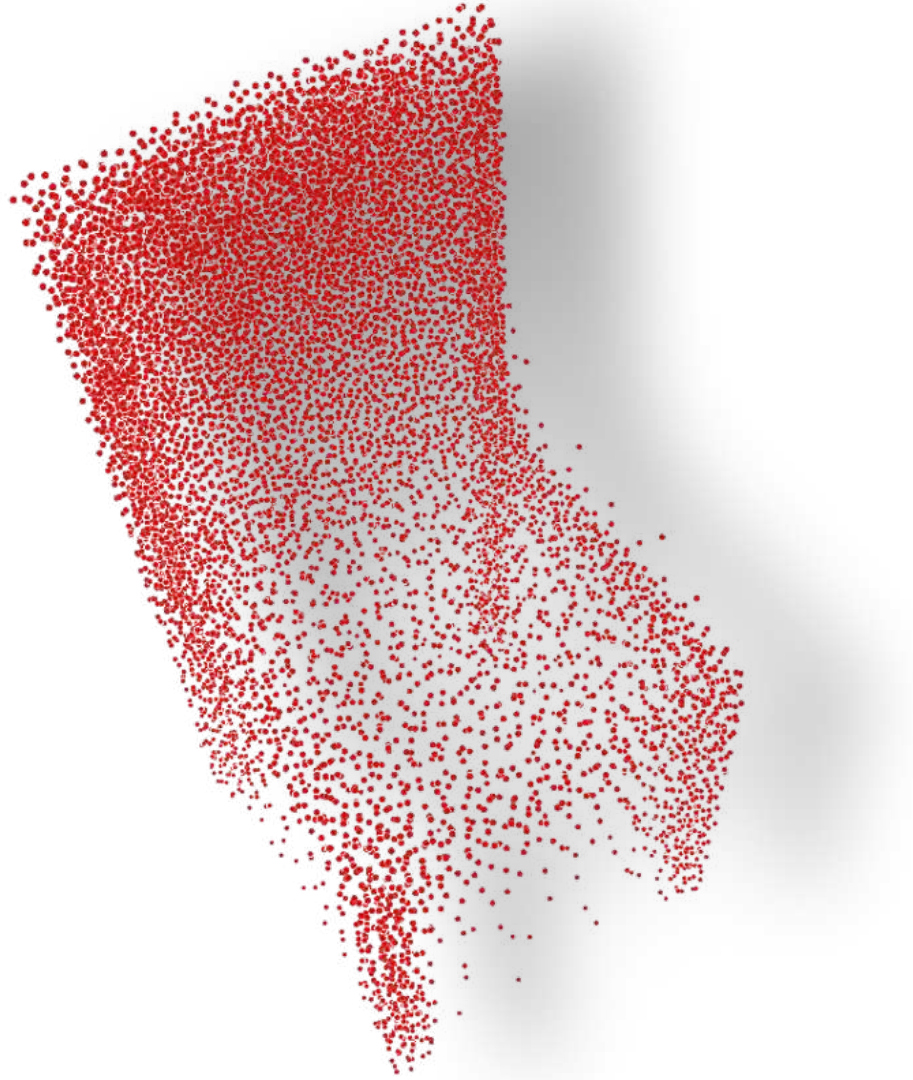



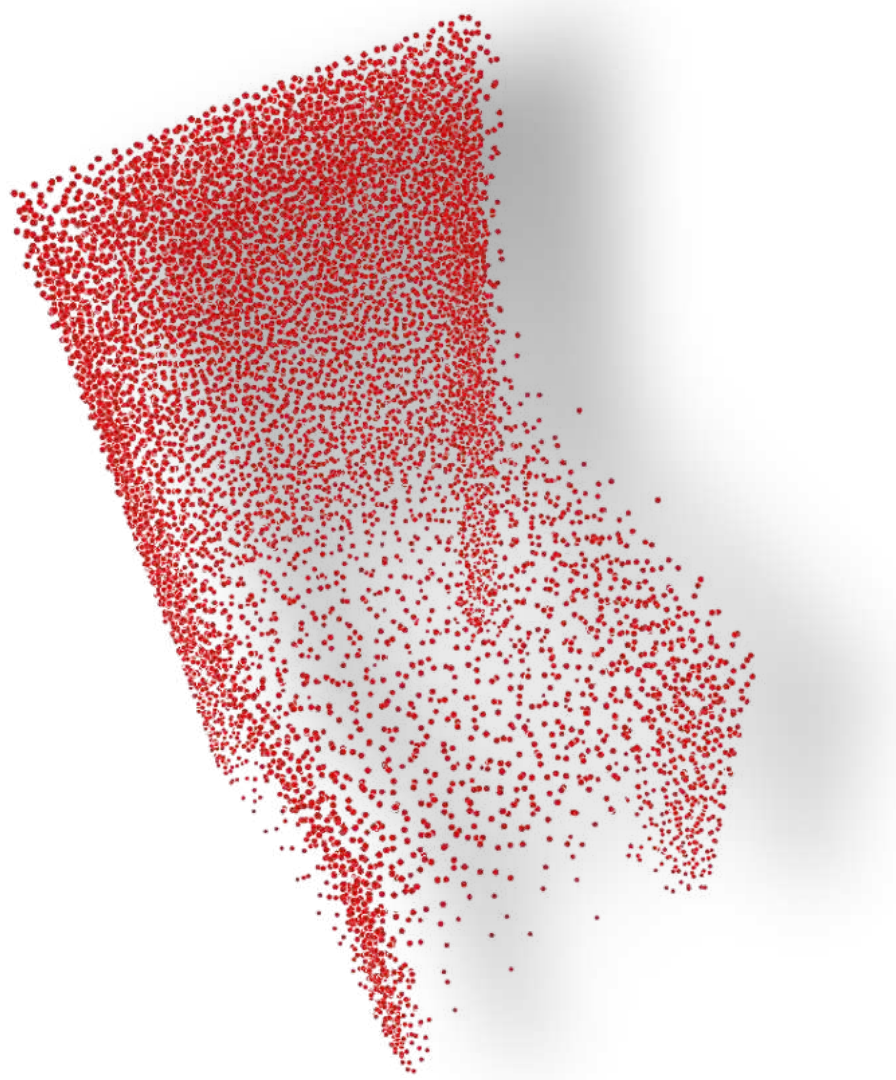

Supplement: Supplementary file 8 [file supp_view.pdf]
