# Supplementary material for: ACL-SPC: Adaptive Closed-Loop system for Self-Supervised Point Cloud Completion
Source: arXiv:2303.01979 source file (2023-03-28)
Supplement: Supplementary file 10 [file asymmetric.tex]

\begin{figure}[!h]
     \centering
     %%%%%%%%%%%%%%%%%%%%%%%%%%% Airplane1 %%%%%%%%%%%%%%%%%%%%%%%%%%
     \begin{subfigure}[b]{0.2\linewidth}
         \centering
         \includegraphics[page=1, width=\textwidth]{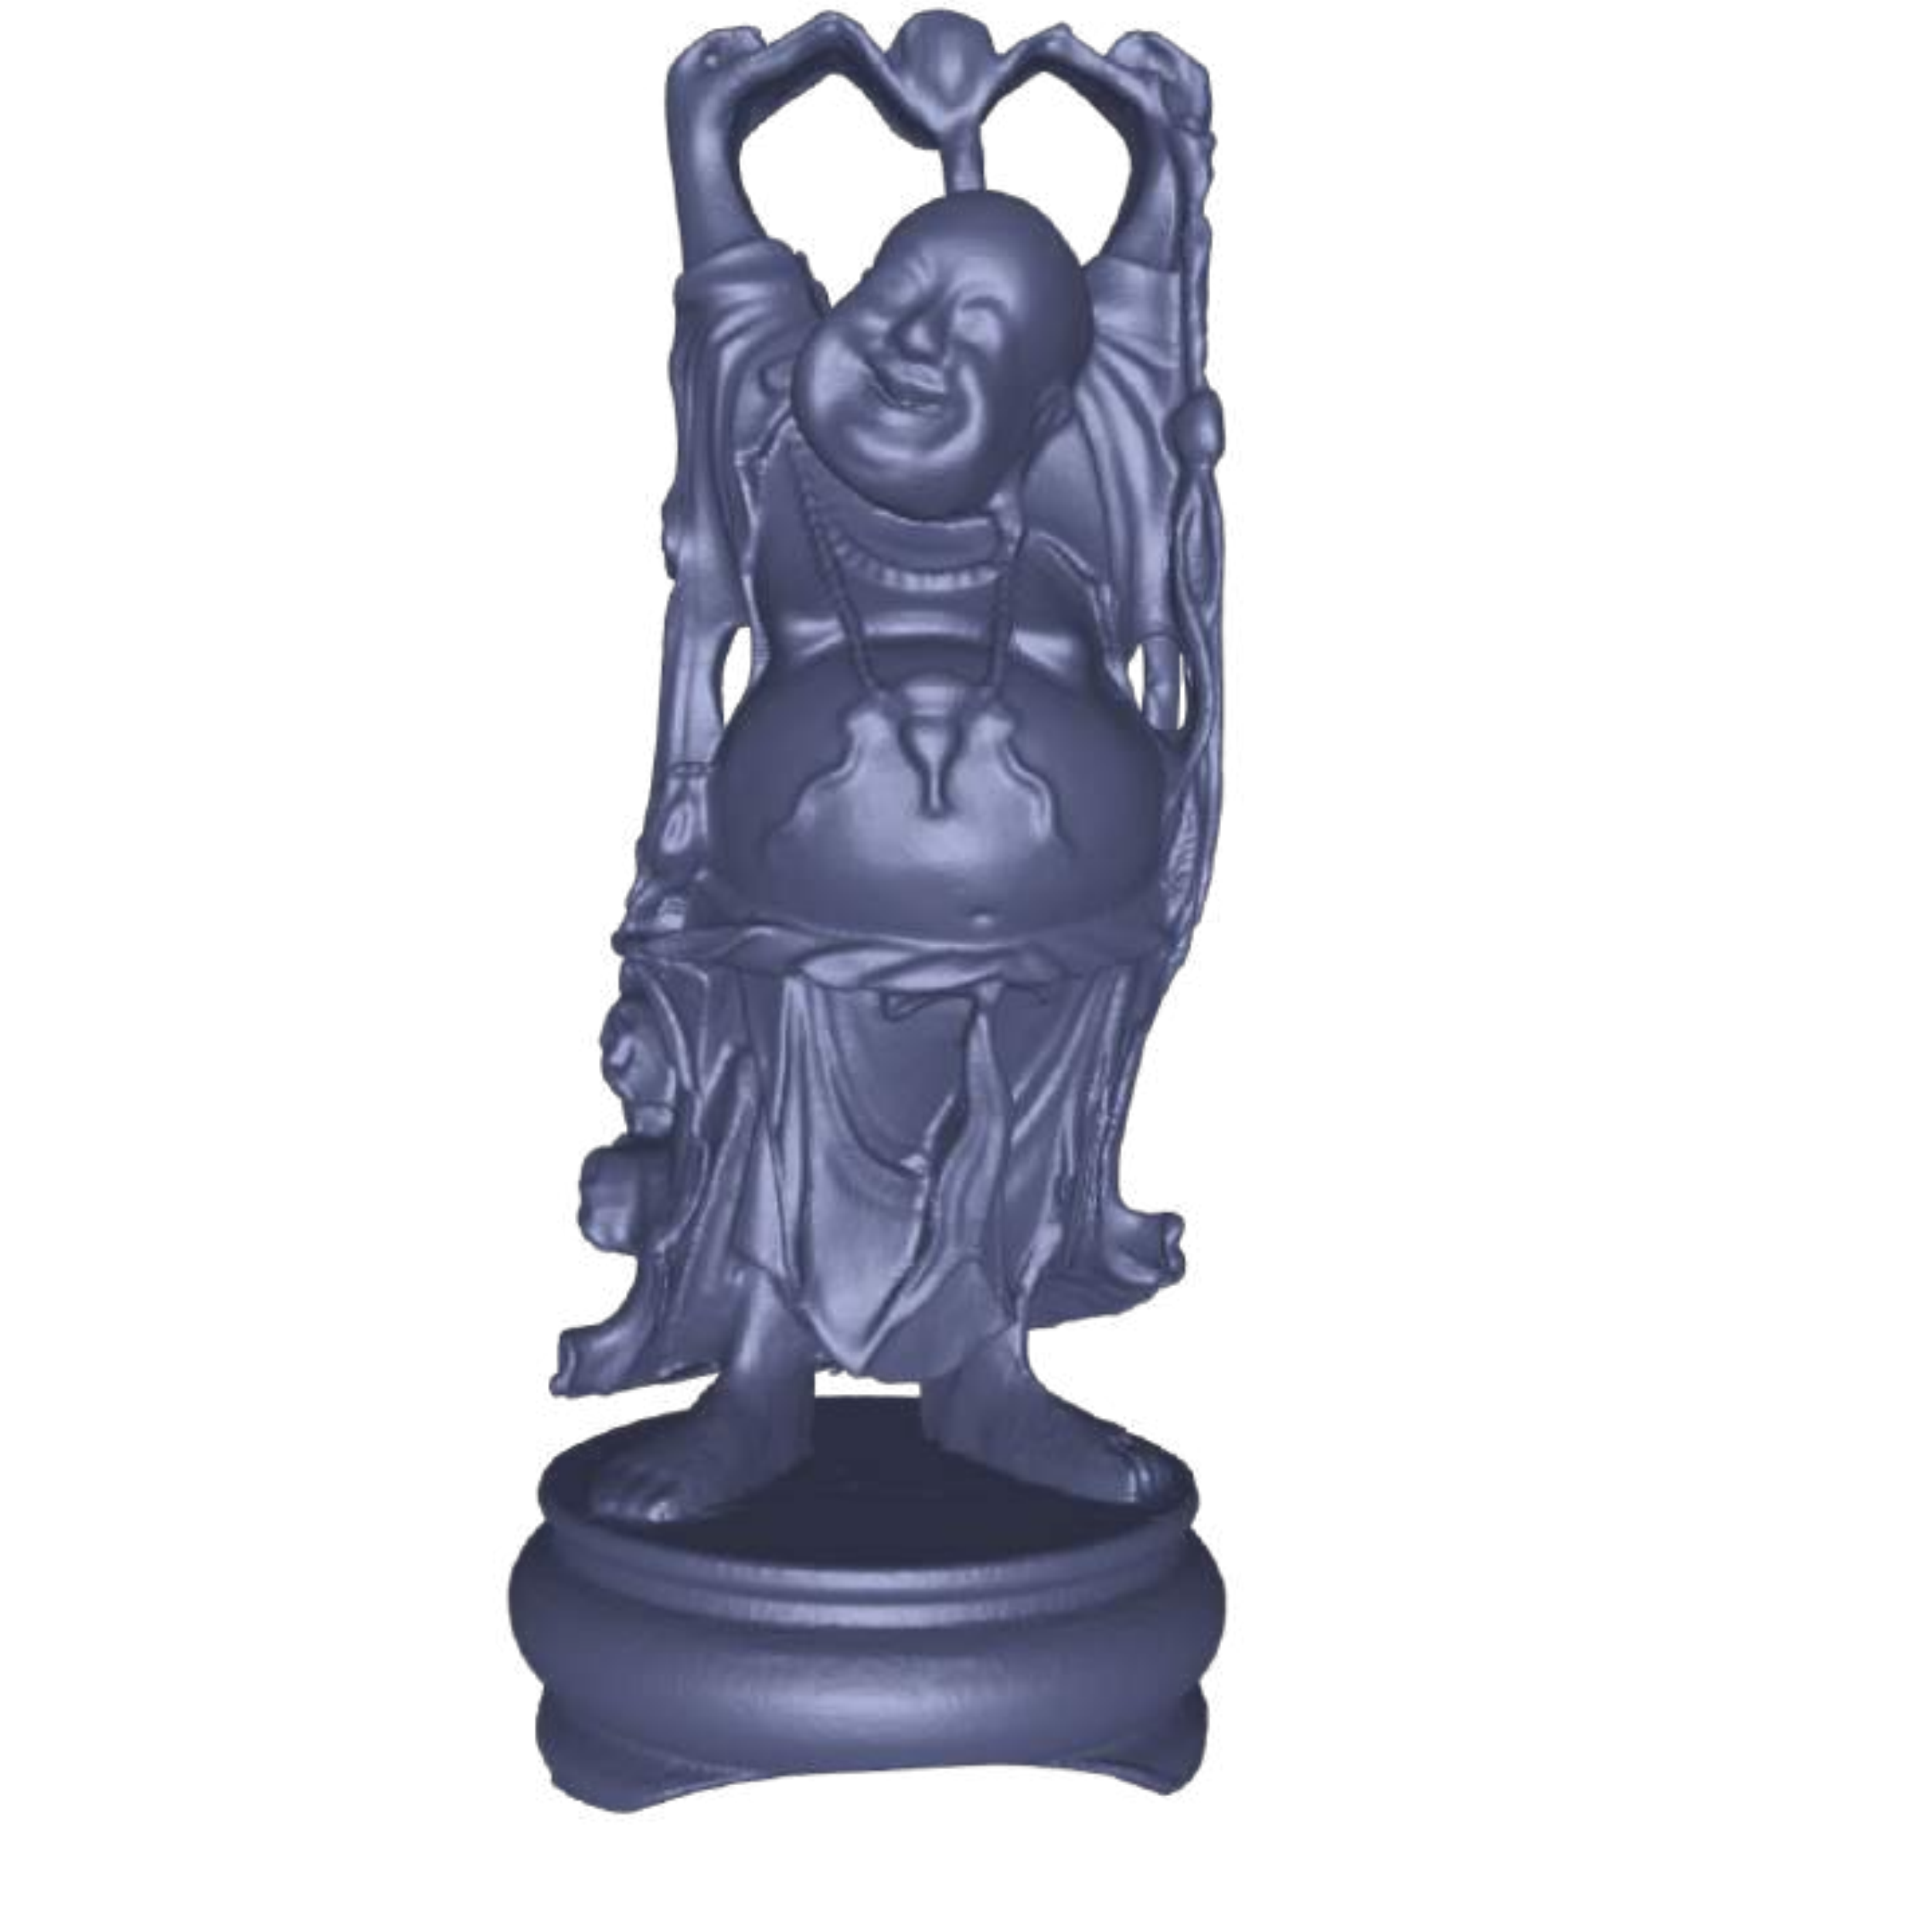}
         \caption*{Object}
     \end{subfigure}
     \hfill
     \begin{subfigure}[b]{0.2\linewidth}
         \centering
         \includegraphics[page=2, width=\textwidth]{figures/rebuttal/rebuttal_assymetric.pdf}
         \caption*{Input}
     \end{subfigure}
     \hfill
     \begin{subfigure}[b]{0.2\linewidth}
         \centering
         \includegraphics[page=3, width=\textwidth]{figures/rebuttal/rebuttal_assymetric.pdf}
         \caption*{Output}
     \end{subfigure}
     \hfill
     \begin{subfigure}[b]{0.2\linewidth}
         \centering
         \includegraphics[page=4,width=\textwidth]{figures/rebuttal/rebuttal_assymetric.pdf}
         \caption*{GT}
     \end{subfigure}
     \vspace{2mm}
     \\
    %%%%%%%%%%%%%%%%%%%%%%%%%%% Cabinet %%%%%%%%%%%%%%%%%%%%%%%%%%
    %\hspace{4mm}
     \begin{subfigure}[b]{0.2\linewidth}
         \centering
         \includegraphics[page=5, width=\textwidth]{figures/rebuttal/rebuttal_assymetric.pdf}
         \caption*{Object}
     \end{subfigure}
     \hfill
     \begin{subfigure}[b]{0.2\linewidth}
         \centering
         \includegraphics[page=6, width=\textwidth]{figures/rebuttal/rebuttal_assymetric.pdf}
         \caption*{Input}
     \end{subfigure}
     \hfill   
     \begin{subfigure}[b]{0.2\linewidth}
         \centering
         \includegraphics[page=7, width=\textwidth]{figures/rebuttal/rebuttal_assymetric.pdf}
         \caption*{Output}
     \end{subfigure}
     \hfill
     \begin{subfigure}[b]{0.2\linewidth}
         \centering
         \includegraphics[page=8, width=\textwidth]{figures/rebuttal/rebuttal_assymetric.pdf}
         \caption*{GT}
     \end{subfigure}
    \caption{
    \textbf{Qualitative results on Asymmetric Data.} 
    }        
\label{fig:asymmetric}    
\end{figure}
