# Supplementary material for: ACL-SPC: Adaptive Closed-Loop system for Self-Supervised Point Cloud Completion
Source: arXiv:2303.01979 source file (2023-03-28)
Supplement: Supplementary file 11 [file failure.tex]

\begin{figure*}[t]
     \centering
     %%%%%%%%%%%%%%%%%%%%%%%%%%% Airplane1 %%%%%%%%%%%%%%%%%%%%%%%%%%
     \begin{subfigure}[b]{0.13\textwidth}
         \centering
         \includegraphics[page=1,width=\textwidth]{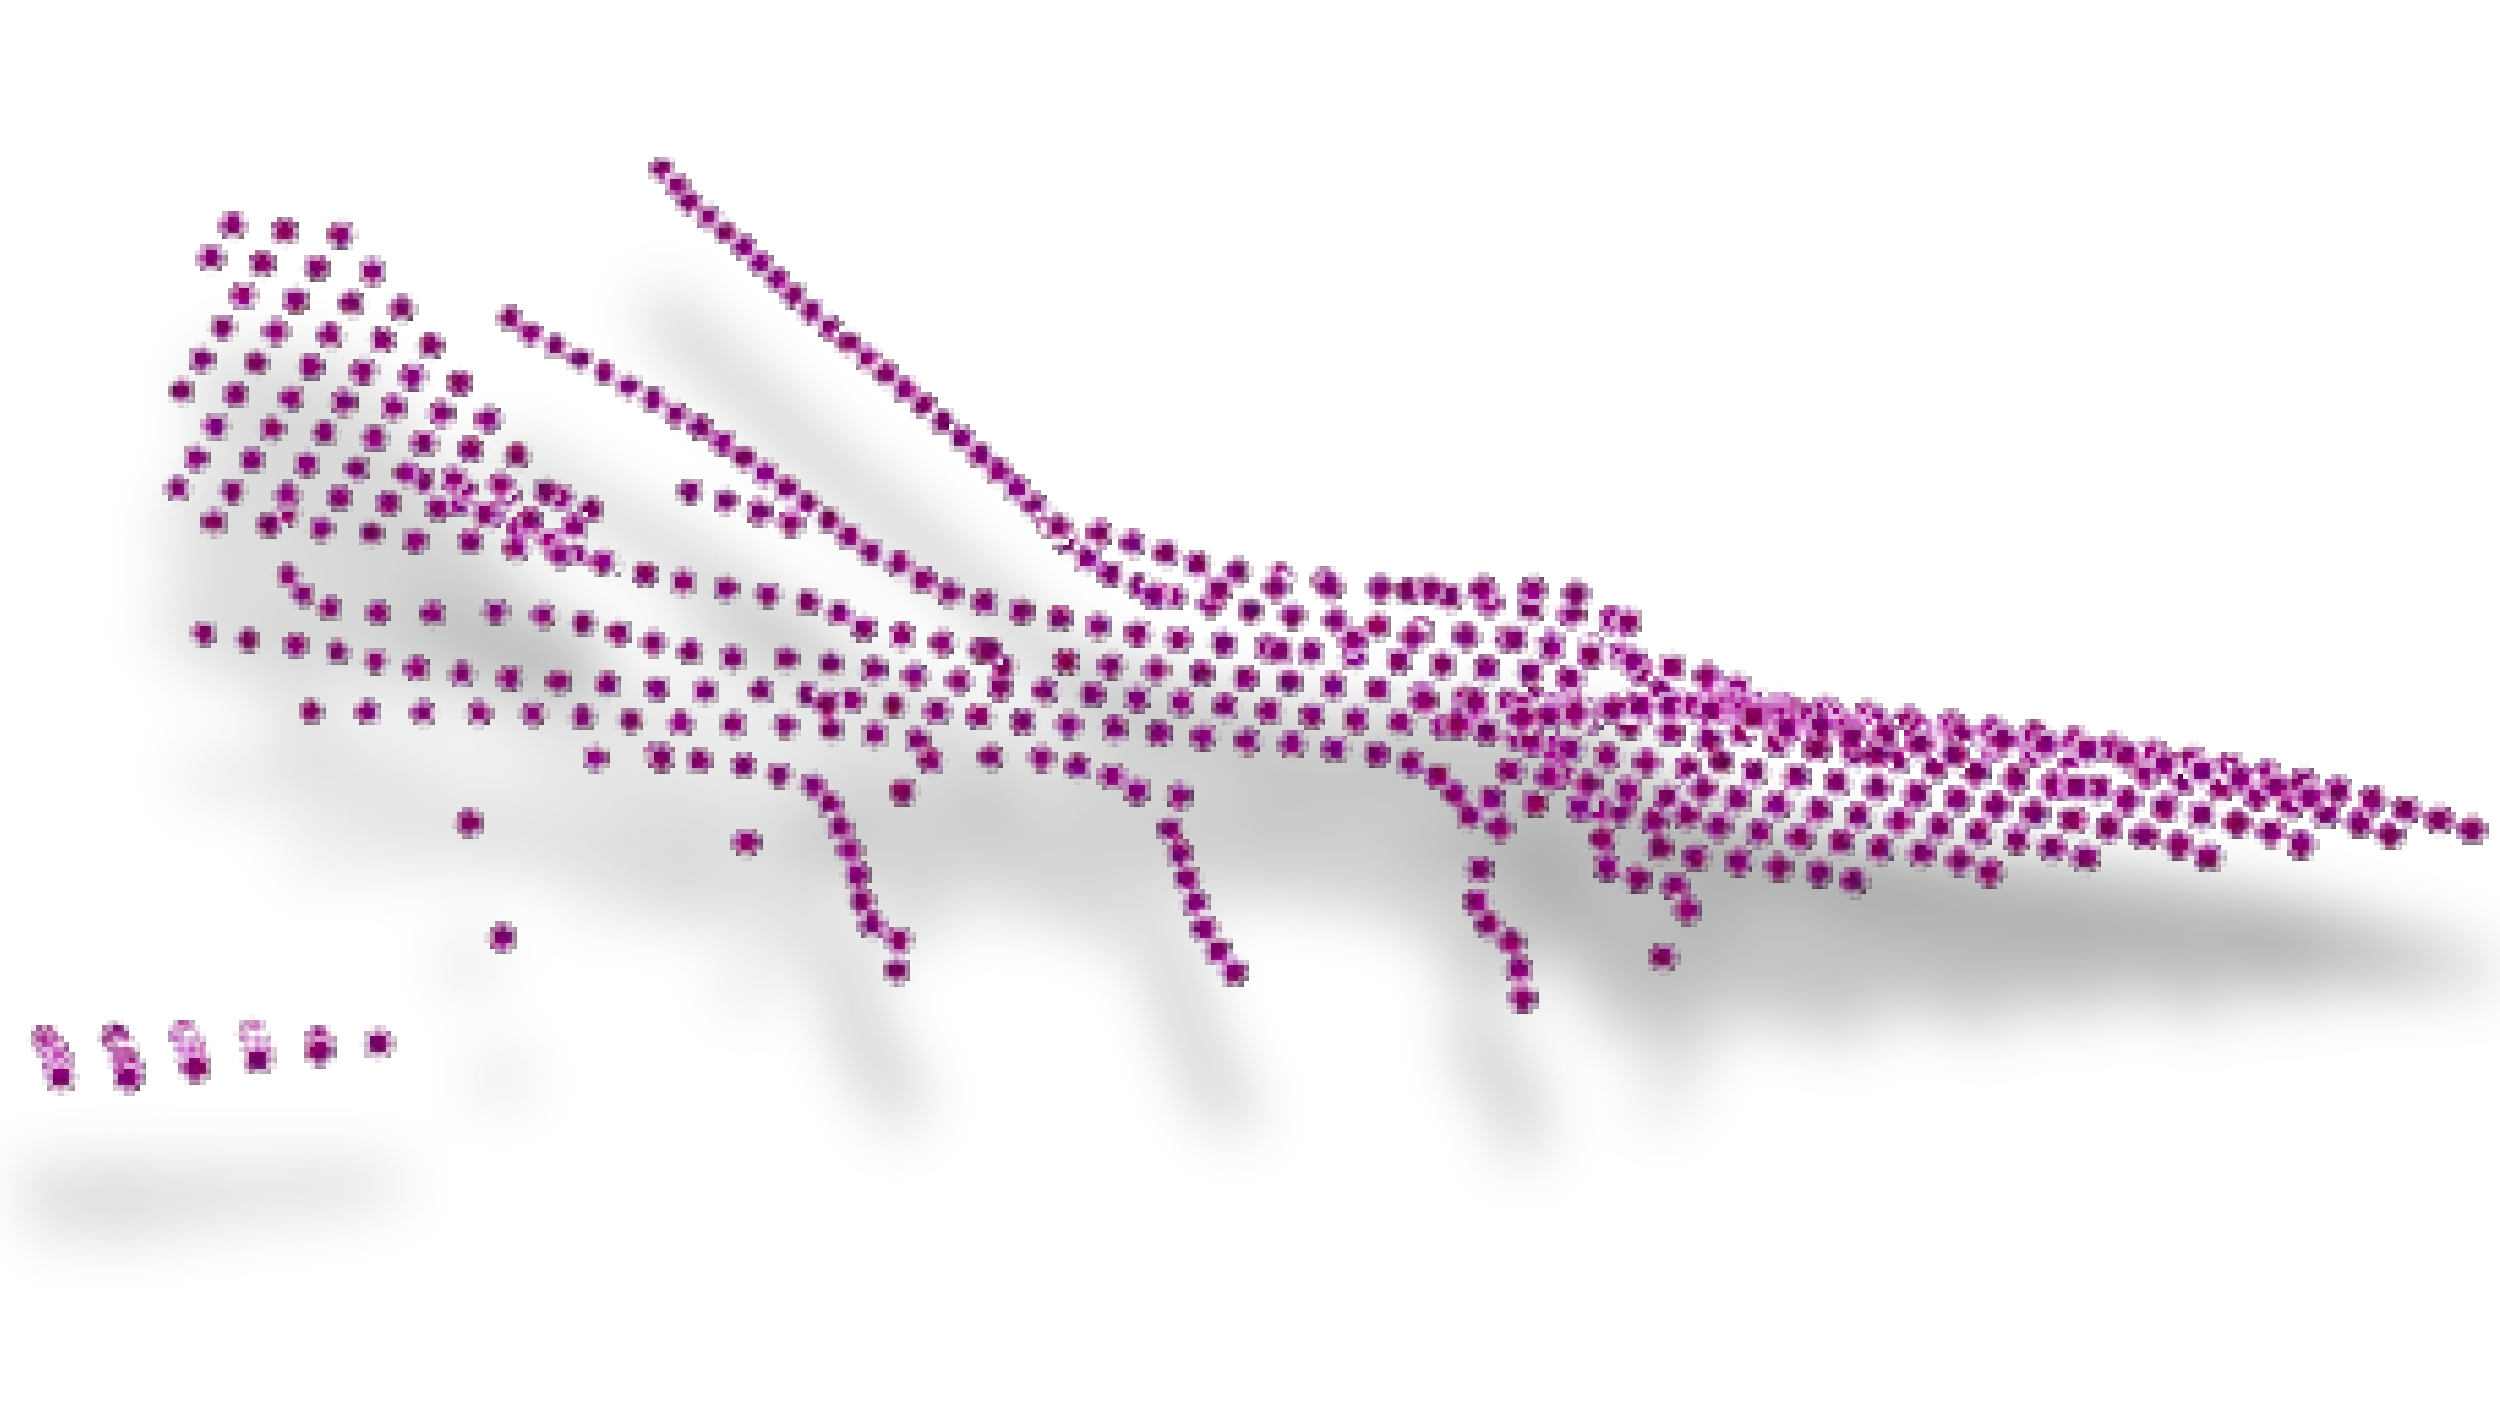}
     \end{subfigure}
     \hfill
     \begin{subfigure}[b]{0.13\textwidth}
         \centering
         \includegraphics[page=2,width=\textwidth]{figures/vis_failure.pdf}
     \end{subfigure}
     \hfill
     \begin{subfigure}[b]{0.13\textwidth}
         \centering
         \includegraphics[page=3,width=\textwidth]{figures/vis_failure.pdf}
     \end{subfigure}
     \hfill
     \hfill
     \begin{subfigure}[b]{0.13\textwidth}
         \centering
         \includegraphics[page=4,width=\textwidth]{figures/vis_failure.pdf}
     \end{subfigure}
     \hfill
     \begin{subfigure}[b]{0.13\textwidth}
         \centering
         \includegraphics[page=5,width=\textwidth]{figures/vis_failure.pdf}
     \end{subfigure}
     \hfill
     \begin{subfigure}[b]{0.13\textwidth}
         \centering
         \includegraphics[page=6,width=\textwidth]{figures/vis_failure.pdf}
     \end{subfigure}
     \\
    %%%%%%%%%%%%%%%%%%%%%%%%%%% Chair %%%%%%%%%%%%%%%%%%%%%%%%%%
     \begin{subfigure}[b]{0.13\textwidth}
         \centering
         \includegraphics[page=7,width=\textwidth]{figures/vis_failure.pdf}
     \end{subfigure}
     \hfill
     \begin{subfigure}[b]{0.13\textwidth}
         \centering
         \includegraphics[page=8,width=\textwidth]{figures/vis_failure.pdf}
     \end{subfigure}
     \hfill   
     \begin{subfigure}[b]{0.13\textwidth}
         \centering
         \includegraphics[page=9,width=\textwidth]{figures/vis_failure.pdf}
     \end{subfigure}
     \hfill
     \hfill
     \begin{subfigure}[b]{0.13\textwidth}
         \centering
         \includegraphics[page=10,width=\textwidth]{figures/vis_failure.pdf}
     \end{subfigure}
     \hfill 
     \begin{subfigure}[b]{0.13\textwidth}
         \centering
         \includegraphics[page=11,width=\textwidth]{figures/vis_failure.pdf}
     \end{subfigure}
     \hfill
     \begin{subfigure}[b]{0.13\textwidth}
         \centering
         \includegraphics[page=12,width=\textwidth]{figures/vis_failure.pdf}
     \end{subfigure}
     \\
     %%%%%%%%%%%%%%%%%%%%%%%%%%% Car %%%%%%%%%%%%%%%%%%%%%%%%%%
     \begin{subfigure}[b]{0.13\textwidth}
         \centering
         \includegraphics[page=13,width=\textwidth]{figures/vis_failure.pdf}
         \caption*{Input}
     \end{subfigure}
     \hfill
     \begin{subfigure}[b]{0.13\textwidth}
         \centering
         \includegraphics[page=14,width=\textwidth]{figures/vis_failure.pdf}
         \caption*{Output}
     \end{subfigure}
     \hfill
     \begin{subfigure}[b]{0.13\textwidth}
         \centering
         \includegraphics[page=15,width=\textwidth]{figures/vis_failure.pdf}
         \caption*{GT}
     \end{subfigure}
     \hfill
     \hfill
     \begin{subfigure}[b]{0.13\textwidth}
         \centering
         \includegraphics[page=16,width=\textwidth]{figures/vis_failure.pdf}
         \caption*{Input}
     \end{subfigure}
     \hfill
     \begin{subfigure}[b]{0.13\textwidth}
         \centering
         \includegraphics[page=17,width=\textwidth]{figures/vis_failure.pdf}
         \caption*{Output}
     \end{subfigure}   
     \hfill
     \begin{subfigure}[b]{0.13\textwidth}
         \centering
         \includegraphics[page=18,width=\textwidth]{figures/vis_failure.pdf}
         \caption*{GT}
     \end{subfigure}
        \caption{
        \textbf{Visualization of failure results.} 
        }
        \label{fig:supp_failure}
\end{figure*}
